# Supplementary material for: One Map Does Not Fit All: Evaluating Saliency Map Explanation on Multi-Modal Medical Images
Source: arXiv:2107.05047 ancillary file (2021-07-11)
Supplement: Supplementary file 1 [file eval_multimodal_heatmap_icml2021w_cameraReady_appendix.pdf]

---

# One Map Does Not Fit All: Evaluating Saliency Map Explanation on Multi-Modal Medical Images

---

Weina Jin<sup>1</sup> Xiaoxiao Li<sup>2</sup> Ghassan Hamarneh<sup>1</sup>

## 1. The Evaluated Saliency Map Methods

We select 16 commonly used activation-, gradient-, and perturbation-based saliency map methods. Except several methods such as CAM, Grad-CAM, feature permutation, and kernel SHAP, the rest can be extended to the multi-modal image input space. We briefly review the evaluated saliency map methods.

### 1.1. Activation-Based Saliency Map Methods

**CAM** (Class Activation Mapping) (Zhou et al., 2016) generates a saliency map for a prediction by aggregating the internal activations of a neural network layer by weighting each neuron’s weights in that layer to the final decision layer.

**Grad-CAM** is similar to CAM but replaces weights with gradients of the target prediction with respect to the activation map. We only include Grad-CAM in our evaluation, because it does not require special model architecture as CAM does.

For activation-based methods including CAM and Grad-CAM, because the activation maps at a deeper layer could not reflect the modality-specific information which is aggregated at the first convolutional layer, the output saliency map is a single-modality image which is not modality-specific. We copy such a saliency map to all modalities to compare it with other methods.

### 1.2. Gradient-Based Saliency Map Methods

**Gradient** reflects how quickly the output changes when input changes (Simonyan et al., 2014).

**Input  $\times$  Gradient** multiplies the input to gradient signal to approximate first-order Taylor (Shrikumar et al., 2017b).

Compare with Gradient, it tends to produce sharper saliency maps. Since (Shrikumar et al., 2017b) showed layer-wise relevance propagation (LRP) is equivalence to Input  $\times$  Gradient when all activations are piece-wise linear and biases are included, we only include Input  $\times$  Gradient in the evaluation.

**SmoothGrad** smooths the noisy gradient signals by averaging the saliency maps for an input and its random neighbourhood samples (Smilkov et al., 2017).

**De-convolution** modifies the gradient computation rule at ReLU activation function. Instead of back-propagating non-negative *input* gradients as in the vanilla Gradient method, De-convolution only back-propagates non-negative *output* gradients (Zeiler & Fergus, 2014).

**Guided Backpropagation** combines Gradient and De-convolution methods by back-propagating *input* and *output* gradients that are both non-negative (Springenberg et al., 2015).

**Guided Grad-CAM** computes the element-wise product between Guided Backpropagation and the up-sampled & broadcasted Grad-CAM signal (Selvaraju et al., 2017).

**Integrated Gradient** approximates the path integral of gradients along the straight line from a neutral baseline input to the target input (Sundararajan et al., 2017).

**DeepLIFT** explains the prediction difference from a non-informative baseline (Shrikumar et al., 2017a). DeepLIFT and Integrated Gradients both address the gradient “saturation” problem, but DeepLIFT is a faster approximation of Integrated Gradient as it is a modification of the gradient backpropagation rule.

**Gradient SHAP** approximates Shapley values by computing the expectation of gradients (Lundberg & Lee, 2017).

### 1.3. Perturbation-Based Saliency Map Methods

**Occlusion** occludes part of the image with a sliding window, and averaged output differences as the feature attribution (Zeiler & Fergus, 2014; Zintgraf et al., 2017). In our implementation, the occlusion is done modality-wise to generate saliency maps that are modality specific. The oc-

---

<sup>1</sup>School of Computing Science, Simon Fraser University, Burnaby, Canada <sup>2</sup>Department of Electrical and Computer Engineering, The University of British Columbia, Vancouver, Canada. Correspondence to: Weina Jin <weina.jin@sfu.ca>.

cluded regions are replaced by values drawn from a normal distribution with the same mean and standard deviation of the given input modality. We experimented with different sliding window and stride size to balance between saliency map resolution and computational time.

**Feature Ablation** is similar to Occlusion, but occludes the individual image features rather than using a sliding window. In our implementation, we use modality-wise superpixel segmentation masks as the image features to generate modality-specific saliency maps, and replace the ablated feature with baseline value of 0s. Cite??

**Feature Permutation** replaces image feature by shuffling the feature values within a batch, and computes the prediction difference accordingly (Fisher et al., 2019).

**LIME** (local interpretable model-agnostic explanation) learns an interpretable model by perturbing and sampling the neighbour data points around the input (Ribeiro et al., 2016).

**Shapley Value Sampling** A feature’s Shapley value is the average marginal feature attribution across all possible feature combination subsets (Shapley, 1951). Shapley Value Sampling is an efficient sampling method to overcome the expensive enumeration of all possible feature combinations (Castro et al., 2009).

**Kernel SHAP** uses the LIME framework to compute Shapley values (Lundberg & Lee, 2017). Since it only receives one superpixel feature segmentation mask that are shared across modalities, the produced saliency maps are *not* modality-specific.

## 2. More Evaluation Results

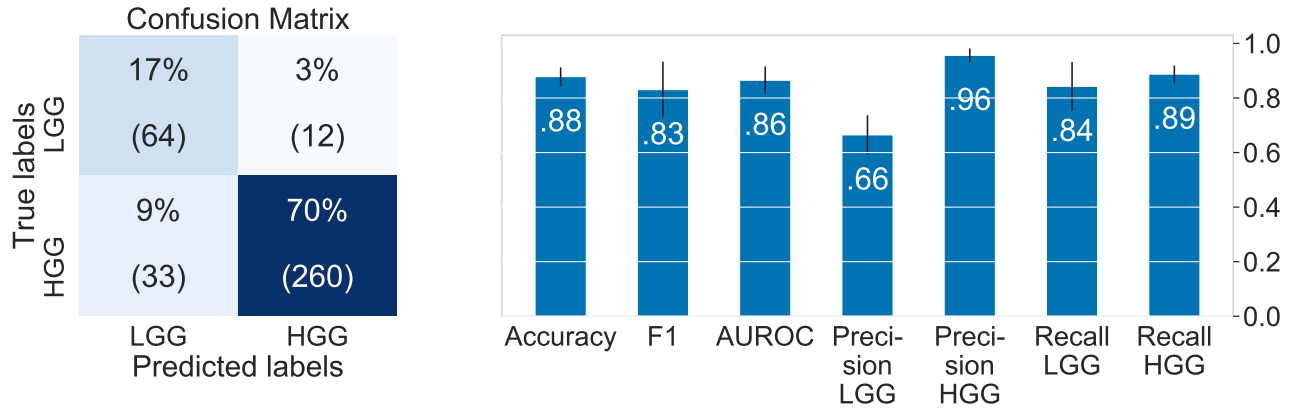

Figure 1. **Model Performance on brain tumor grade prediction.** Left: Aggregated confusion matrix of testing performance from five-fold models. Right: Mean and standard deviation of the model performance metrics.

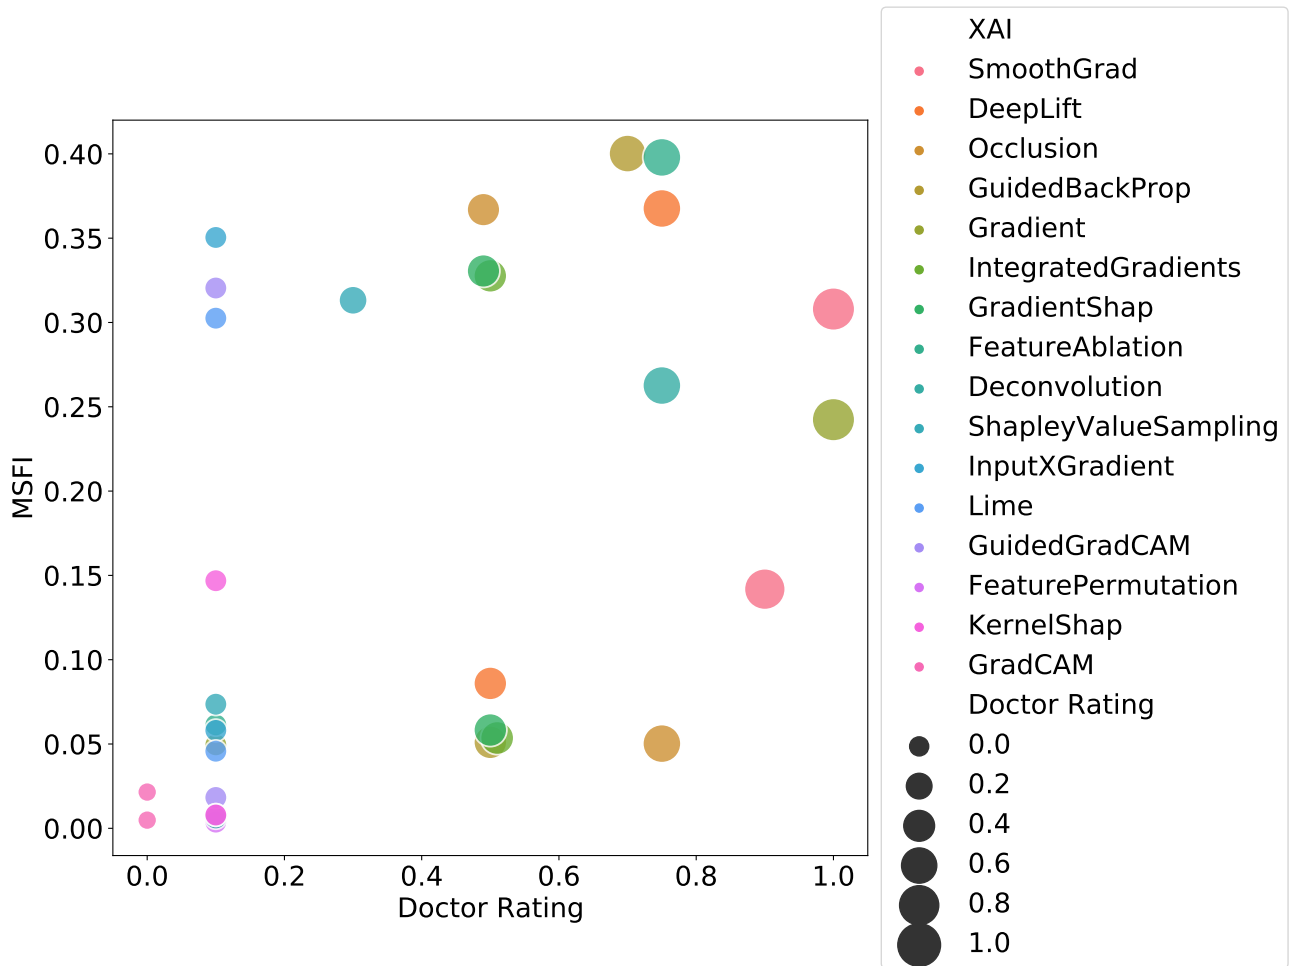

Figure 2. **Scatter plot showing the correlation of Doctor Rating and MSFI score.** Each method has two doctor ratings on two MRIs. Spearman correlation coefficient = 0.53,  $p=0.001$

## Evaluating Saliency Map Explanation on Multi-Modal Medical Images

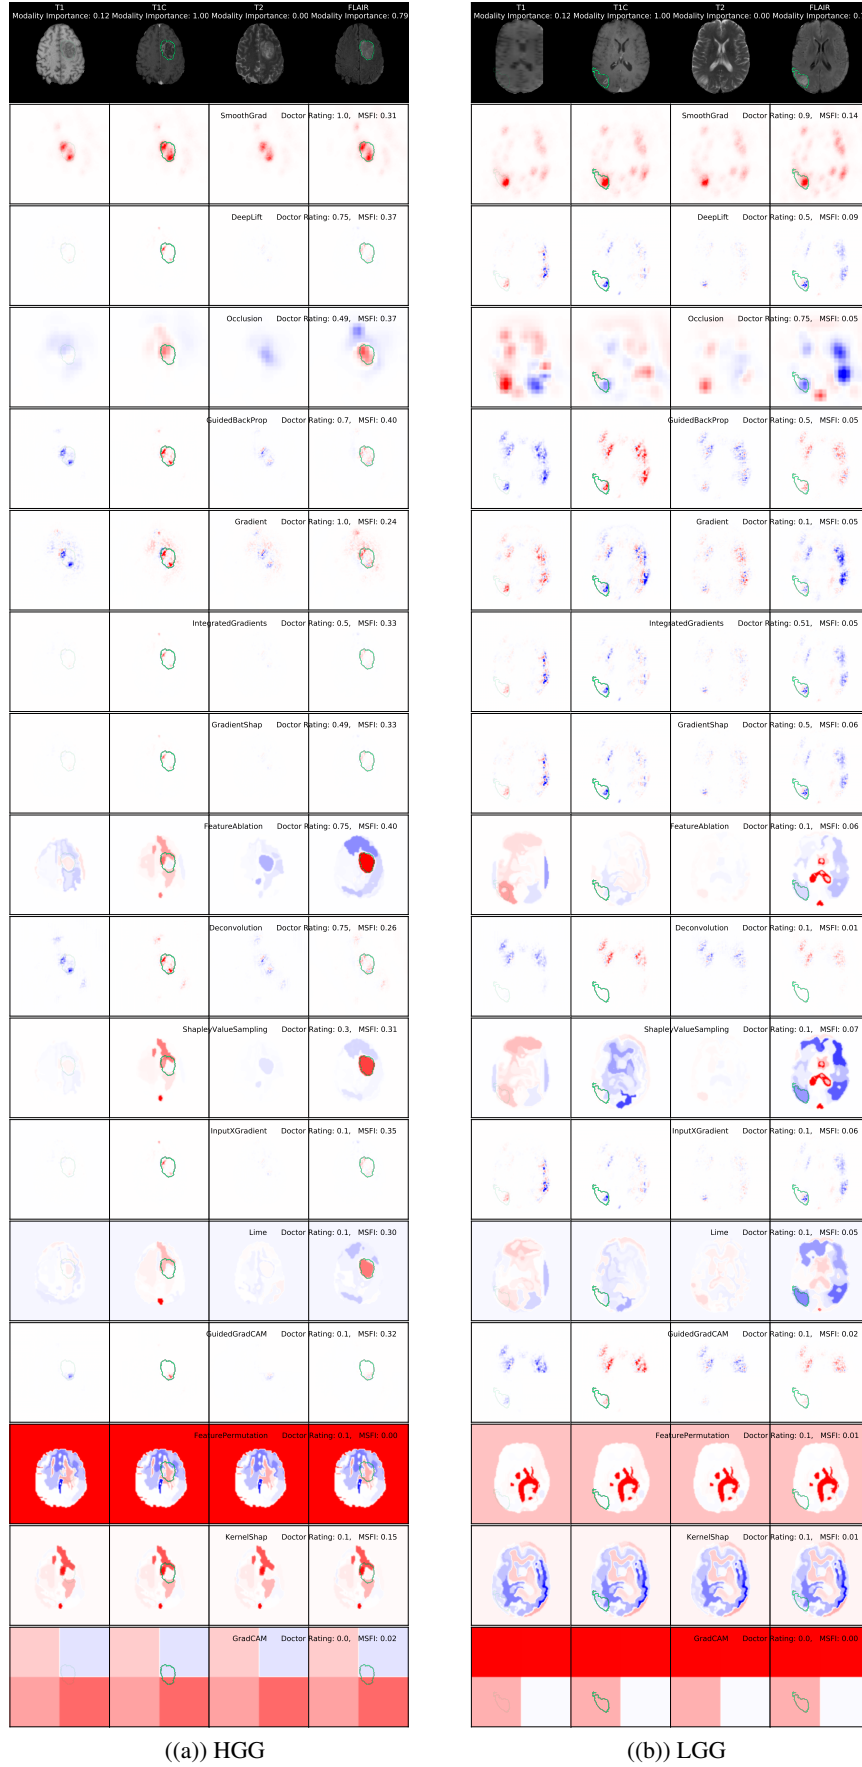

Figure 3. The evaluated 16 saliency maps on BraTS dataset/models. The ground-truth segmentation map is marked as green contour, and the Modality Importance is coded by the intensity of the mask contour. The model predicts correctly on both MRIs.



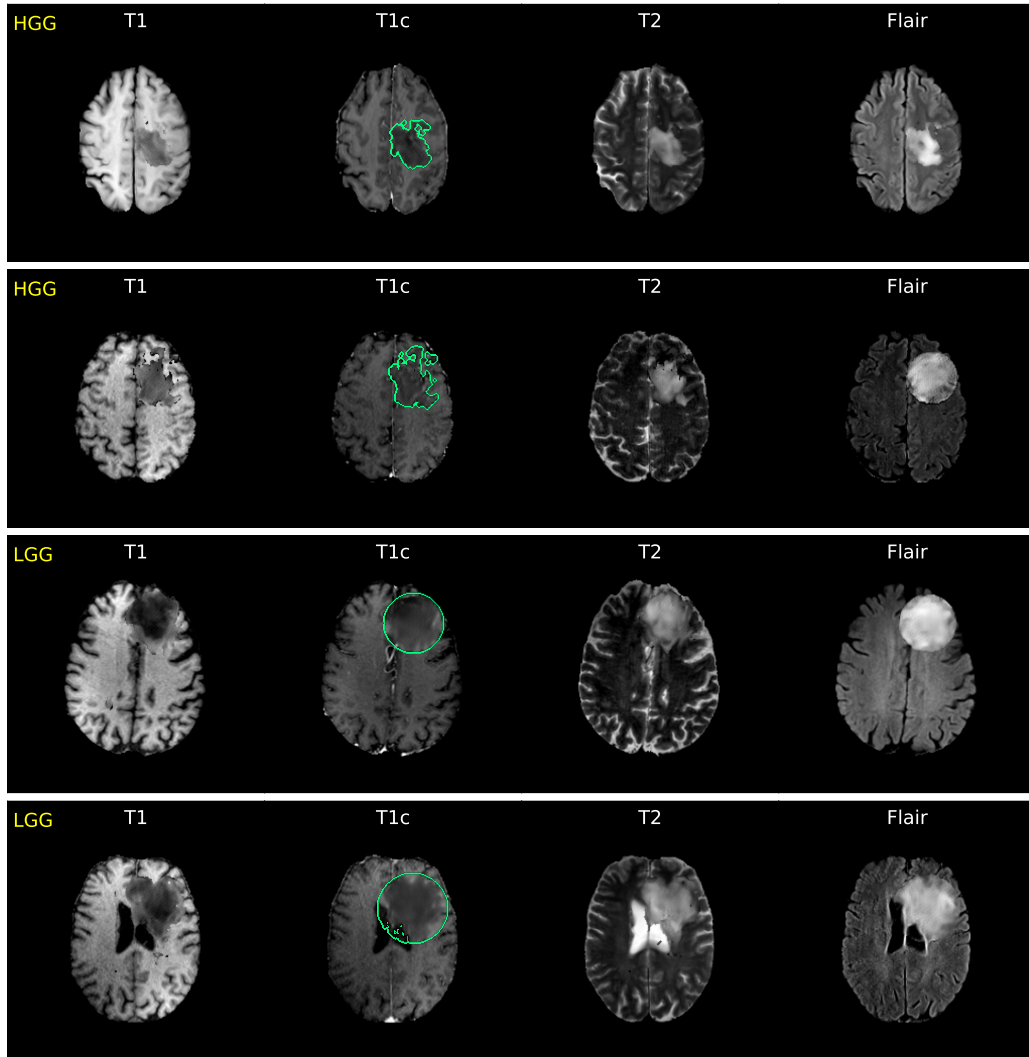

Figure 4. The synthesized multi-modal gliomas MRI. The label of HGG and LGG corresponds to tumor shapes on T1C modality, with the tumor shape outlined in segmentation mask (LGG: round; HGG: irregular). The Flair modality has 70% alignment with the label, while T1 and T2 modalities are not associated with tumor grade label.

## Evaluating Saliency Map Explanation on Multi-Modal Medical Images

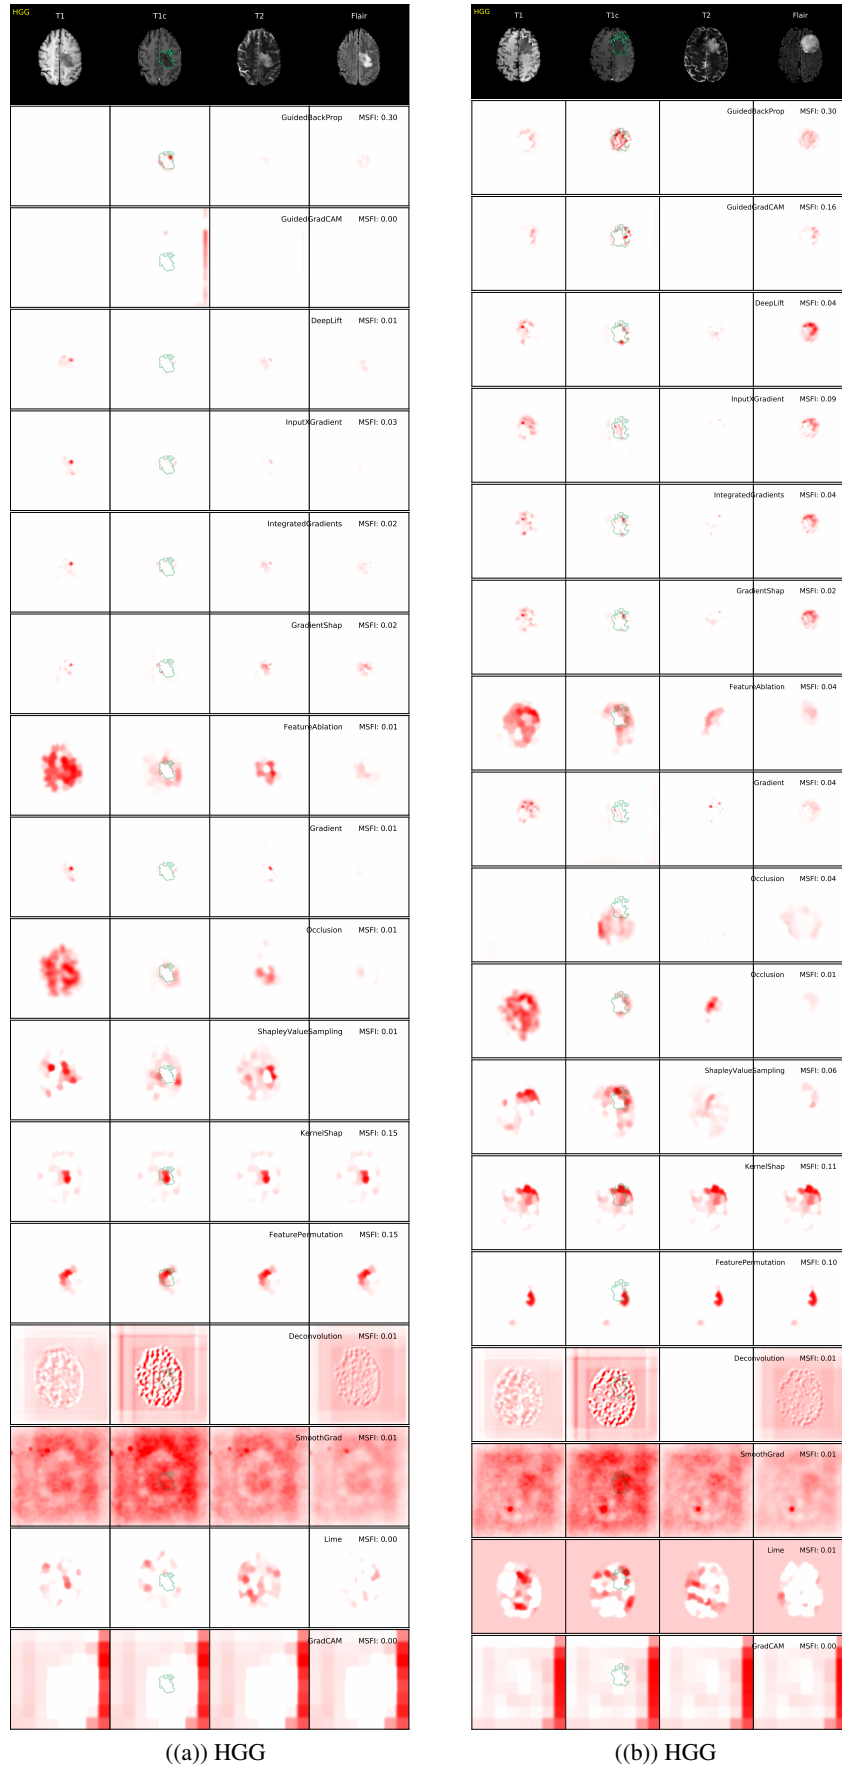

Figure 5. The evaluated 16 saliency maps on synthetic dataset/models.



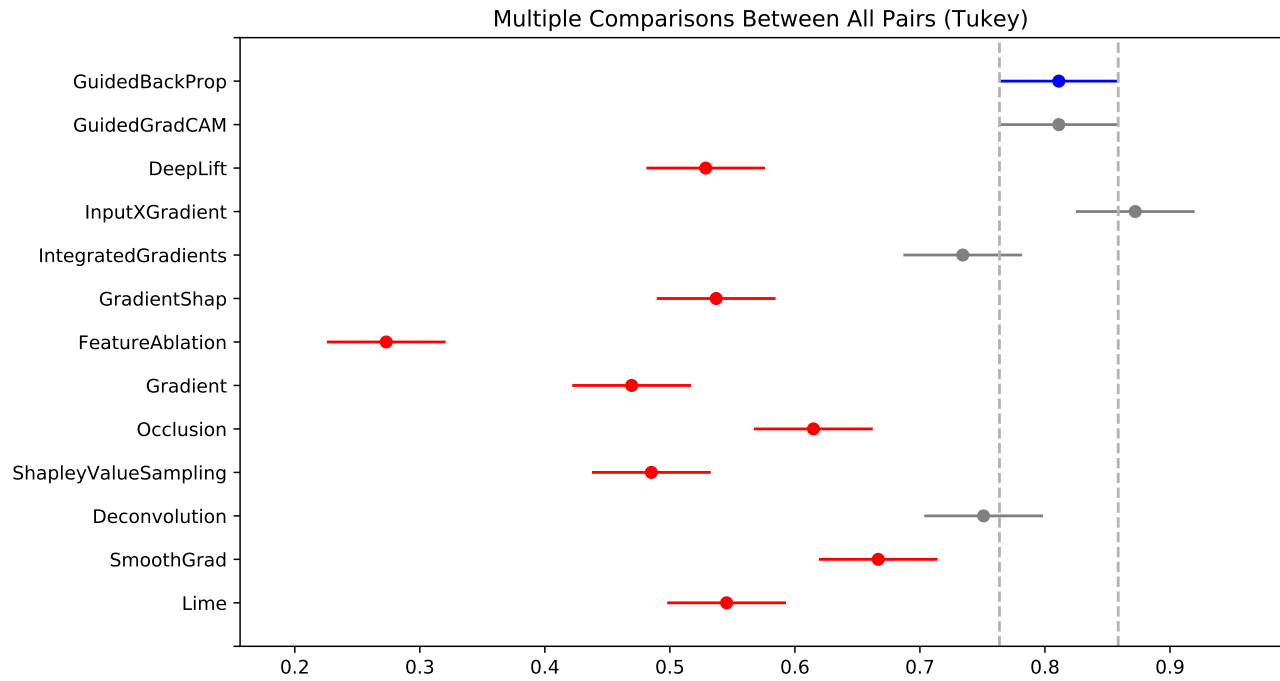

Figure 7. **Modality Importance Ranking Correlation.** The plot shows means and confidence intervals of Modality Importance Ranking Correlation. The confidence intervals are computed using Tukey's HSD test. The saliency map methods which means are significant different can be determined if their intervals do not overlap.

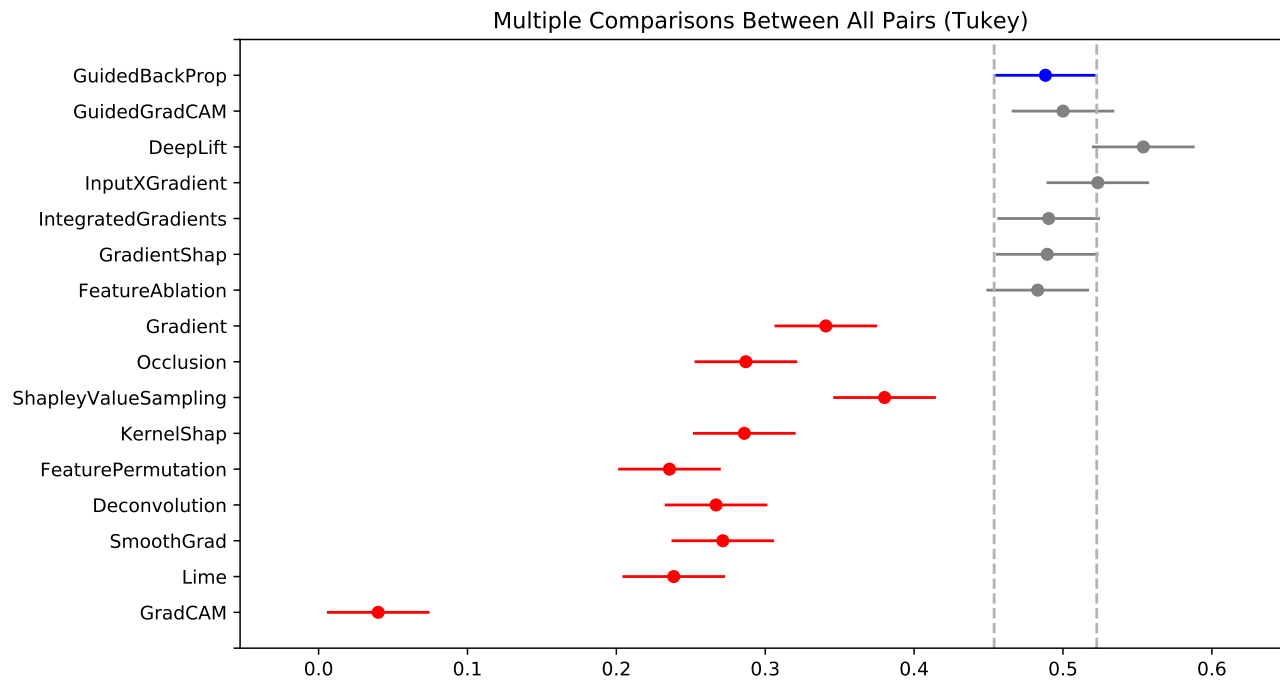

Figure 8. **MSFI: BraTS Experiment**

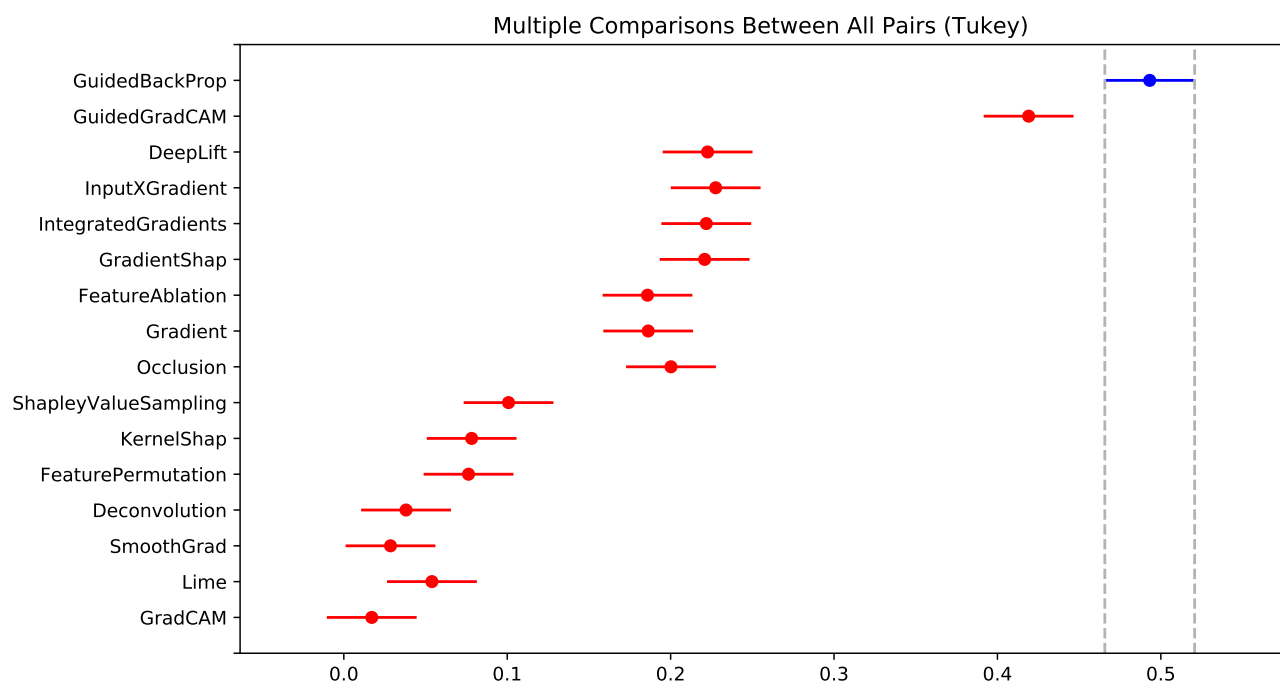

Figure 9. MSFI: Synthetic Experiment

## References

- Castro, J., Gómez, D., and Tejada, J. Polynomial calculation of the shapley value based on sampling. *Computers & Operations Research*, 36(5):1726–1730, 2009. ISSN 0305-0548. doi: <https://doi.org/10.1016/j.cor.2008.04.004>. URL <https://www.sciencedirect.com/science/article/pii/S0305054808000804>. Selected papers presented at the Tenth International Symposium on Locational Decisions (ISOLDE X).
- Fisher, A., Rudin, C., and Dominici, F. All models are wrong, but many are useful: Learning a variable’s importance by studying an entire class of prediction models simultaneously. *Journal of Machine Learning Research*, 20(177):1–81, 2019. URL <http://jmlr.org/papers/v20/18-760.html>.
- Lundberg, S. M. and Lee, S.-I. A unified approach to interpreting model predictions. In Guyon, I., Luxburg, U. V., Bengio, S., Wallach, H., Fergus, R., Vishwanathan, S., and Garnett, R. (eds.), *Advances in Neural Information Processing Systems*, volume 30. Curran Associates, Inc., 2017. URL <https://proceedings.neurips.cc/paper/2017/file/8a20a8621978632d76c43dfd28b67767-Paper.pdf>.
- Ribeiro, M. T., Singh, S., and Guestrin, C. “why should i trust you?”: Explaining the predictions of any classifier. In *Proceedings of the 22nd ACM SIGKDD International Conference on Knowledge Discovery and Data Mining*, KDD ’16, pp. 1135–1144, New York, NY, USA, 2016. Association for Computing Machinery. ISBN 9781450342322. doi: 10.1145/2939672.2939778. URL <https://doi.org/10.1145/2939672.2939778>.
- Selvaraju, R. R., Cogswell, M., Das, A., Vedantam, R., Parikh, D., and Batra, D. Grad-cam: Visual explanations from deep networks via gradient-based localization. In *2017 IEEE International Conference on Computer Vision (ICCV)*, pp. 618–626, 2017. doi: 10.1109/ICCV.2017.74.
- Shapley, L. S. *Notes on the n-Person Game – II: The Value of an n-Person Game*. RAND Corporation, Santa Monica, CA, 1951.
- Shrikumar, A., Greenside, P., and Kundaje, A. Learning important features through propagating activation differences. In *Proceedings of the 34th International Conference on Machine Learning - Volume 70*, ICML’17, pp. 3145–3153. JMLR.org, 2017a.
- Shrikumar, A., Greenside, P., Shcherbina, A., and Kundaje, A. Not just a black box: Learning important features through propagating activation differences, 2017b.
- Simonyan, K., Vedaldi, A., and Zisserman, A. Deep inside convolutional networks: Visualising image classification models and saliency maps, 2014.
- Smilkov, D., Thorat, N., Kim, B., Viégas, F., and Wattenberg, M. Smoothgrad: removing noise by adding noise, 2017.
- Springenberg, J. T., Dosovitskiy, A., Brox, T., and Riedmiller, M. Striving for simplicity: The all convolutional net, 2015.
- Sundararajan, M., Taly, A., and Yan, Q. Axiomatic attribution for deep networks. In *Proceedings of the 34th International Conference on Machine Learning - Volume 70*, ICML’17, pp. 3319–3328. JMLR.org, 2017.
- Zeiler, M. D. and Fergus, R. Visualizing and understanding convolutional networks. In Fleet, D., Pajdla, T., Schiele, B., and Tuytelaars, T. (eds.), *Computer Vision – ECCV 2014*, pp. 818–833, Cham, 2014. Springer International Publishing. ISBN 978-3-319-10590-1.
- Zhou, B., Khosla, A., Lapedriza, A., Oliva, A., and Torralba, A. Learning deep features for discriminative localization. In *2016 IEEE Conference on Computer Vision and Pattern Recognition (CVPR)*, pp. 2921–2929, 2016. doi: 10.1109/CVPR.2016.319.
- Zintgraf, L. M., Cohen, T. S., Adel, T., and Welling, M. Visualizing deep neural network decisions: Prediction difference analysis. In *5th International Conference on Learning Representations, ICLR 2017, Toulon, France, April 24-26, 2017, Conference Track Proceedings*. OpenReview.net, 2017. URL <https://openreview.net/forum?id=BJ5UeU9xx>.
