# Supplementary material for: One Map Does Not Fit All: Evaluating Saliency Map Explanation on Multi-Modal Medical Images
Source: arXiv:2107.05047 ancillary file (2021-07-11)
Supplement: Supplementary file 2 [file doctor_survey_content.pdf]

## **Welcome to the Medical AI study**

### **Welcome to our Medical AI study!**

**Study title: A usability study to assess the clinical utility of AI and explainable AI**

We have an AI system that learns to predict diagnosis, interested clinical metrics, or prognosis from brain MRI.

We are interested in its clinical utility to neurosurgeons/neuro-radiologists. Therefore, we would like to invite you to our study.

Before we proceed, please read the study consent form below, and decide if you would like to participate in the study.

Please feel free to ask any questions you have about the consent form or the study.

**\* 1. Do you agree to participate in the study?**

Taking part in this study is entirely up to you. You have the right to refuse to participate in this study.

If you decide to take part in the study, you may choose to withdraw from the study at any time without giving reasons.

If you have any concerns or complaints about your rights as a research participant and/or your experiences while participating in this study, you may contact Dr. Jeffrey Toward, Director, Office of Research Ethics, Simon Fraser University, British Columbia, Canada, at [jtoward@sfu.ca](mailto:jtoward@sfu.ca) or +1 778-782-6593.

☐ Yes, I agree to participate in the study

☐ No, I will not participate in the study

## Welcome to the Medical AI study

### Meet the medical AI system that grades gliomas on MRI

We have an AI system that learns to predict diagnosis, interested clinical metrics, or prognosis from brain MRI.

As a preliminary step of applying AI for clinical decision support, we trained the AI model on the task to classify gliomas from MRI into two types:

**low-grade gliomas (LGG)** or **high-grade (HGG) gliomas**.

**\* 2. What is your initial trust level in this AI model?**

-5, Totally distrust the AI      0, Neutral, neither distrust nor trust      5, Totally trust the AI

\* 3. How likely will you incorporate this AI's suggestions into your clinical practice?

Consider the likelihood that you are willing to let this AI assist you (in ways such as: it may reinforce your confidence about a decision; or it may alert you to potential mistakes, etc.), and consider its suggestions to your patient's management plan.

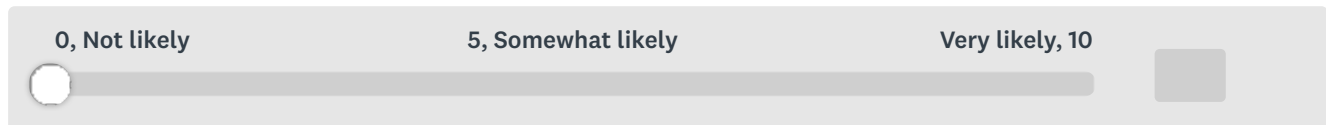

The prediction accuracy of the AI model is: **90%**.

I.e.: given a new patient MRI, its prediction has a **90% likelihood of being correct**.

This performance is tested on a test set, which is a dataset of new patients that have never been used to train the AI model).

Its fine-grained performance metrics are shown below:

\* 4. After viewing the AI's performance on previous test data, what is your trust level in this AI?

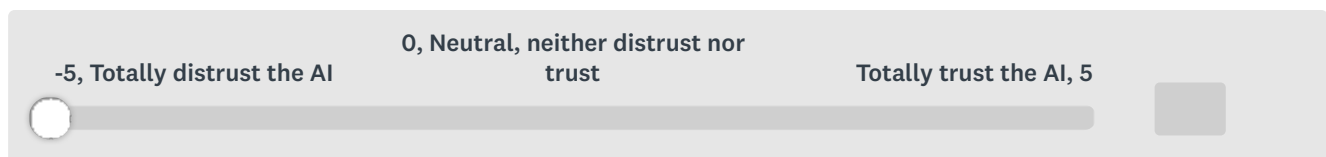

\* 5. After viewing the AI's performance on previous test data, how likely will you incorporate this AI's suggestions into your clinical practice?

Consider the likelihood that you are willing to let this AI assist you (in ways such as: it may reinforce your confidence about a decision; or it may alert you to potential mistakes, etc.), and consider its suggestions to your patient's management plan.

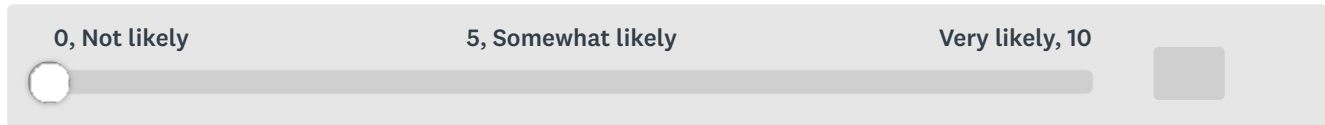

A horizontal slider scale is displayed within a light gray rectangular container. The scale is marked with three labels: "0, Not likely" at the left end, "5, Somewhat likely" in the middle, and "Very likely, 10" at the right end. A white circular slider knob is positioned at the far left, corresponding to the value 0. A thin gray line extends from the knob towards the right, ending in a small gray square at the 10 mark.

\* 6. Now you have a new patient MRI, and this AI is available for you to use, to assist your judgment on tumor grade.

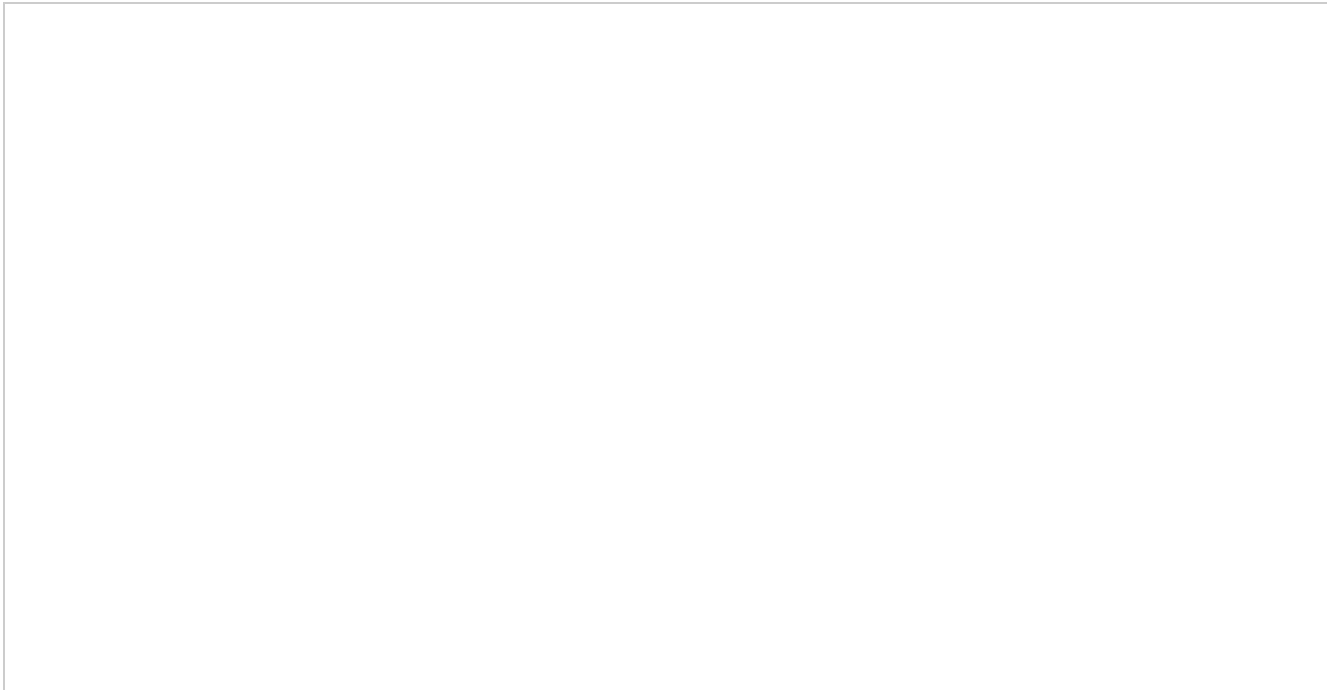

First, would you mind providing your judgment on this patient's MRI?

- ☐ Low-grade gliomas (LGG)
- ☐ High-grade gliomas (HGG)
- ☐ Other, please specify.

7. How confident are you in making this judgment?

0, Not confident at all

5, Somewhat confident

Completely confident, 10

Welcome to the Medical AI  
study

MRI for Patient 1

\* 8. AI predicts this is **high-grade gliomas**. What are your thoughts about AI's prediction?

- ☐ I am **OK with the prediction from AI**. I would like to check more detailed information from AI, to see how it reaches this prediction .
- ☐ I am **not comfortable with the prediction from AI** . I would like to check more detailed information from AI, to see how it reaches this prediction .
- ☐ I am **OK with the prediction from AI**. I have other priorities, and **won't check more detailed information from AI**.
- ☐ I am **not comfortable with the prediction from AI** . But I have other priorities, and **won't check more detailed information from AI**.

9. After viewing this AI's prediction on the new patient, what is your trust level in this AI?

-5, Totally distrust the AI

0, Neutral, neither distrust nor trust

Totally trust the AI, 5

10. After viewing this AI's prediction on the new patient, how likely will you incorporate this AI's suggestions into your clinical practice?

Consider the likelihood that you are willing to let this AI assist you (in ways such as: it may reinforce your confidence about a decision; or it may alert you to potential mistakes, etc.), and consider its suggestions to your patient's management plan.

0, Not likely                      5, Somewhat likely                      Very likely, 10

## Welcome to the Medical AI study

### Color Map Explanation for Patient 1

The AI could explain its decisions using color maps. The color maps indicate important brain regions for the AI's prediction.

We have different methods to generate the color map explanation. But we don't know which ones would fulfill your clinical requirements, and would like to ask you to help select the ones that work best for you clinically.

Next, we would like to invite you to review the following 16 color maps. They all try to explain the same AI model that predicts **high-grade gliomas**, for the same patient MRI.

Row 1: the original MRI you just read

Row 2: the color map only

Row 3: the color map overlaid on the MRI

**11.**

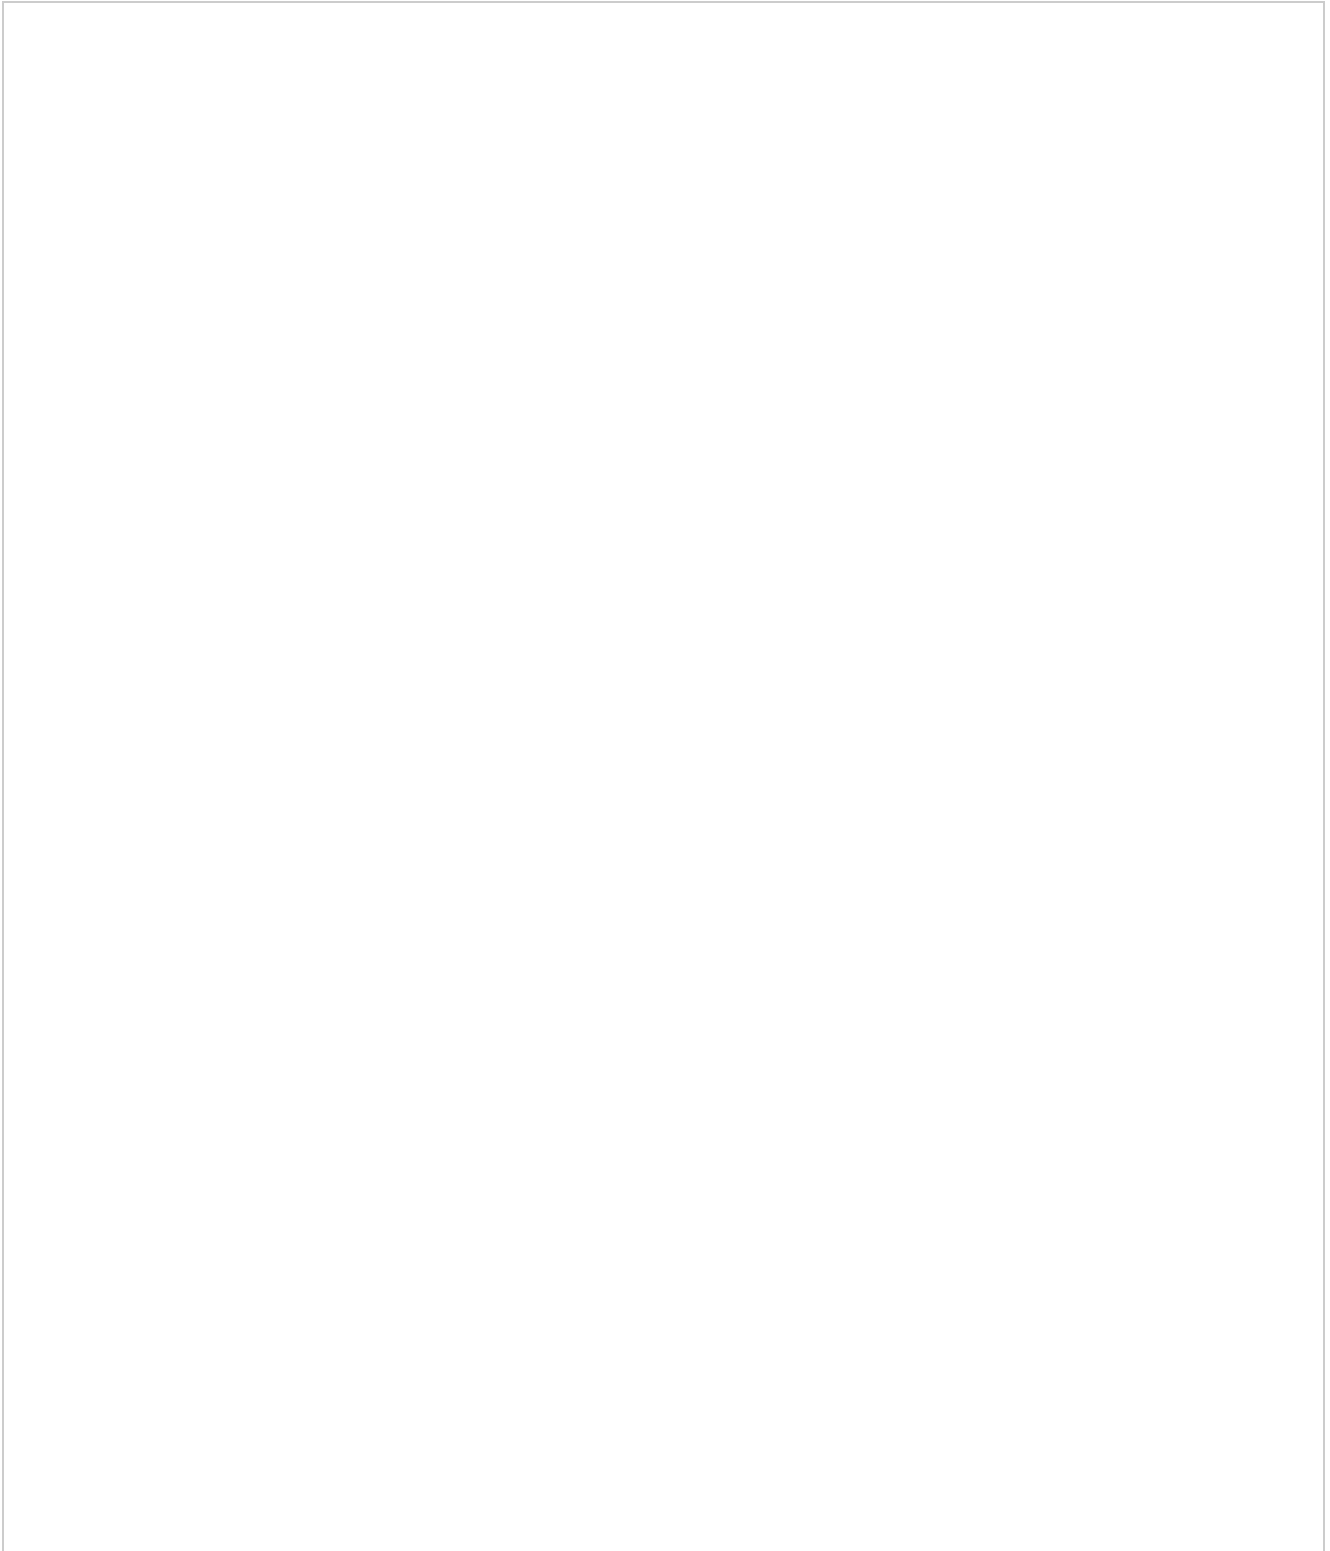

**Please provide any of your comments on this color map.**

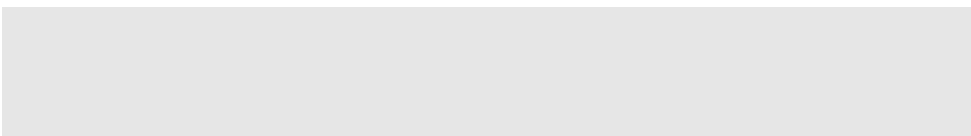



**12. How many percentages do the highlighted area match with your clinical judgment on the important features to classify LGG/HGG?**

0%, Not matches at all                      50%                      Completely matches with mine, 100%

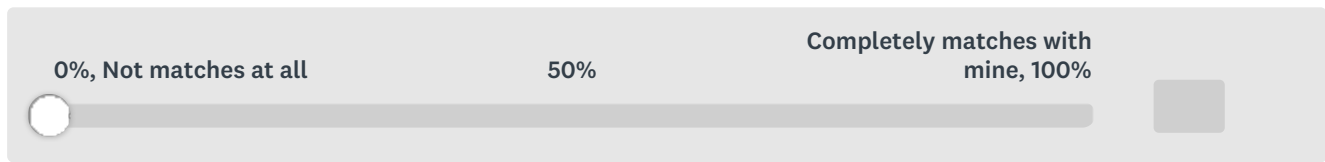A horizontal slider bar with a white circular knob at the 0% position. The bar is light gray and spans the width of the question area.☐

**13. How helpful is this color map in clinical settings?**

0, Not helpful at all                      5, Somewhat helpful                      Extremely helpful, 10

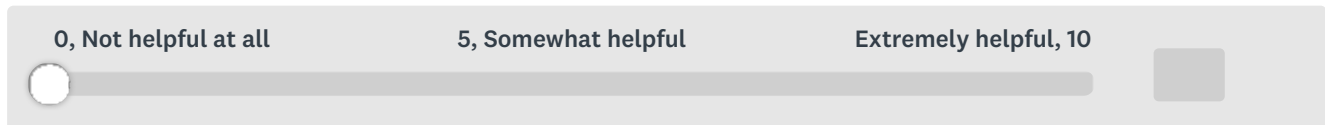A horizontal slider bar with a white circular knob at the 0 position. The bar is light gray and spans the width of the question area.☐

**14. Did you notice the color map differences on different MRI modalities? How helpful is this feature in clinical settings?**

0, Not helpful at all                      5, Somewhat helpful                      Extremely helpful, 10

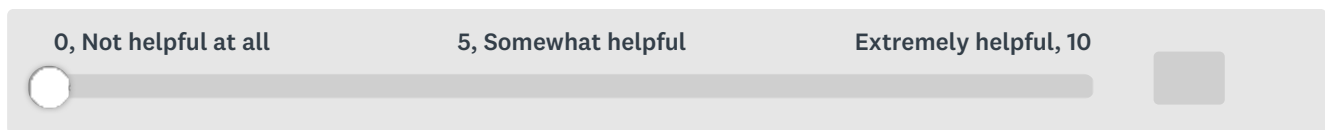A horizontal slider bar with a white circular knob at the 0 position. The bar is light gray and spans the width of the question area.☐

15.

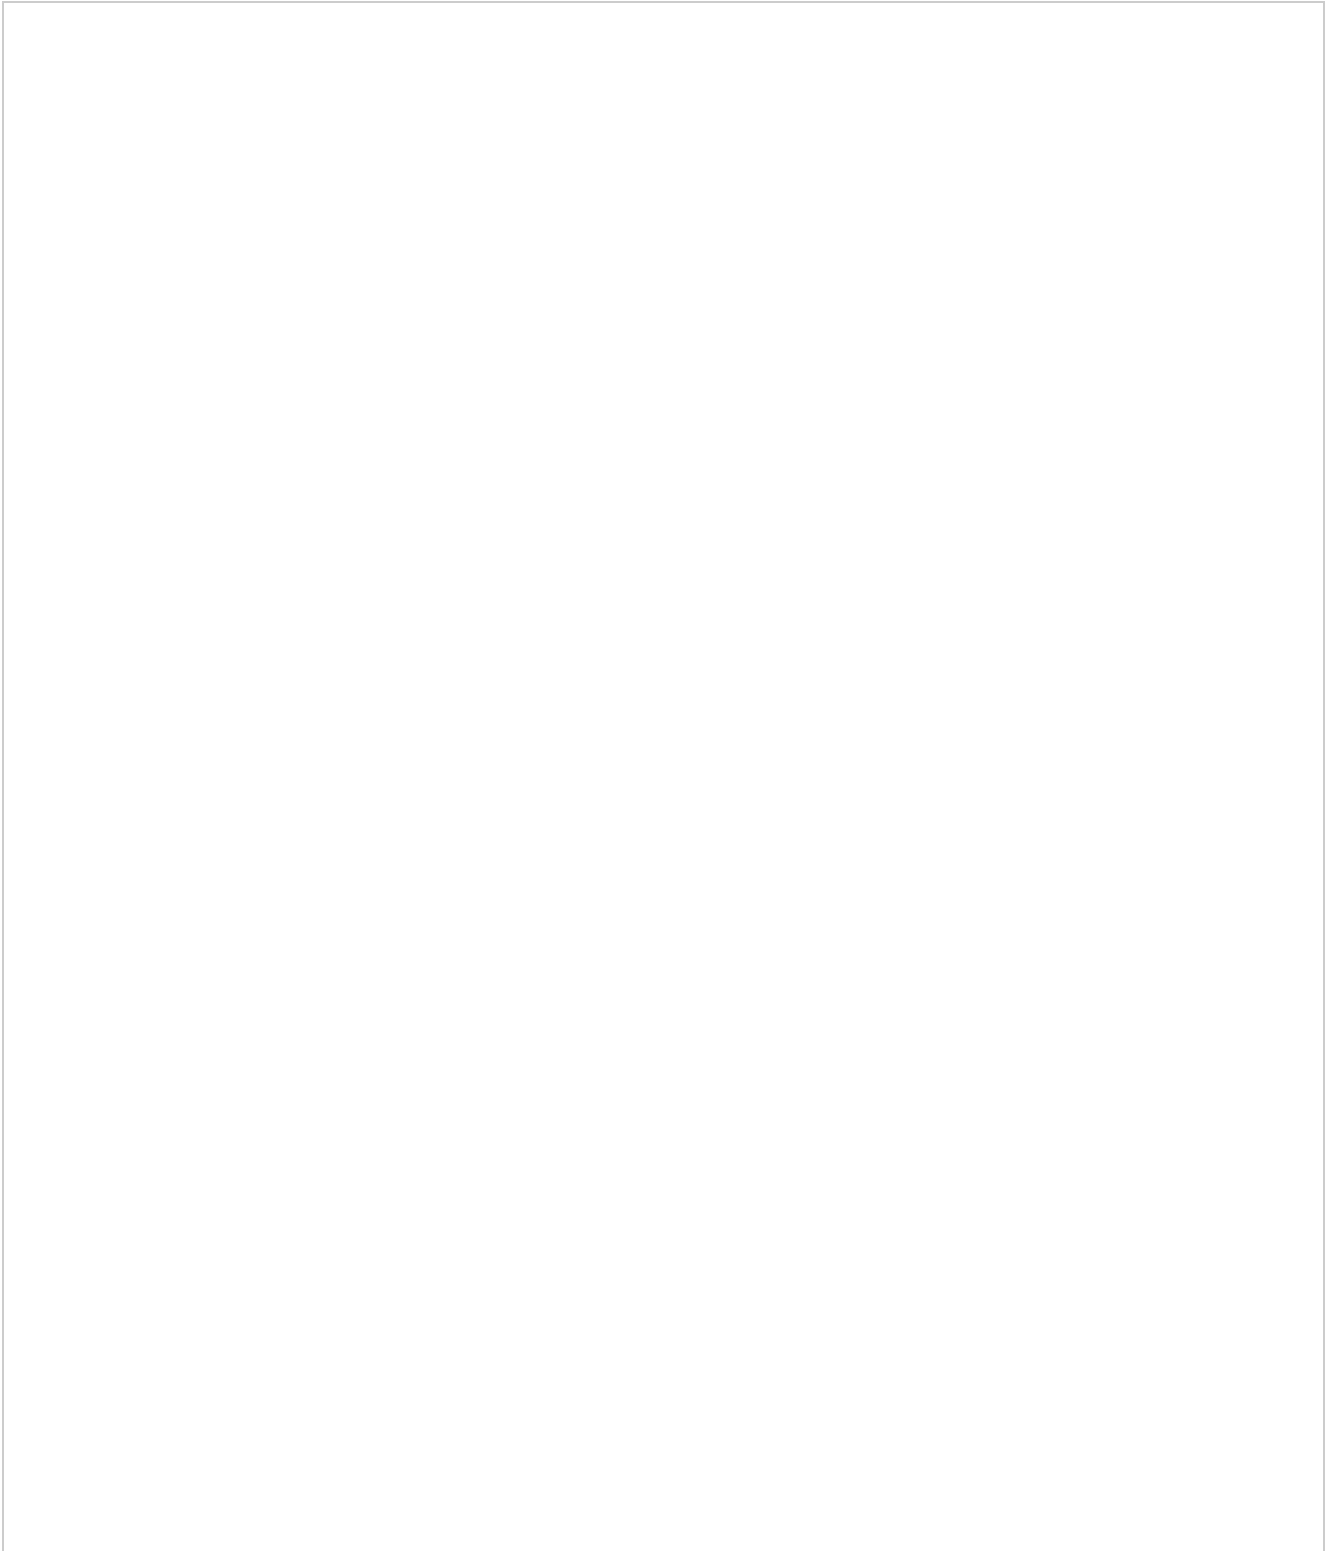

Please provide any of your comments on this color map.

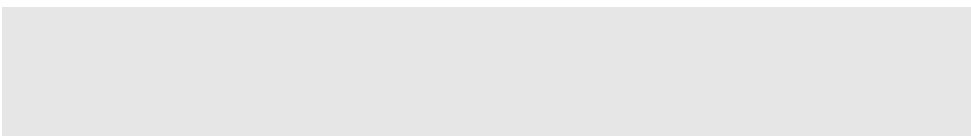

16. How many percentages do the highlighted area match with your clinical judgment on the important features to classify LGG/HGG?

0%, Not matches at all                      50%                      Completely matches with mine, 100%

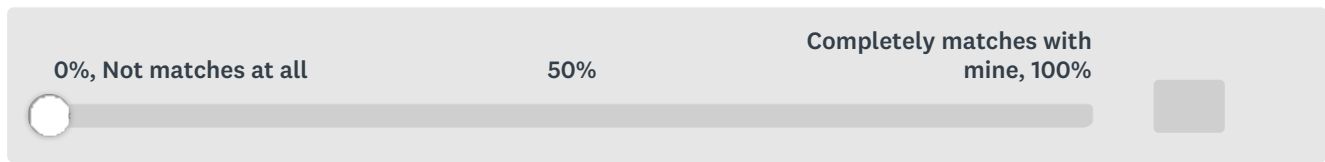A horizontal slider bar with a white circular knob at the 0% position. The bar is light gray with a darker gray track. The text "0%, Not matches at all" is at the left end, "50%" is in the middle, and "Completely matches with mine, 100%" is at the right end.☐

17. How helpful is this color map in clinical settings?

0, Not helpful at all                      5, Somewhat helpful                      Extremely helpful, 10

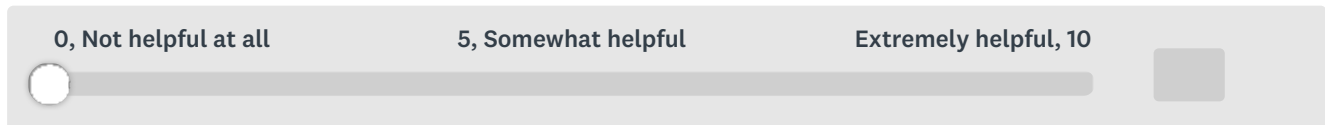A horizontal slider bar with a white circular knob at the 0 position. The bar is light gray with a darker gray track. The text "0, Not helpful at all" is at the left end, "5, Somewhat helpful" is in the middle, and "Extremely helpful, 10" is at the right end.☐

18. Did you notice the color map differences on different MRI modalities? How helpful is this feature in clinical settings?

0, Not helpful at all                      5, Somewhat helpful                      Extremely helpful, 10

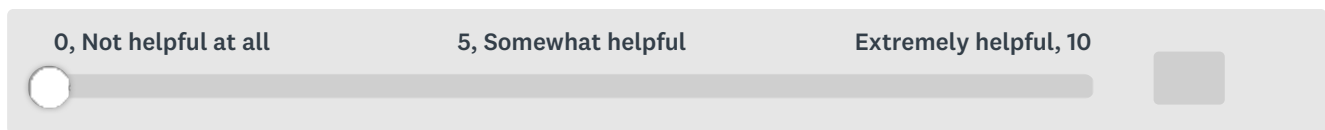A horizontal slider bar with a white circular knob at the 0 position. The bar is light gray with a darker gray track. The text "0, Not helpful at all" is at the left end, "5, Somewhat helpful" is in the middle, and "Extremely helpful, 10" is at the right end.☐

19.

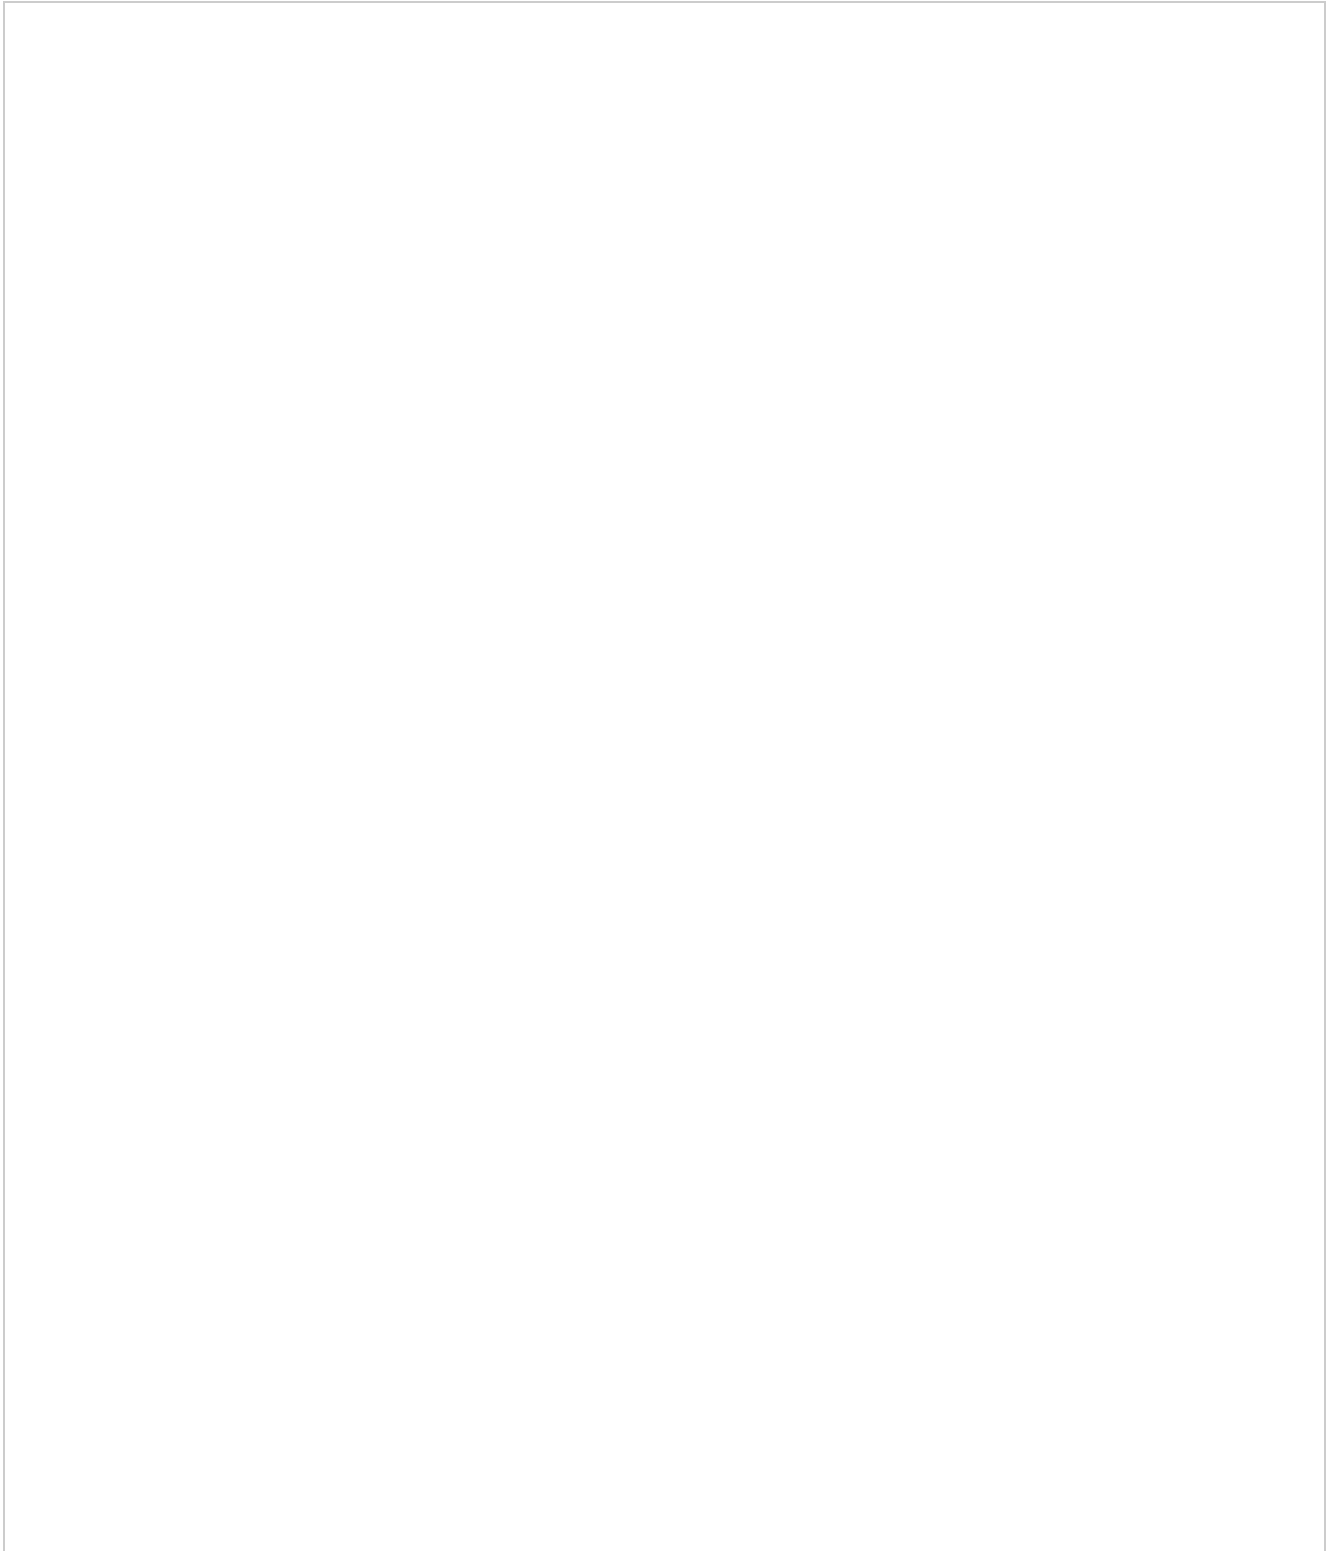

Please provide any of your comments on this color map.

A solid gray rectangular box, intended for providing comments on the color map.

20. How many percentages do the highlighted area match with your clinical judgment on the important features to classify LGG/HGG?

0%, Not matches at all                      50%                      Completely matches with mine, 100%

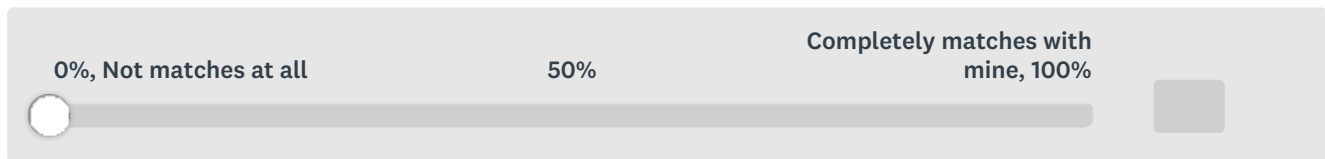A horizontal slider bar with a white circular knob at the 0% position. The bar is light gray and spans the width of the form.☐

21. How helpful is this color map in clinical settings?

0, Not helpful at all                      5, Somewhat helpful                      Extremely helpful, 10

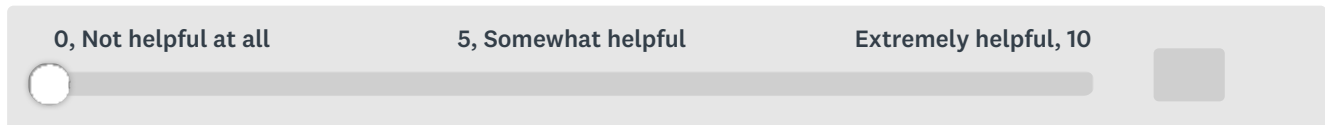A horizontal slider bar with a white circular knob at the 0 position. The bar is light gray and spans the width of the form.☐

22. Did you notice the color map differences on different MRI modalities? How helpful is this feature in clinical settings?

0, Not helpful at all                      5, Somewhat helpful                      Extremely helpful, 10

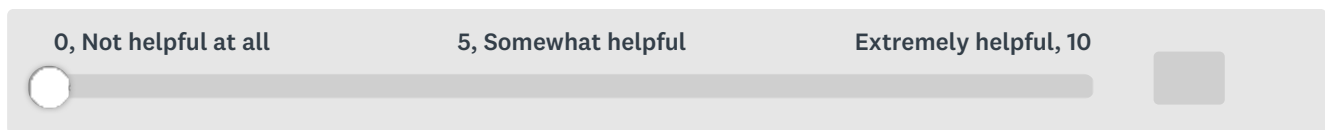A horizontal slider bar with a white circular knob at the 0 position. The bar is light gray and spans the width of the form.☐

**23.**

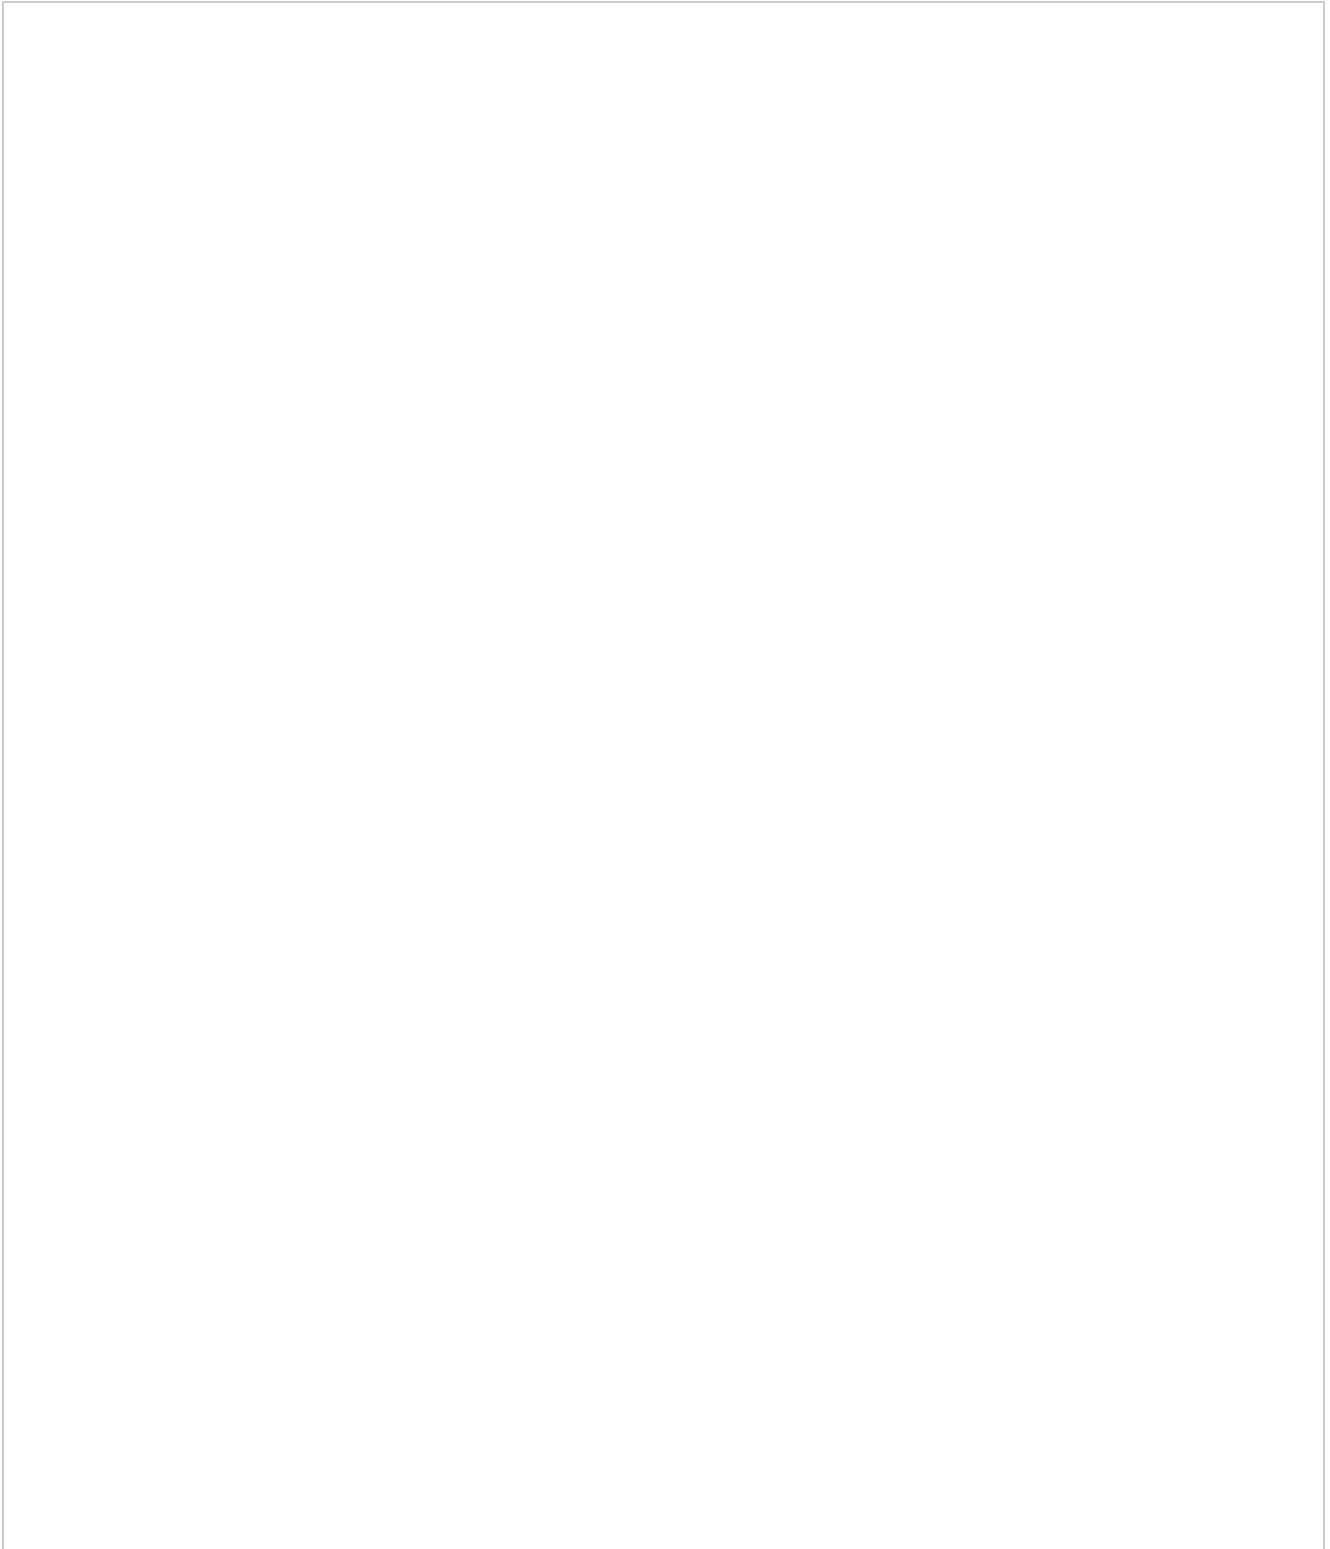

**Please provide any of your comments on this color map.**

A solid gray rectangular box, intended for providing comments or feedback on the color map.

24. How many percentages do the highlighted area match with your clinical judgment on the important features to classify LGG/HGG?

0%, Not matches at all                      50%                      Completely matches with mine, 100%

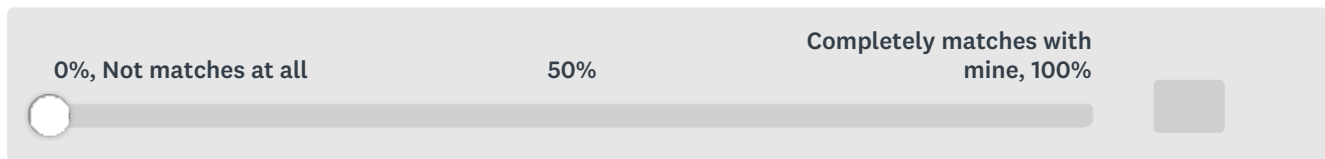A horizontal slider bar with a white circular knob at the 0% position. The bar is light gray and spans the width of the form.☐

25. How helpful is this color map in clinical settings?

0, Not helpful at all                      5, Somewhat helpful                      Extremely helpful, 10

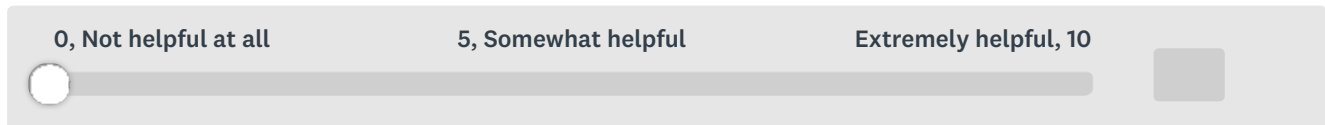A horizontal slider bar with a white circular knob at the 0 position. The bar is light gray and spans the width of the form.☐

26. Did you notice the color map differences on different MRI modalities? How helpful is this feature in clinical settings?

0, Not helpful at all                      5, Somewhat helpful                      Extremely helpful, 10

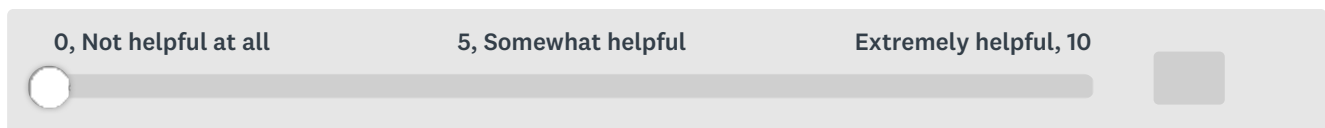A horizontal slider bar with a white circular knob at the 0 position. The bar is light gray and spans the width of the form.☐

**27.**

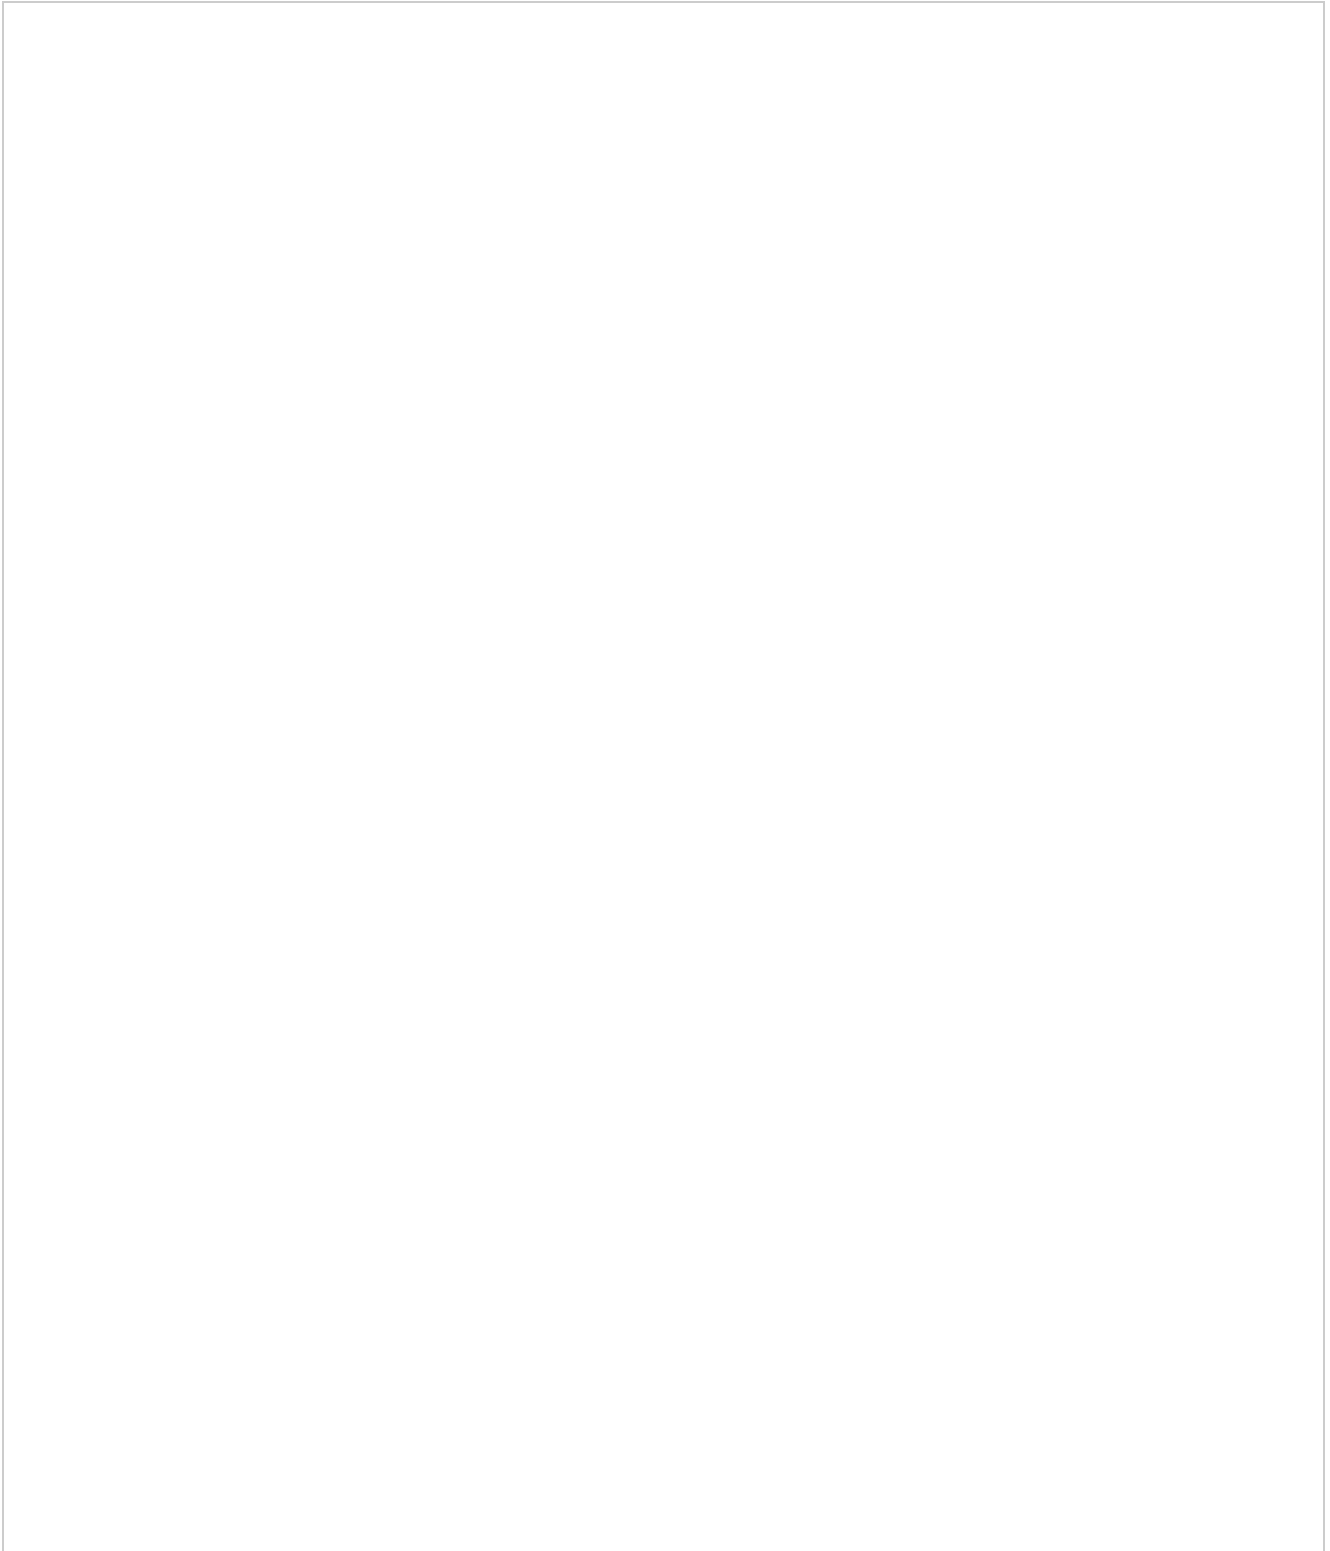

**Please provide any of your comments on this color map.**

A solid gray rectangular box, intended for providing comments on the color map.



28. How many percentages do the highlighted area match with your clinical judgment on the important features to classify LGG/HGG?

0%, Not matches at all                      50%                      Completely matches with mine, 100%

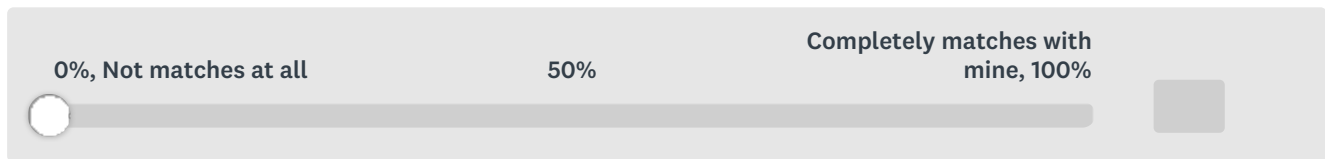

A horizontal slider bar with a white circular knob at the 0% position. The bar is light gray and spans the width of the form. To the right of the bar is a small gray square button.

29. How helpful is this color map in clinical settings?

0, Not helpful at all                      5, Somewhat helpful                      Extremely helpful, 10

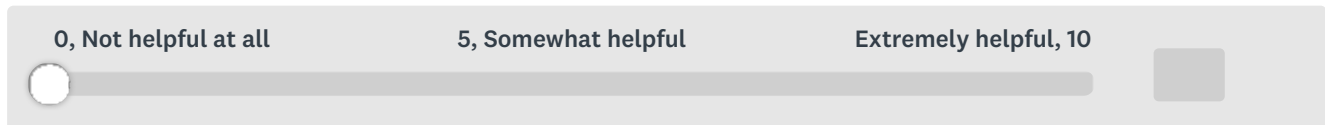

A horizontal slider bar with a white circular knob at the 0 position. The bar is light gray and spans the width of the form. To the right of the bar is a small gray square button.

30. Did you notice the **color map differences** on different **MRI modalities**? How helpful is this feature in clinical settings?

0, Not helpful at all                      5, Somewhat helpful                      Extremely helpful, 10

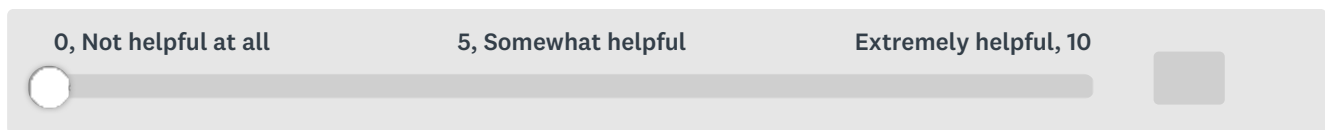

A horizontal slider bar with a white circular knob at the 0 position. The bar is light gray and spans the width of the form. To the right of the bar is a small gray square button.

31.

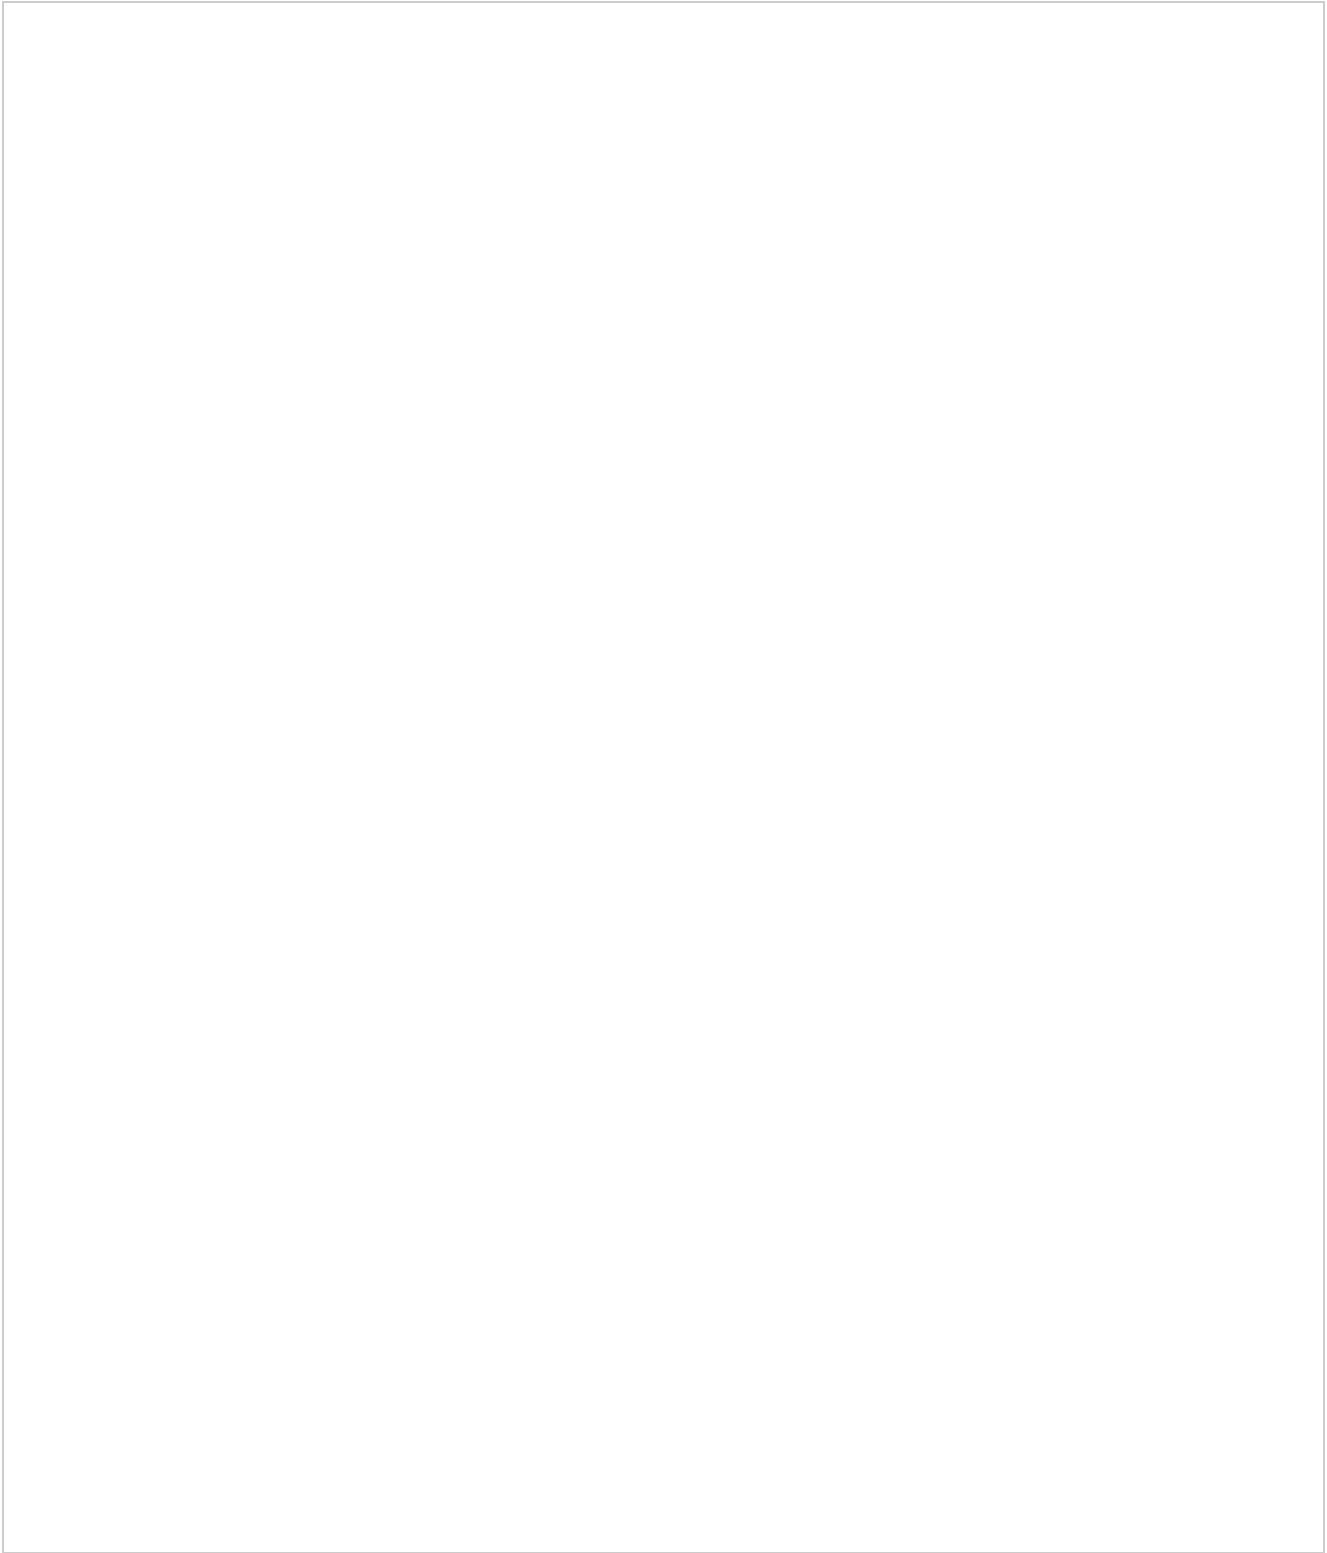

Please provide any of your comments on this color map.

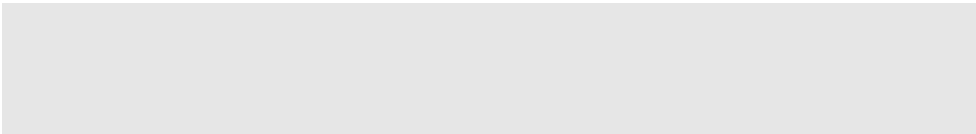

32. How many percentages do the highlighted area match with your clinical judgment on the important features to classify LGG/HGG?

0%, Not matches at all                      50%                      Completely matches with mine, 100%

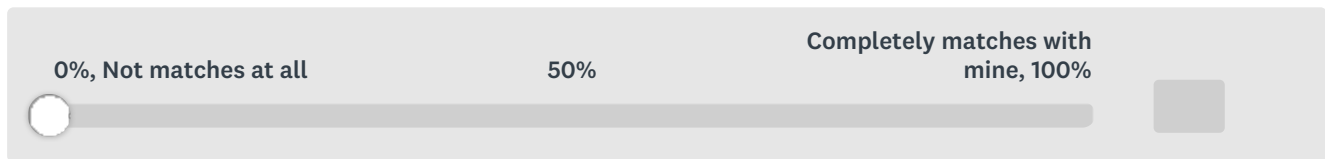A horizontal slider bar with a white circular knob at the 0% position. The bar is light gray and spans the width of the form.☐

33. How helpful is this color map in clinical settings?

0, Not helpful at all                      5, Somewhat helpful                      Extremely helpful, 10

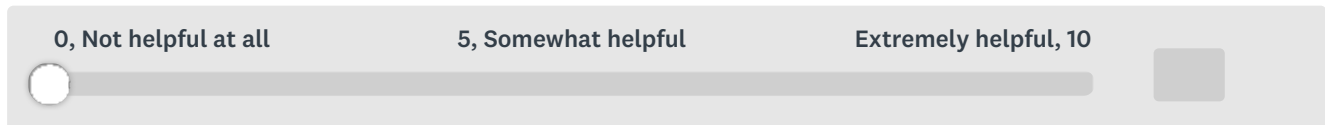A horizontal slider bar with a white circular knob at the 0 position. The bar is light gray and spans the width of the form.☐

34. Did you notice the color map differences on different MRI modalities? How helpful is this feature in clinical settings?

0, Not helpful at all                      5, Somewhat helpful                      Extremely helpful, 10

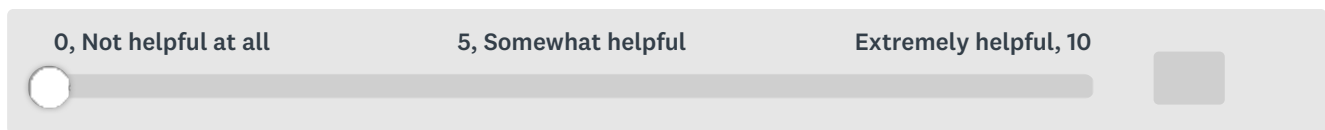A horizontal slider bar with a white circular knob at the 0 position. The bar is light gray and spans the width of the form.☐

35.

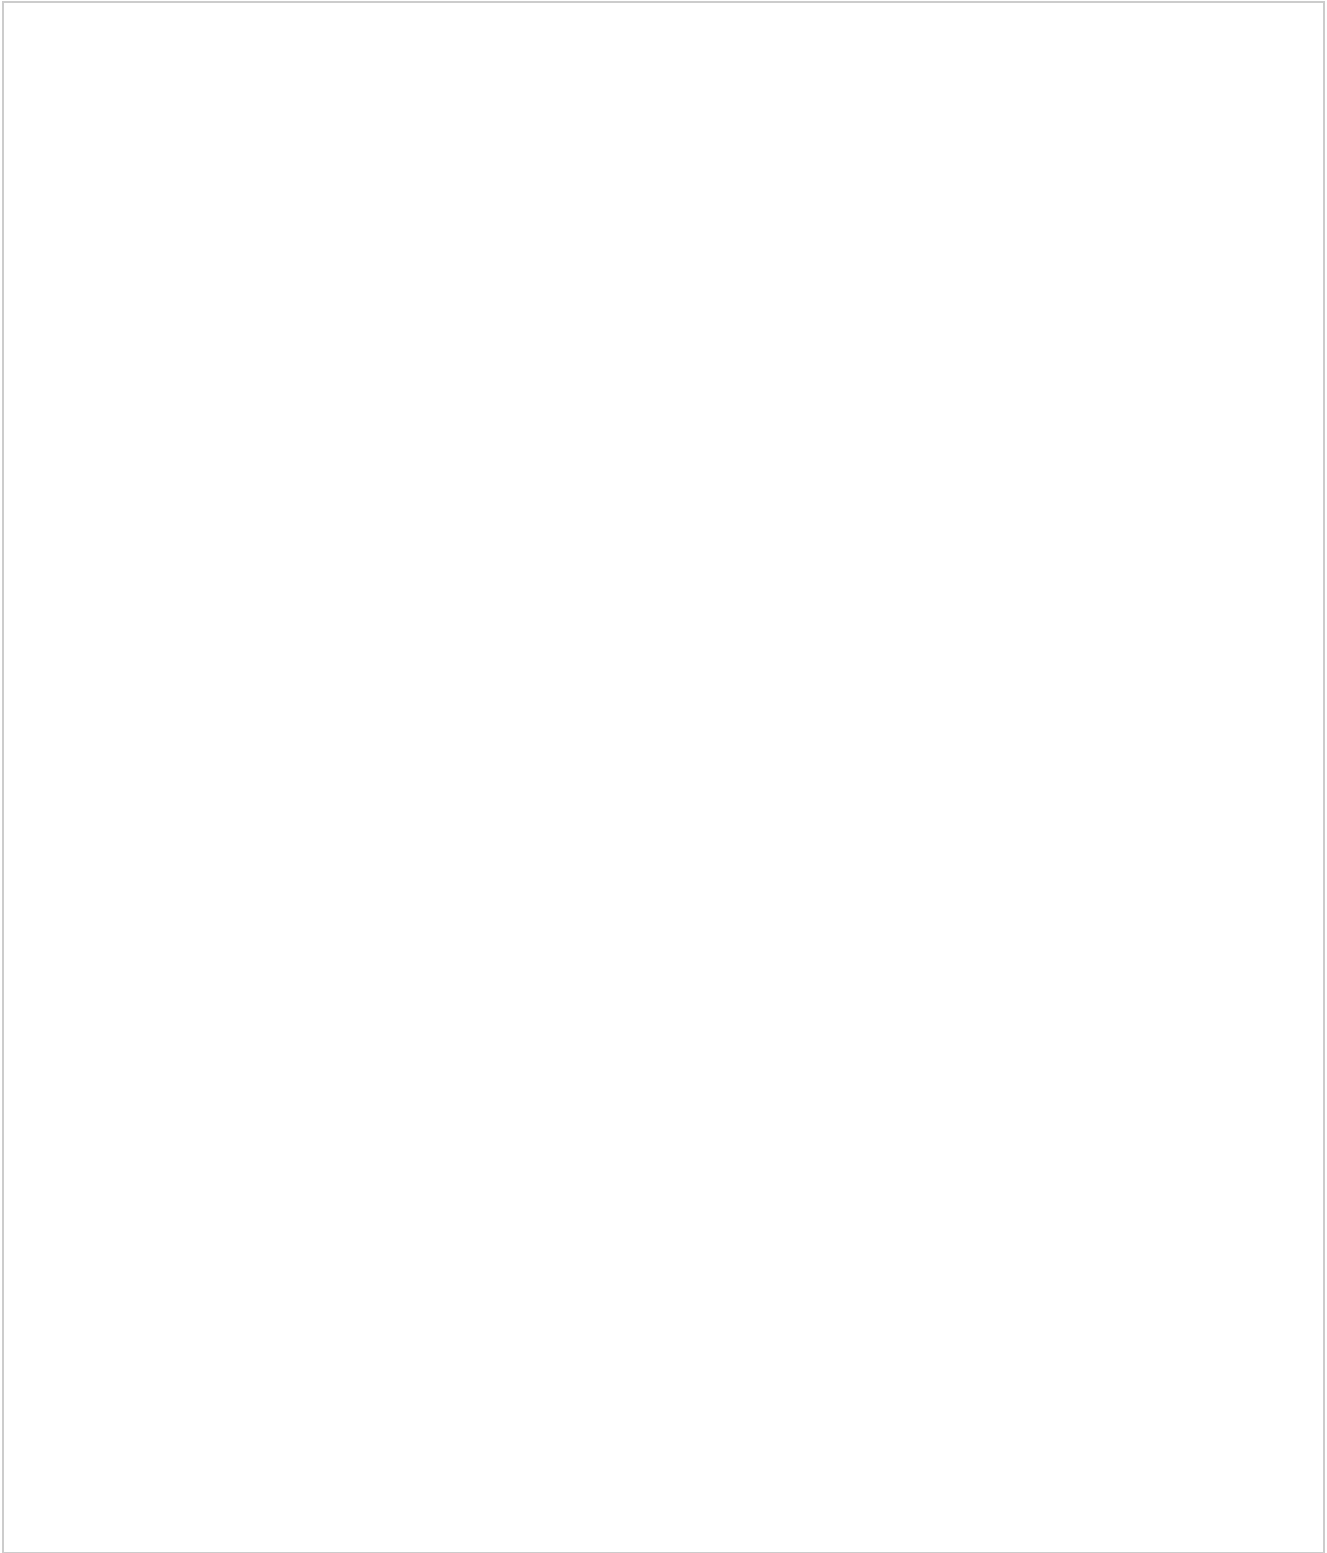

Please provide any of your comments on this color map.

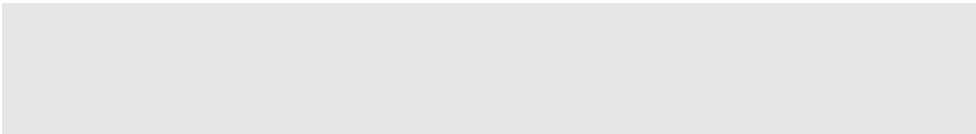

36. How many percentages do the highlighted area match with your clinical judgment on the important features to classify LGG/HGG?

0%, Not matches at all                      50%                      Completely matches with mine, 100%

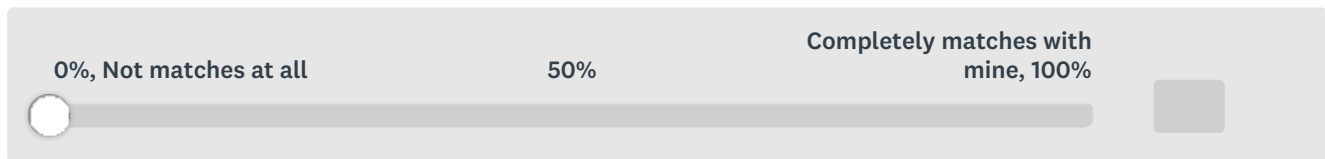A horizontal slider bar with a white circular knob at the 0% position. The bar is light gray and spans the width of the question area.☐

37. How helpful is this color map in clinical settings?

0, Not helpful at all                      5, Somewhat helpful                      Extremely helpful, 10

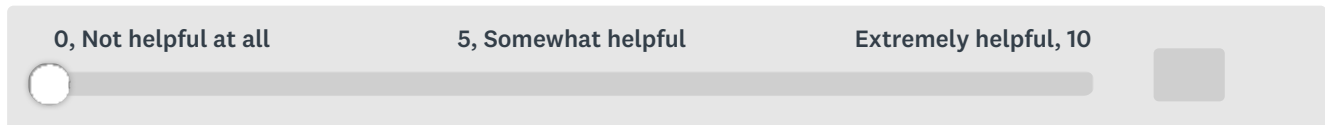A horizontal slider bar with a white circular knob at the 0 position. The bar is light gray and spans the width of the question area.☐

38. Did you notice the color map differences on different MRI modalities? How helpful is this feature in clinical settings?

0, Not helpful at all                      5, Somewhat helpful                      Extremely helpful, 10

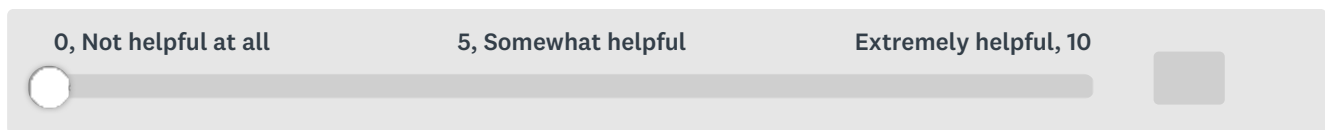A horizontal slider bar with a white circular knob at the 0 position. The bar is light gray and spans the width of the question area.☐

39.

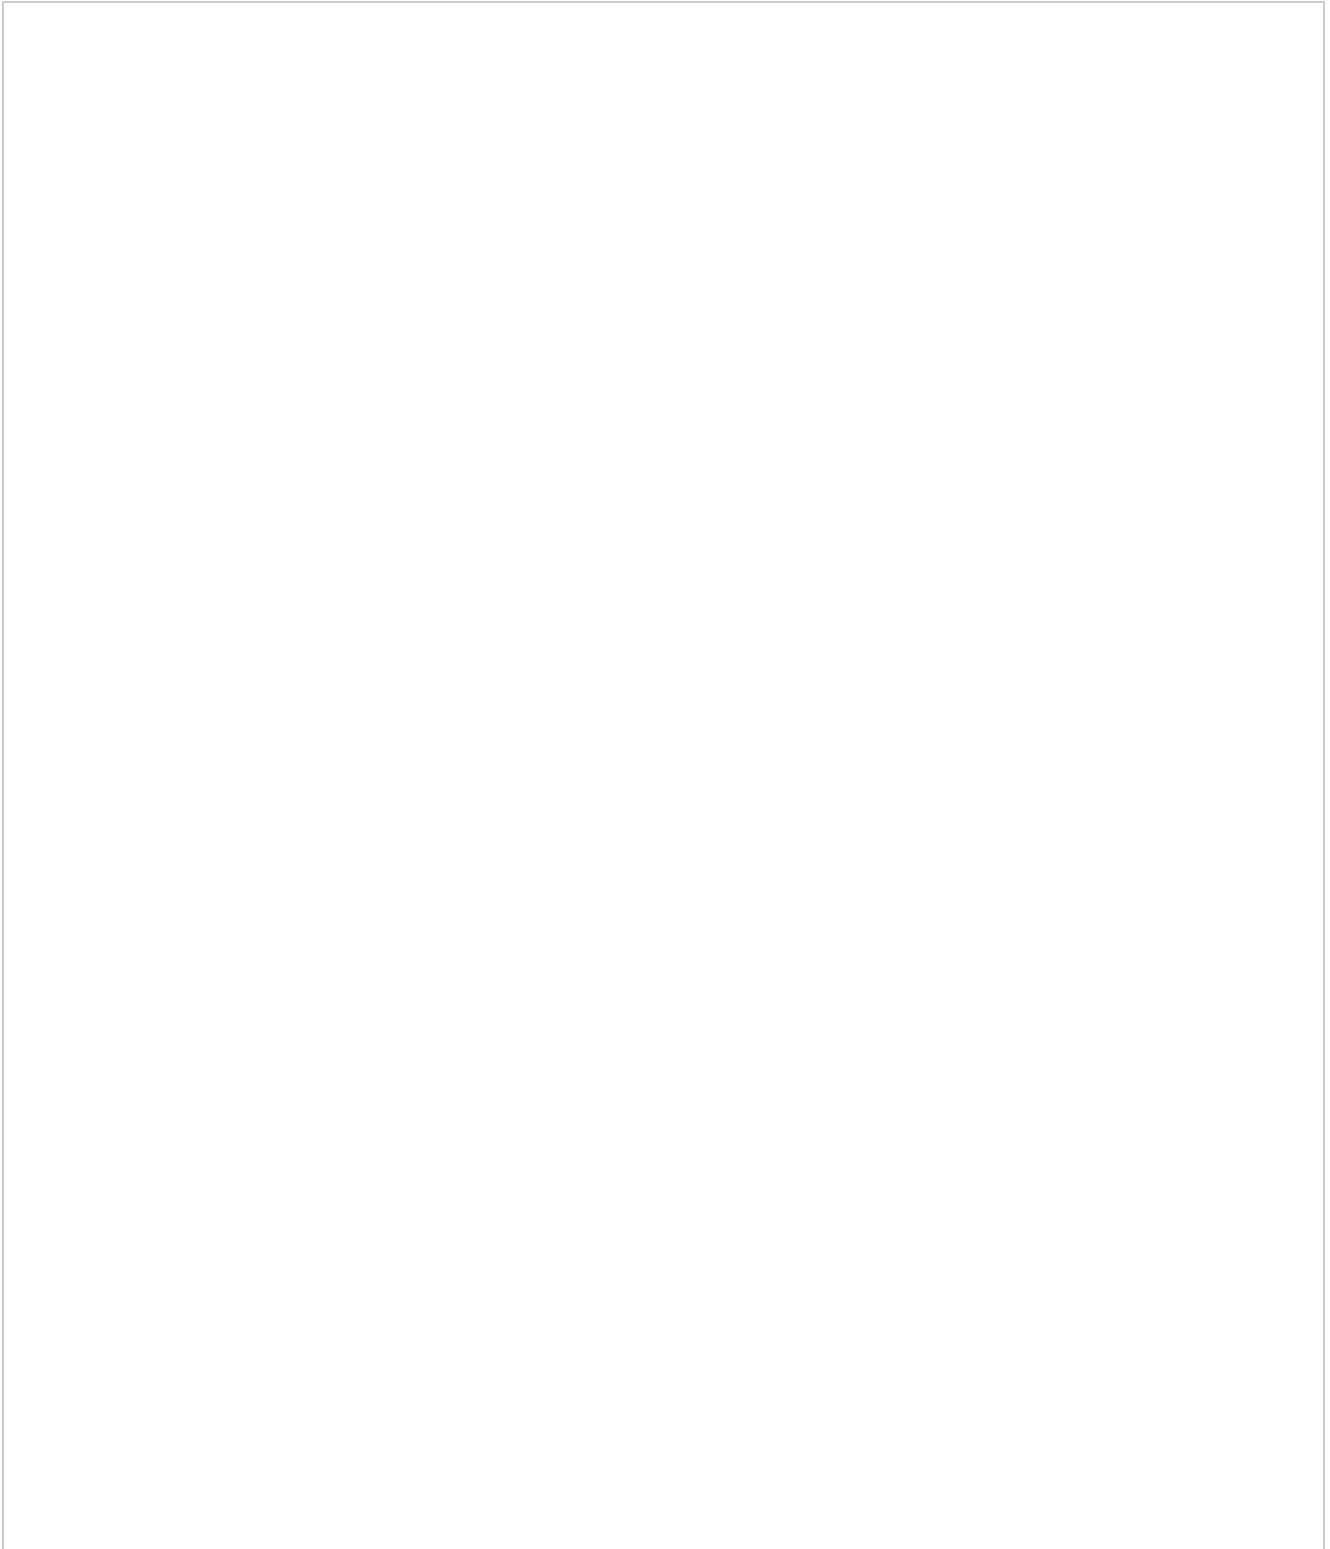

Please provide any of your comments on this color map.

A solid gray rectangular box, intended for providing comments or feedback on the color map.

40. How many percentages do the highlighted area match with your clinical judgment on the important features to classify LGG/HGG?

0%, Not matches at all                      50%                      Completely matches with mine, 100%

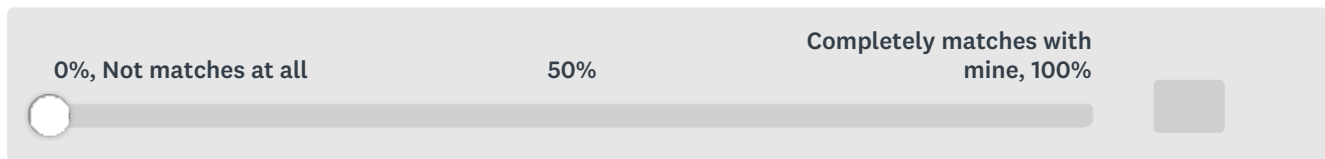A horizontal slider bar with a white circular knob at the 0% position. The bar is light gray with a darker gray track. The text "0%, Not matches at all" is on the left, "50%" is in the middle, and "Completely matches with mine, 100%" is on the right.☐

41. How helpful is this color map in clinical settings?

0, Not helpful at all                      5, Somewhat helpful                      Extremely helpful, 10

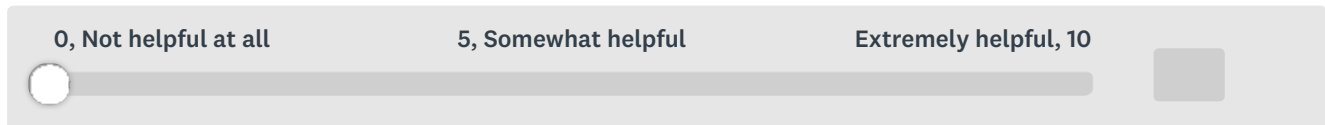A horizontal slider bar with a white circular knob at the 0 position. The bar is light gray with a darker gray track. The text "0, Not helpful at all" is on the left, "5, Somewhat helpful" is in the middle, and "Extremely helpful, 10" is on the right.☐

42. Did you notice the color map differences on different MRI modalities? How helpful is this feature in clinical settings?

0, Not helpful at all                      5, Somewhat helpful                      Extremely helpful, 10

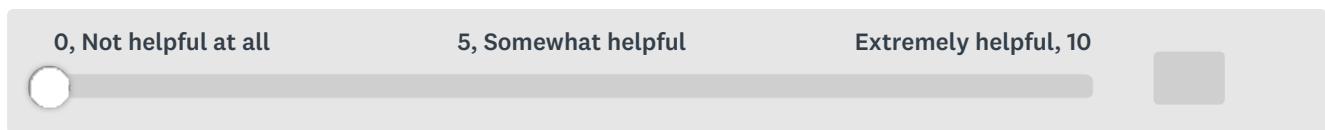A horizontal slider bar with a white circular knob at the 0 position. The bar is light gray with a darker gray track. The text "0, Not helpful at all" is on the left, "5, Somewhat helpful" is in the middle, and "Extremely helpful, 10" is on the right.☐

43.

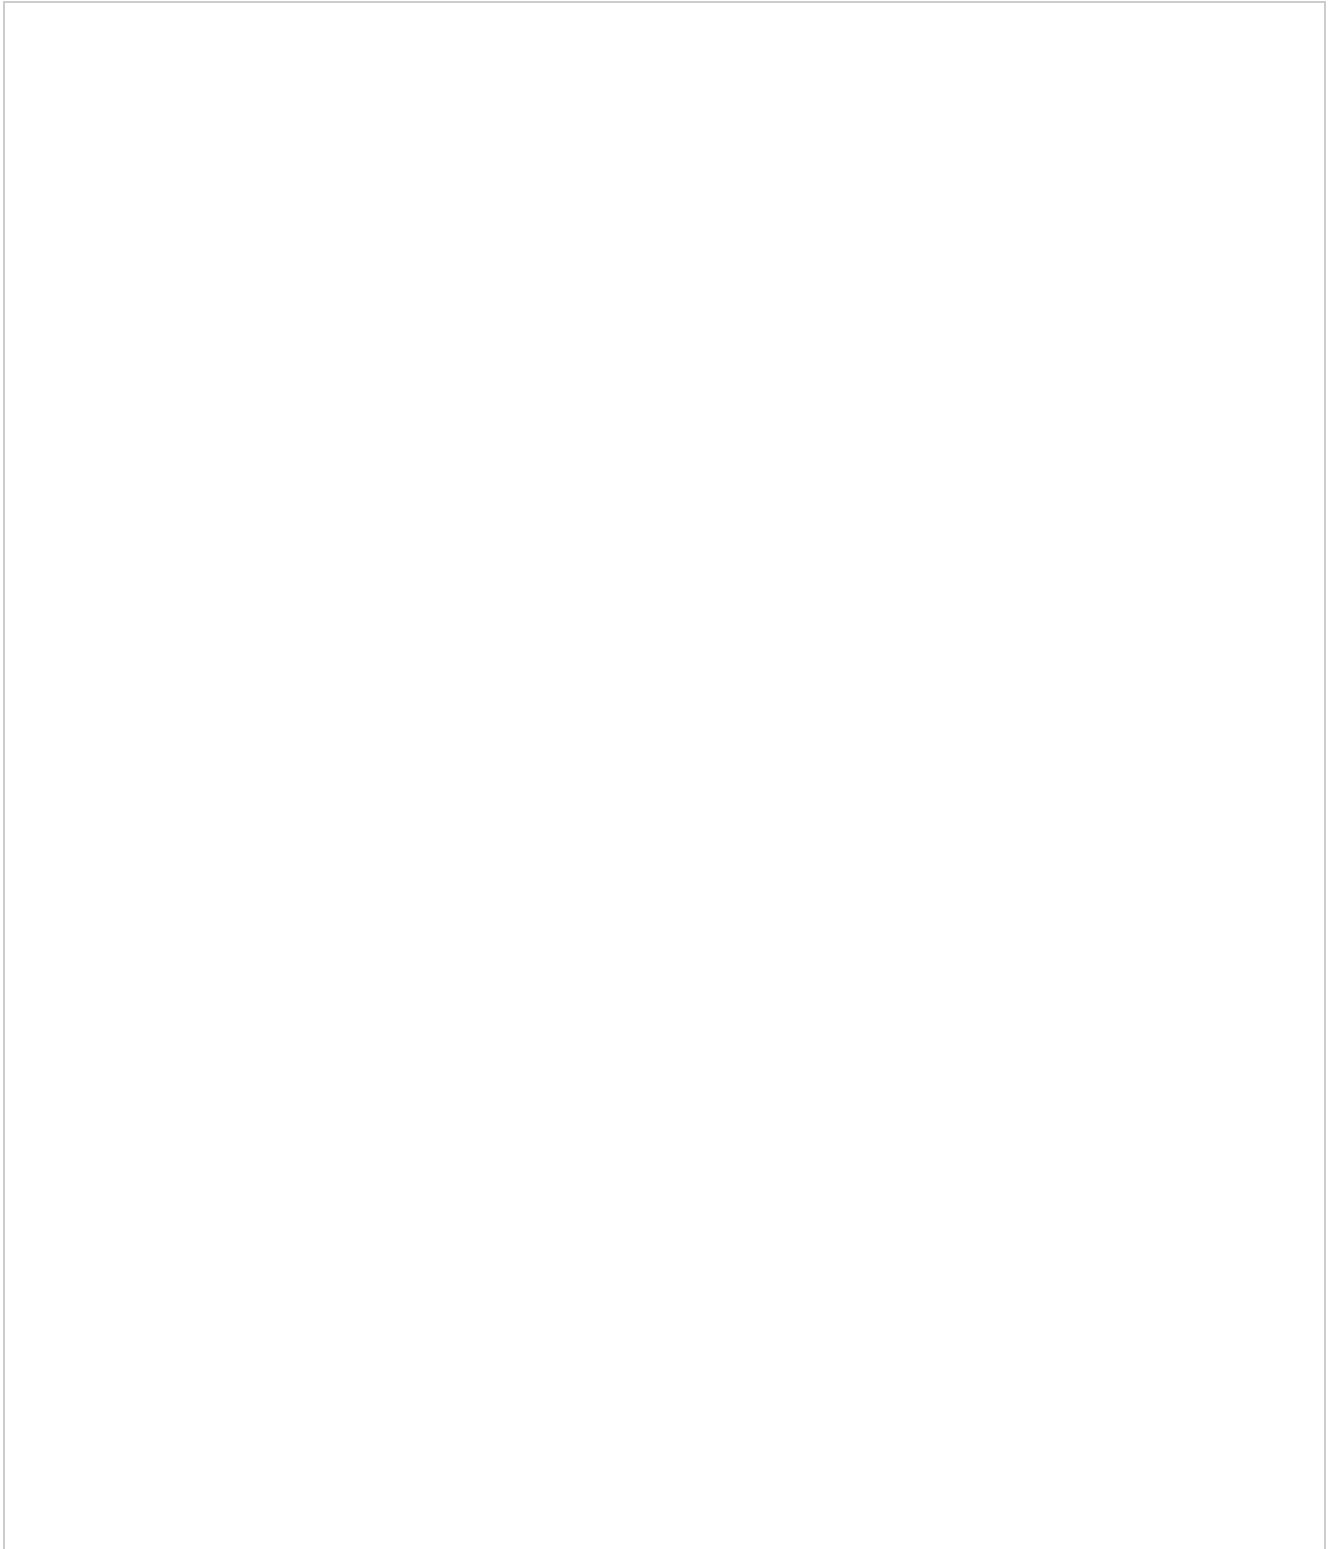

Please provide any of your comments on this color map.

A solid gray rectangular box, intended for providing comments or feedback on the color map.



44. How many percentages do the highlighted area match with your clinical judgment on the important features to classify LGG/HGG?

0%, Not matches at all                      50%                      Completely matches with mine, 100%

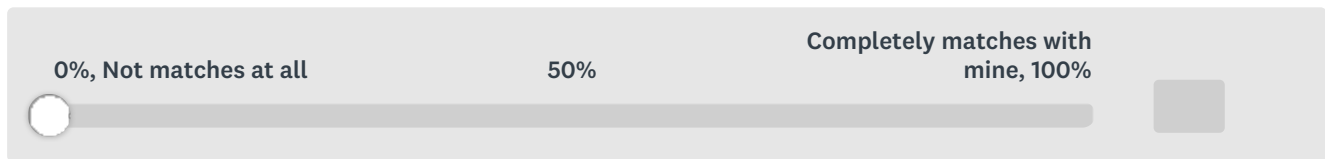A horizontal slider bar with a white circular knob at the 0% position. The bar is light gray with a darker gray track. The text "0%, Not matches at all" is on the left, "50%" is in the middle, and "Completely matches with mine, 100%" is on the right.☐

45. How helpful is this color map in clinical settings?

0, Not helpful at all                      5, Somewhat helpful                      Extremely helpful, 10

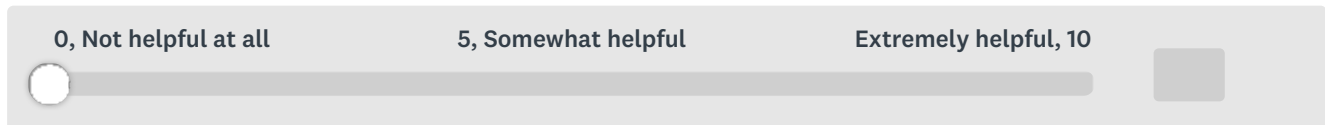A horizontal slider bar with a white circular knob at the 0 position. The bar is light gray with a darker gray track. The text "0, Not helpful at all" is on the left, "5, Somewhat helpful" is in the middle, and "Extremely helpful, 10" is on the right.☐

46. Did you notice the **color map differences** on **different MRI modalities**? How helpful is this feature in clinical settings?

0, Not helpful at all                      5, Somewhat helpful                      Extremely helpful, 10

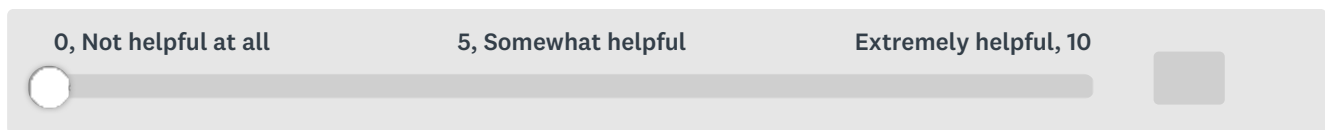A horizontal slider bar with a white circular knob at the 0 position. The bar is light gray with a darker gray track. The text "0, Not helpful at all" is on the left, "5, Somewhat helpful" is in the middle, and "Extremely helpful, 10" is on the right.☐

47.

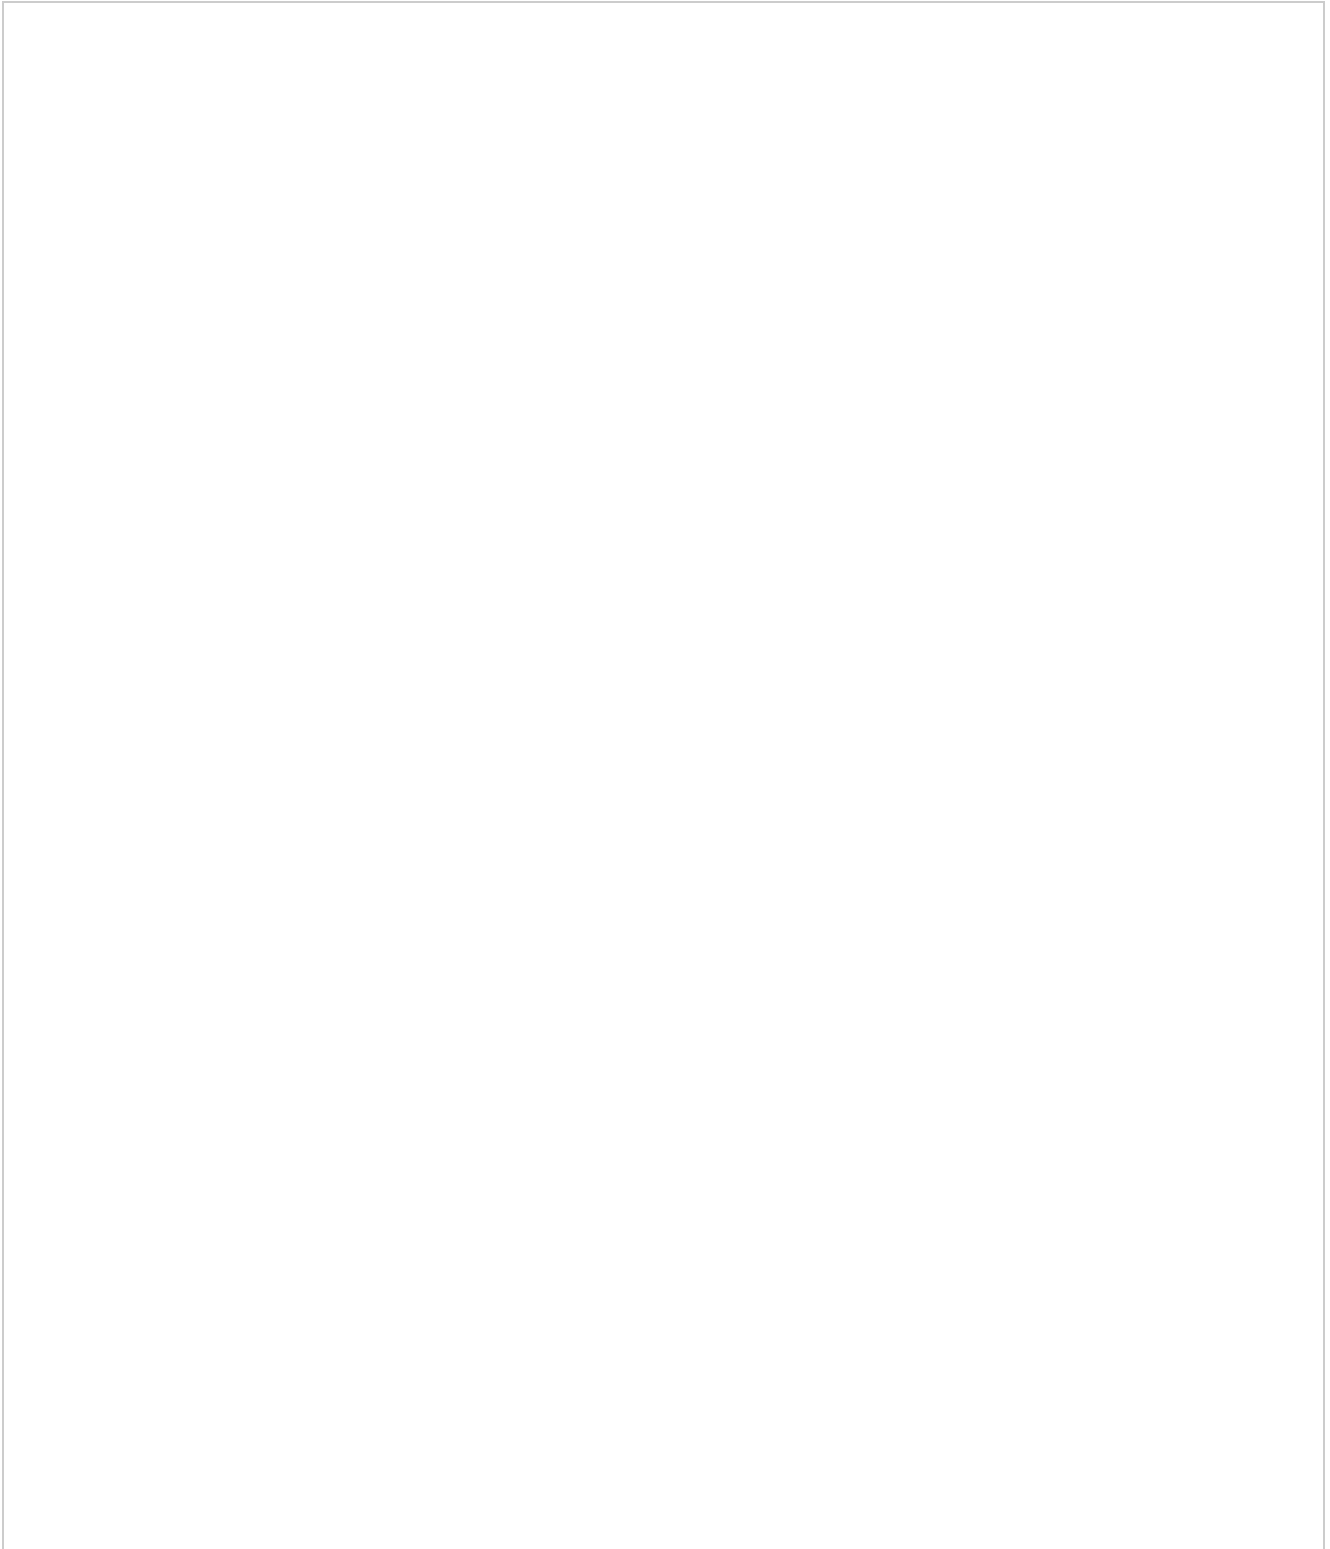

Please provide any of your comments on this color map.

A solid gray rectangular box, intended for providing comments or feedback on the color map.

48. How many percentages do the highlighted area match with your clinical judgment on the important features to classify LGG/HGG?

0%, Not matches at all                      50%                      Completely matches with mine, 100%

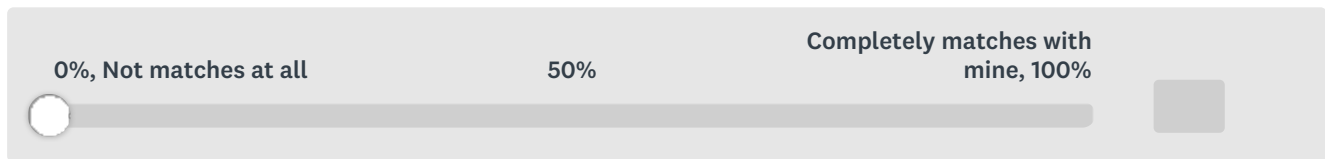A horizontal slider bar with a white circular knob at the 0% position. The bar is light gray and has a darker gray segment at the end. A small gray square button is located to the right of the slider.

49. How helpful is this color map in clinical settings?

0, Not helpful at all                      5, Somewhat helpful                      Extremely helpful, 10

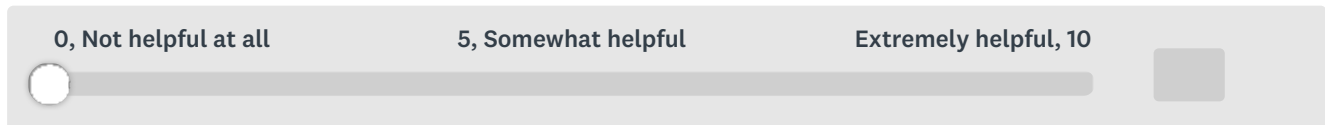A horizontal slider bar with a white circular knob at the 0 position. The bar is light gray and has a darker gray segment at the end. A small gray square button is located to the right of the slider.

50. Did you notice the color map differences on different MRI modalities? How helpful is this feature in clinical settings?

0, Not helpful at all                      5, Somewhat helpful                      Extremely helpful, 10

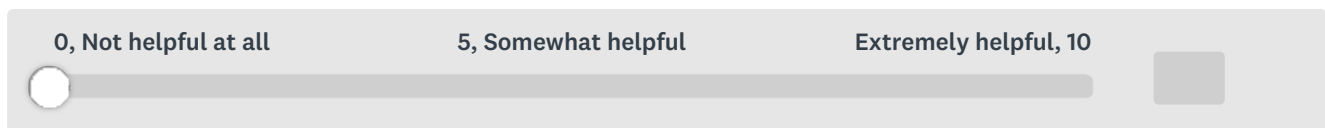A horizontal slider bar with a white circular knob at the 0 position. The bar is light gray and has a darker gray segment at the end. A small gray square button is located to the right of the slider.

51.

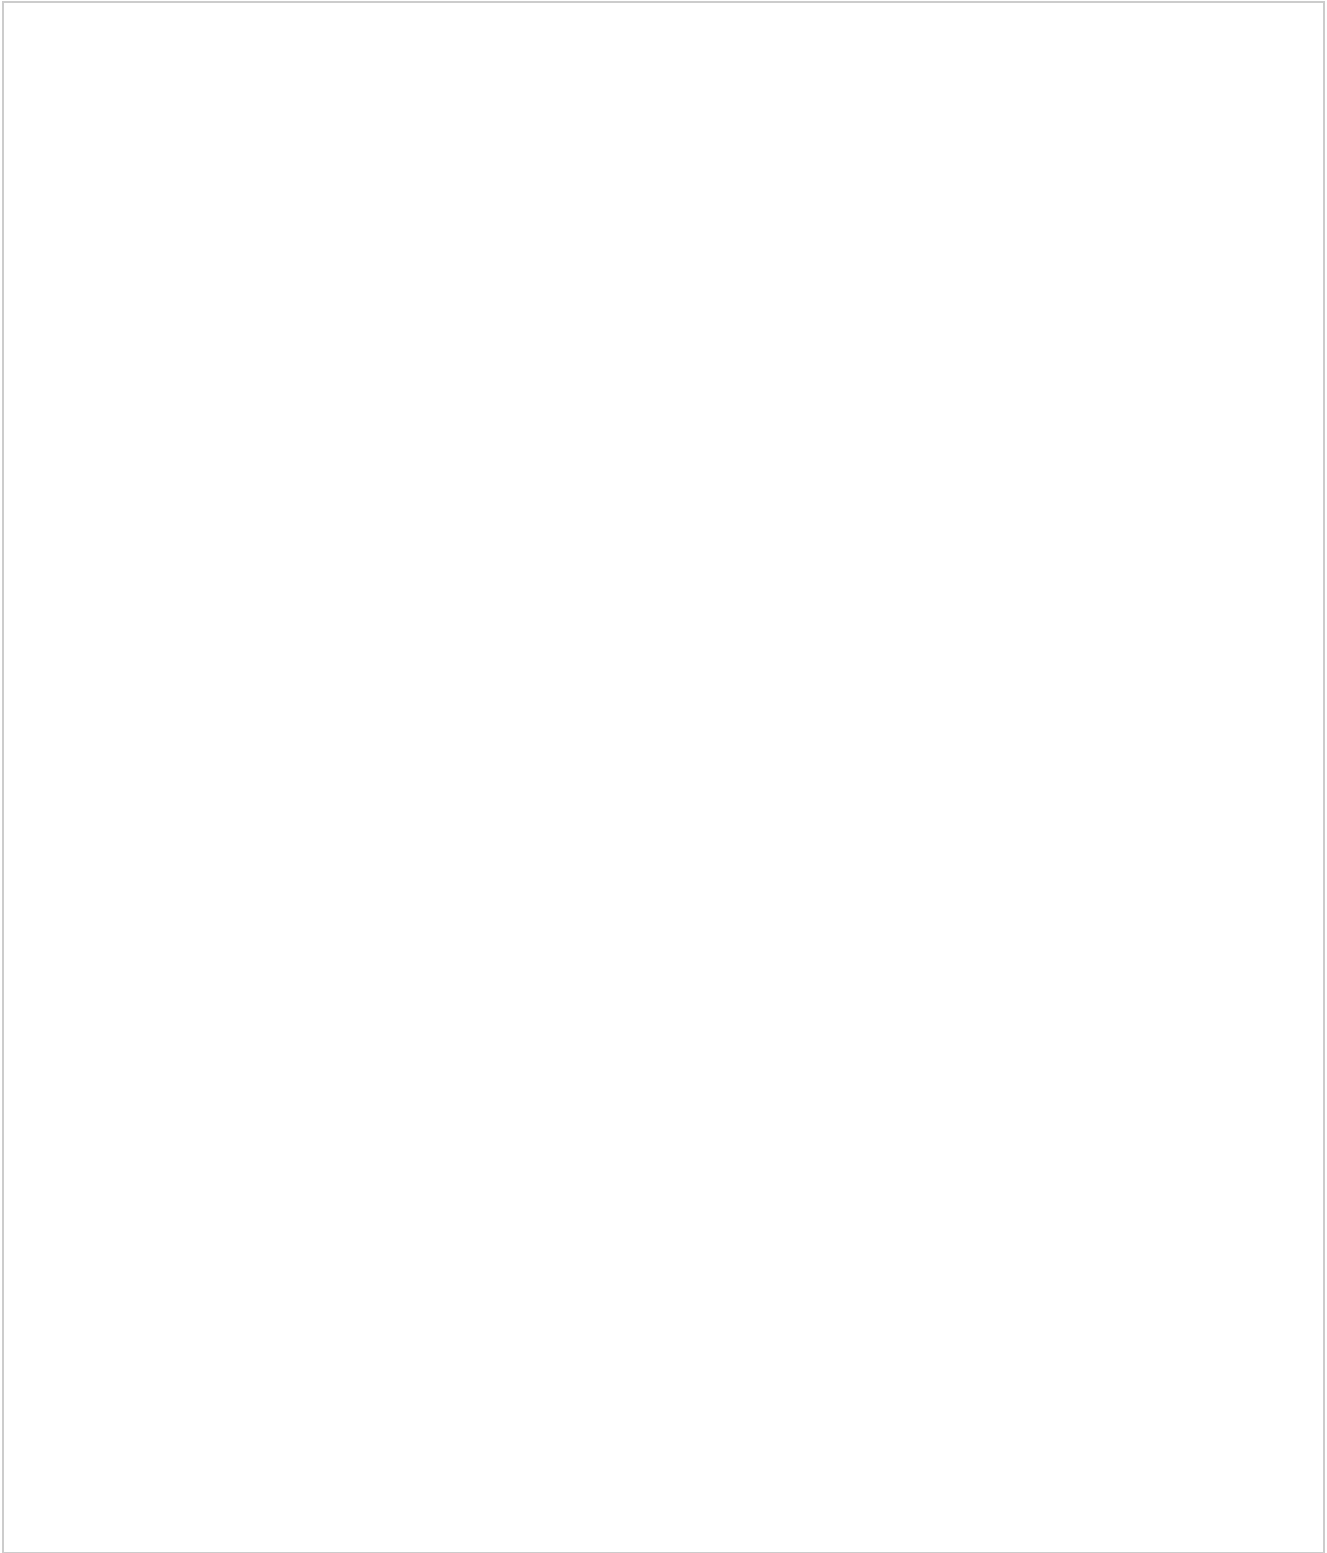

Please provide any of your comments on this color map.

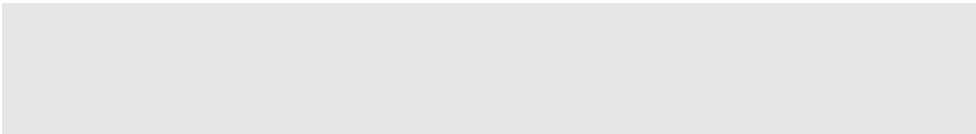

52. How many percentages do the highlighted area match with your clinical judgment on the important features to classify LGG/HGG?

0%, Not matches at all                      50%                      Completely matches with mine, 100%

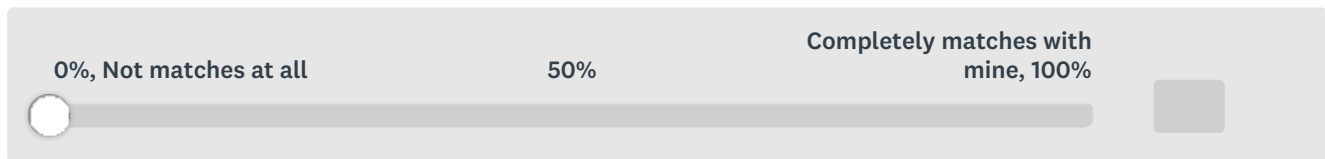A horizontal slider bar with a white circular knob at the 0% position. The bar is light gray and has a darker gray track. A small gray square button is located at the right end of the slider.

53. How helpful is this color map in clinical settings?

0, Not helpful at all                      5, Somewhat helpful                      Extremely helpful, 10

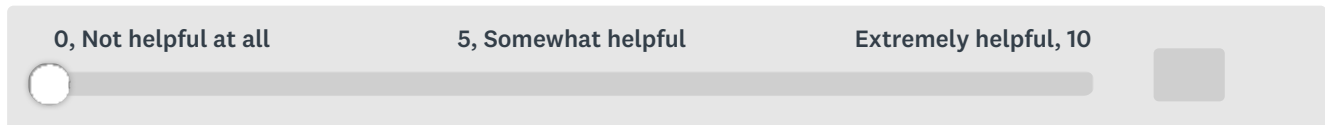A horizontal slider bar with a white circular knob at the 0 position. The bar is light gray and has a darker gray track. A small gray square button is located at the right end of the slider.

54. Did you notice the color map differences on different MRI modalities? How helpful is this feature in clinical settings?

0, Not helpful at all                      5, Somewhat helpful                      Extremely helpful, 10

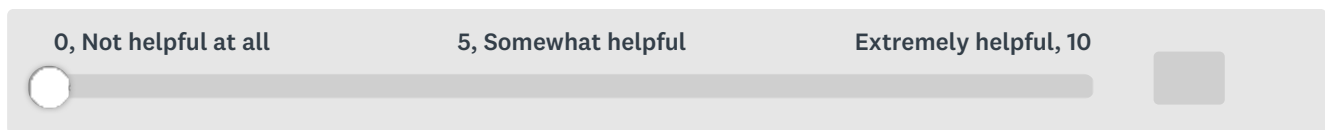A horizontal slider bar with a white circular knob at the 0 position. The bar is light gray and has a darker gray track. A small gray square button is located at the right end of the slider.

55.

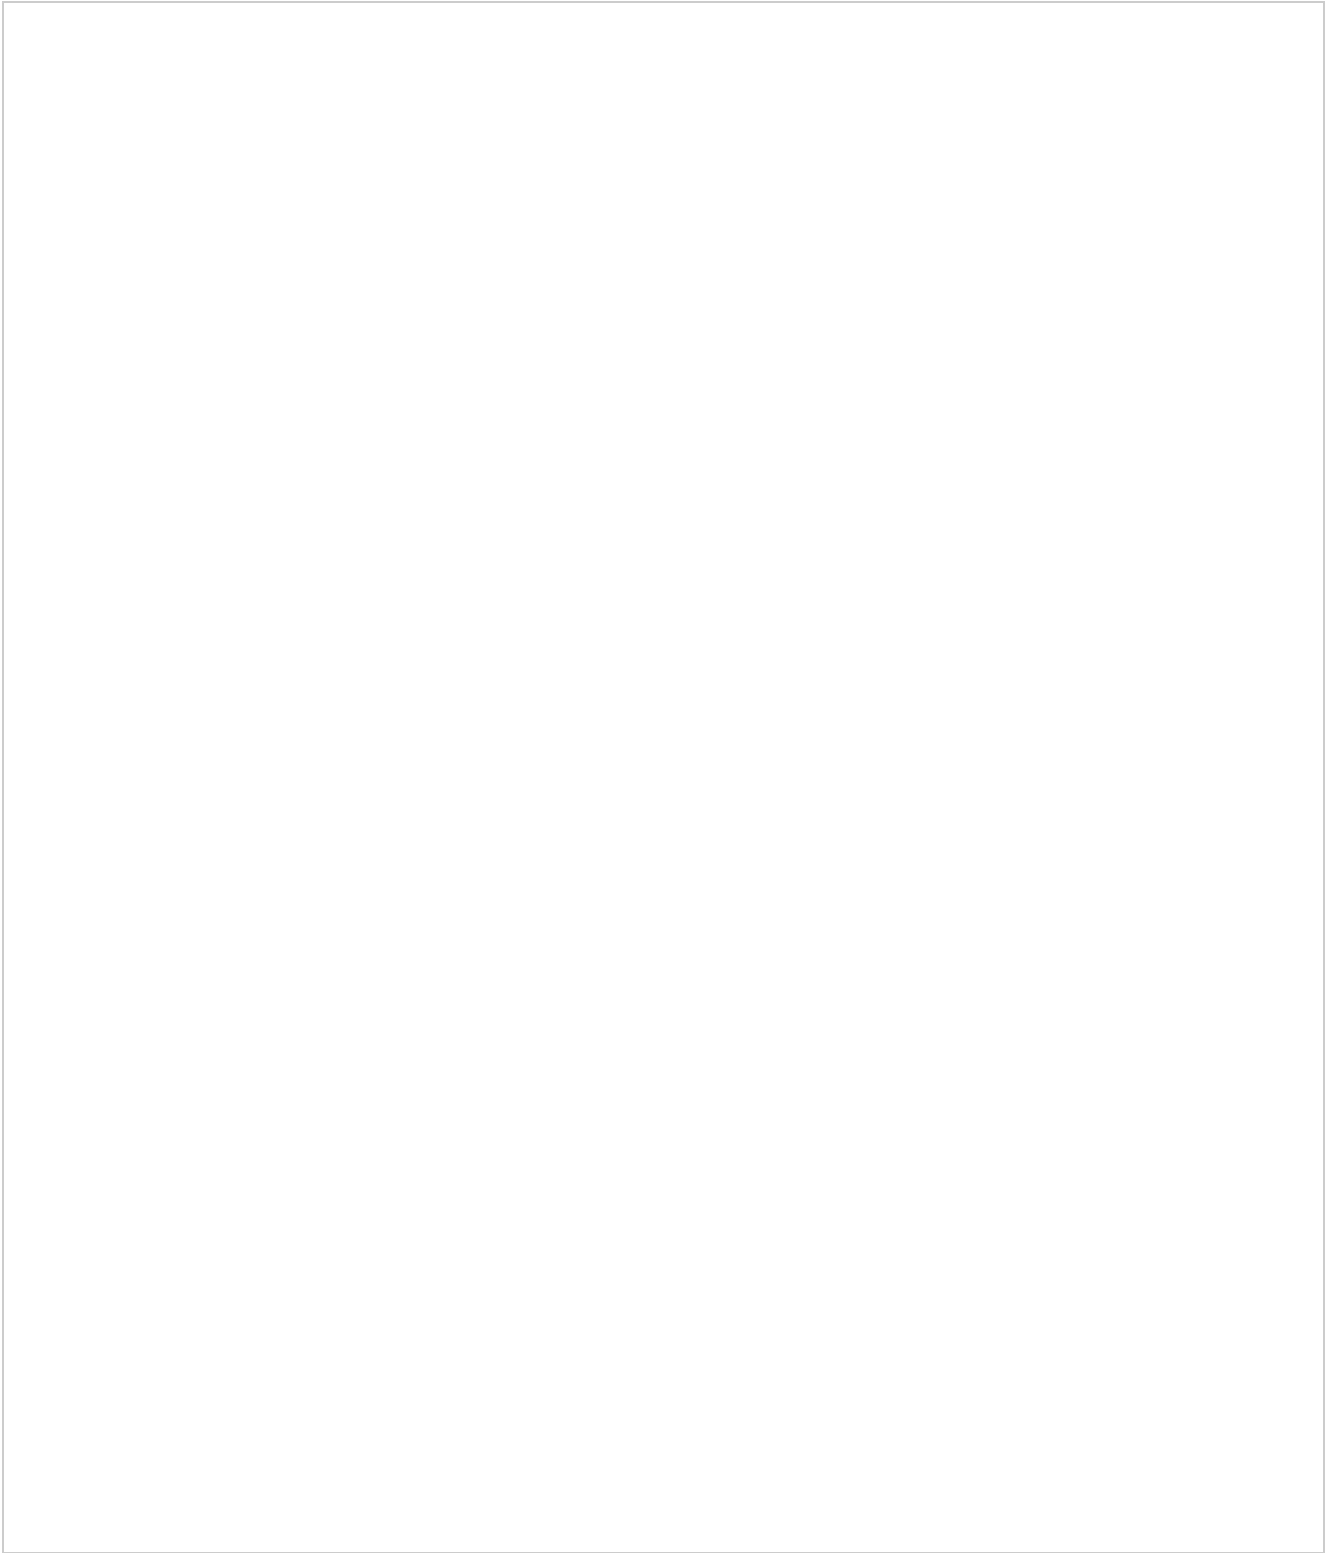

Please provide any of your comments on this color map.

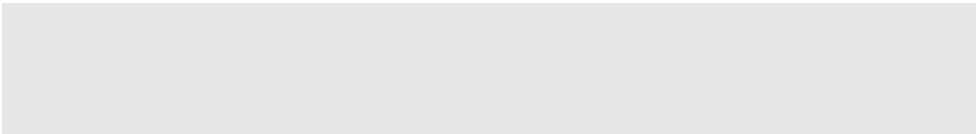

56. How many percentages do the highlighted area match with your clinical judgment on the important features to classify LGG/HGG?

0%, Not matches at all                      50%                      Completely matches with mine, 100%

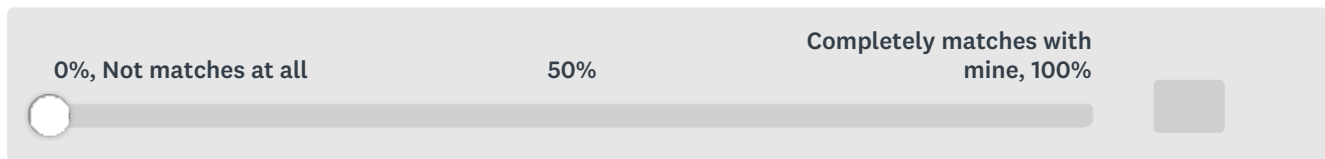A horizontal slider bar with a white circular knob at the 0% position. The bar is light gray with a darker gray track. The text "0%, Not matches at all" is at the left end, "50%" is in the middle, and "Completely matches with mine, 100%" is at the right end.☐

57. How helpful is this color map in clinical settings?

0, Not helpful at all                      5, Somewhat helpful                      Extremely helpful, 10

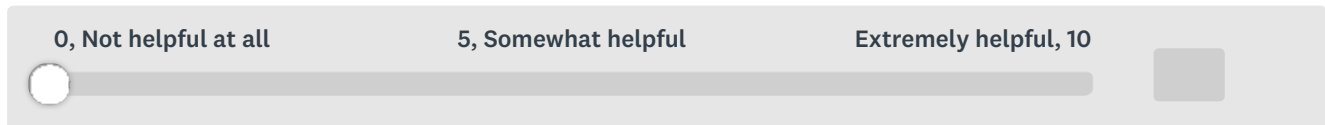A horizontal slider bar with a white circular knob at the 0 position. The bar is light gray with a darker gray track. The text "0, Not helpful at all" is at the left end, "5, Somewhat helpful" is in the middle, and "Extremely helpful, 10" is at the right end.☐

58. Did you notice the color map differences on different MRI modalities? How helpful is this feature in clinical settings?

0, Not helpful at all                      5, Somewhat helpful                      Extremely helpful, 10

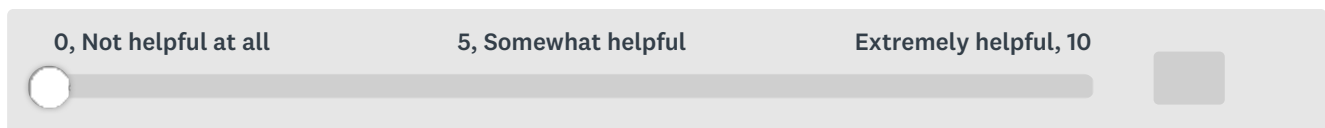A horizontal slider bar with a white circular knob at the 0 position. The bar is light gray with a darker gray track. The text "0, Not helpful at all" is at the left end, "5, Somewhat helpful" is in the middle, and "Extremely helpful, 10" is at the right end.☐

59.

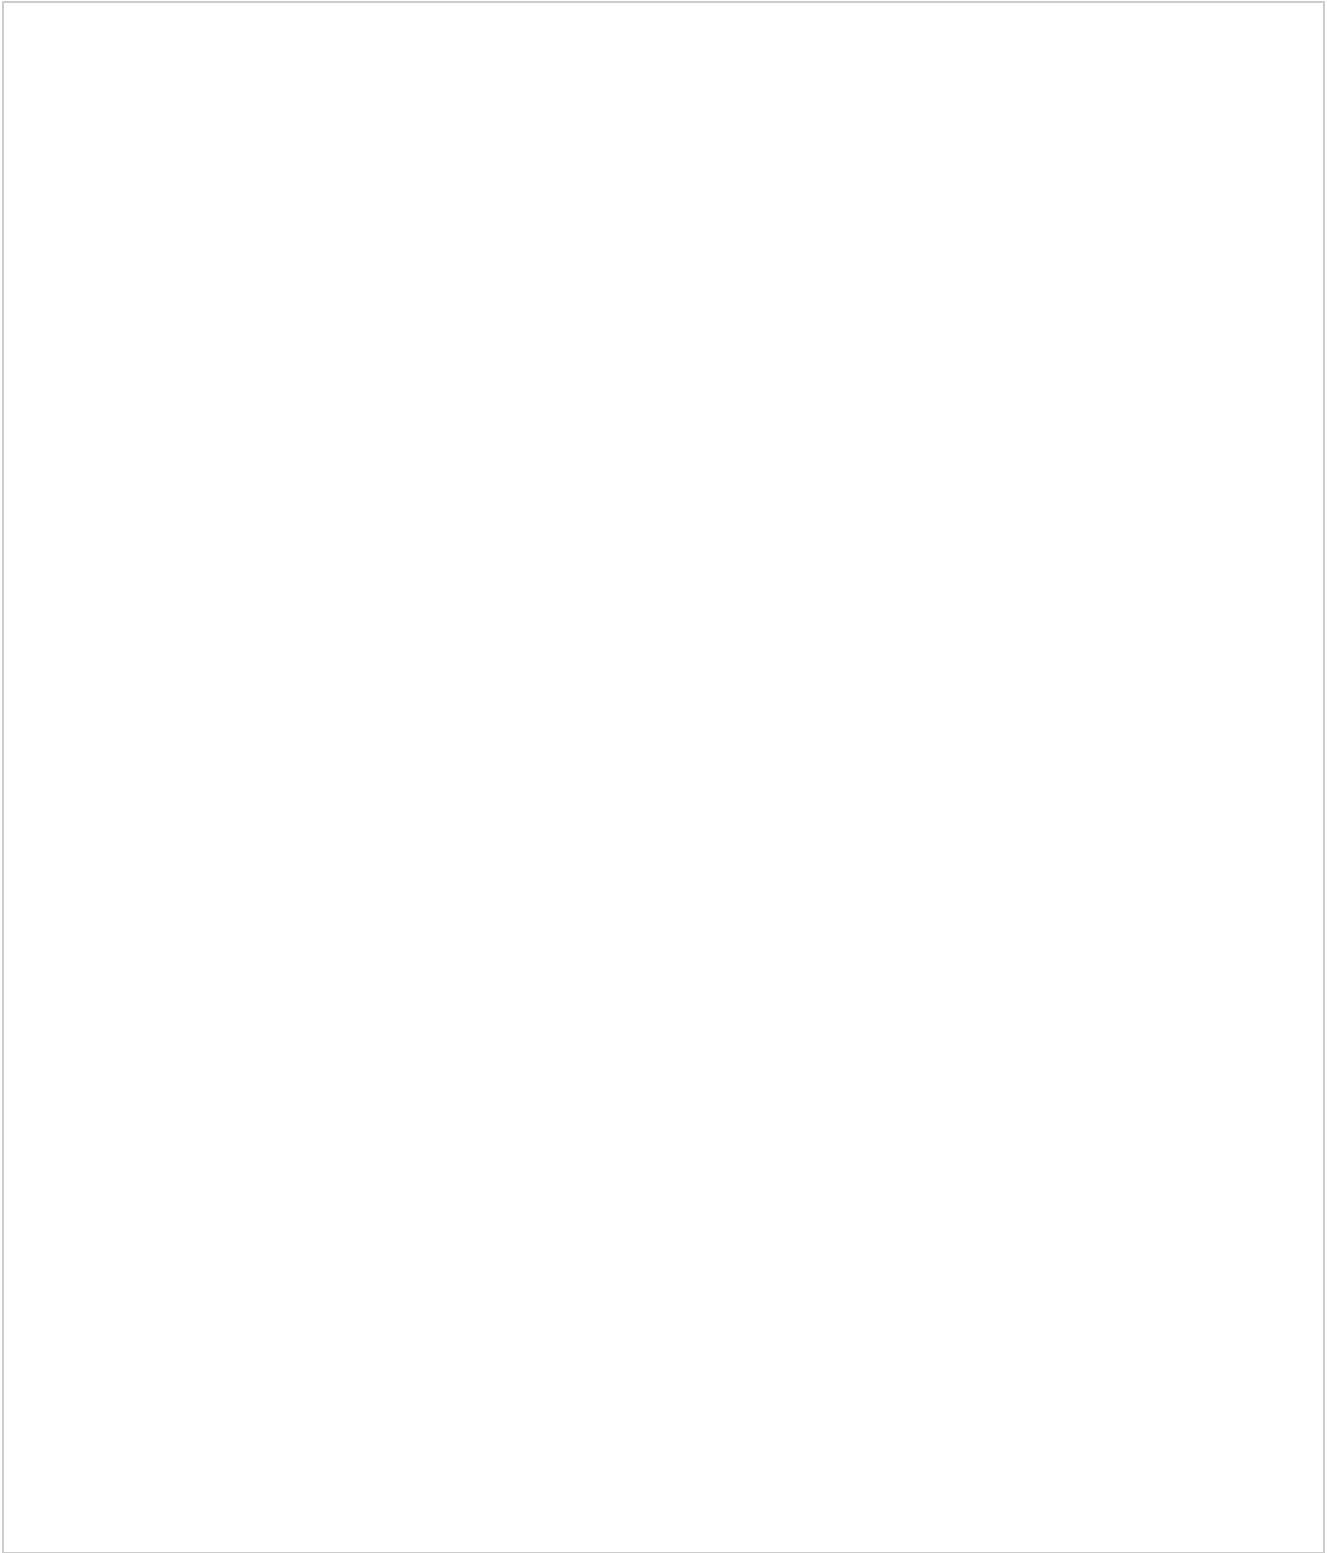

Please provide any of your comments on this color map.



60. How many percentages do the highlighted area match with your clinical judgment on the important features to classify LGG/HGG?

0%, Not matches at all                      50%                      Completely matches with mine, 100%

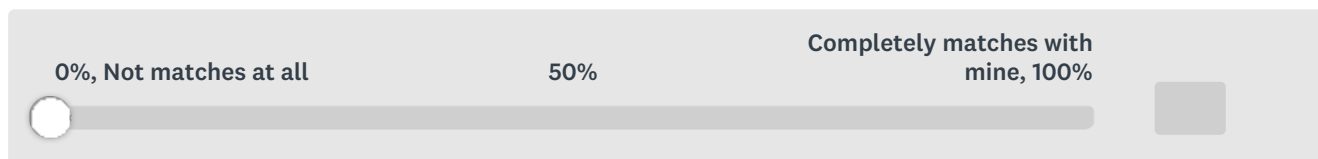A horizontal slider bar with a white circular knob at the 0% position. The bar is light gray with a darker gray track. The text "0%, Not matches at all" is on the left, "50%" is in the middle, and "Completely matches with mine, 100%" is on the right. A small gray square button is at the far right.

61. How helpful is this color map in clinical settings?

0, Not helpful at all                      5, Somewhat helpful                      Extremely helpful, 10

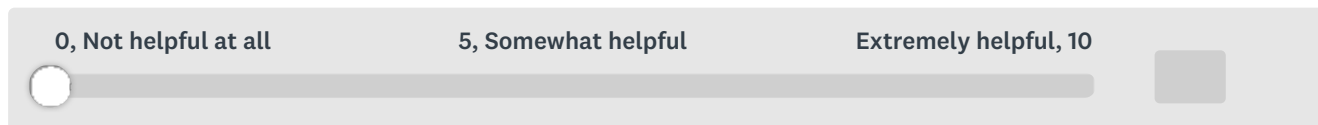A horizontal slider bar with a white circular knob at the 0 position. The bar is light gray with a darker gray track. The text "0, Not helpful at all" is on the left, "5, Somewhat helpful" is in the middle, and "Extremely helpful, 10" is on the right. A small gray square button is at the far right.

62. Did you notice the color map differences on different MRI modalities? How helpful is this feature in clinical settings?

0, Not helpful at all                      5, Somewhat helpful                      Extremely helpful, 10

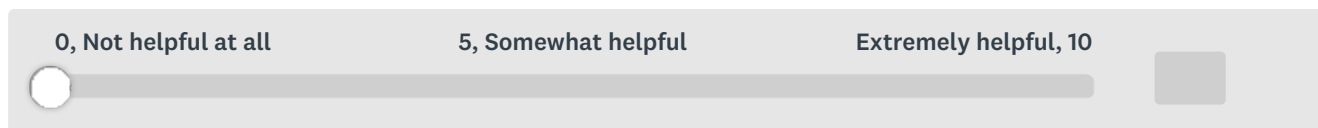A horizontal slider bar with a white circular knob at the 0 position. The bar is light gray with a darker gray track. The text "0, Not helpful at all" is on the left, "5, Somewhat helpful" is in the middle, and "Extremely helpful, 10" is on the right. A small gray square button is at the far right.

63.

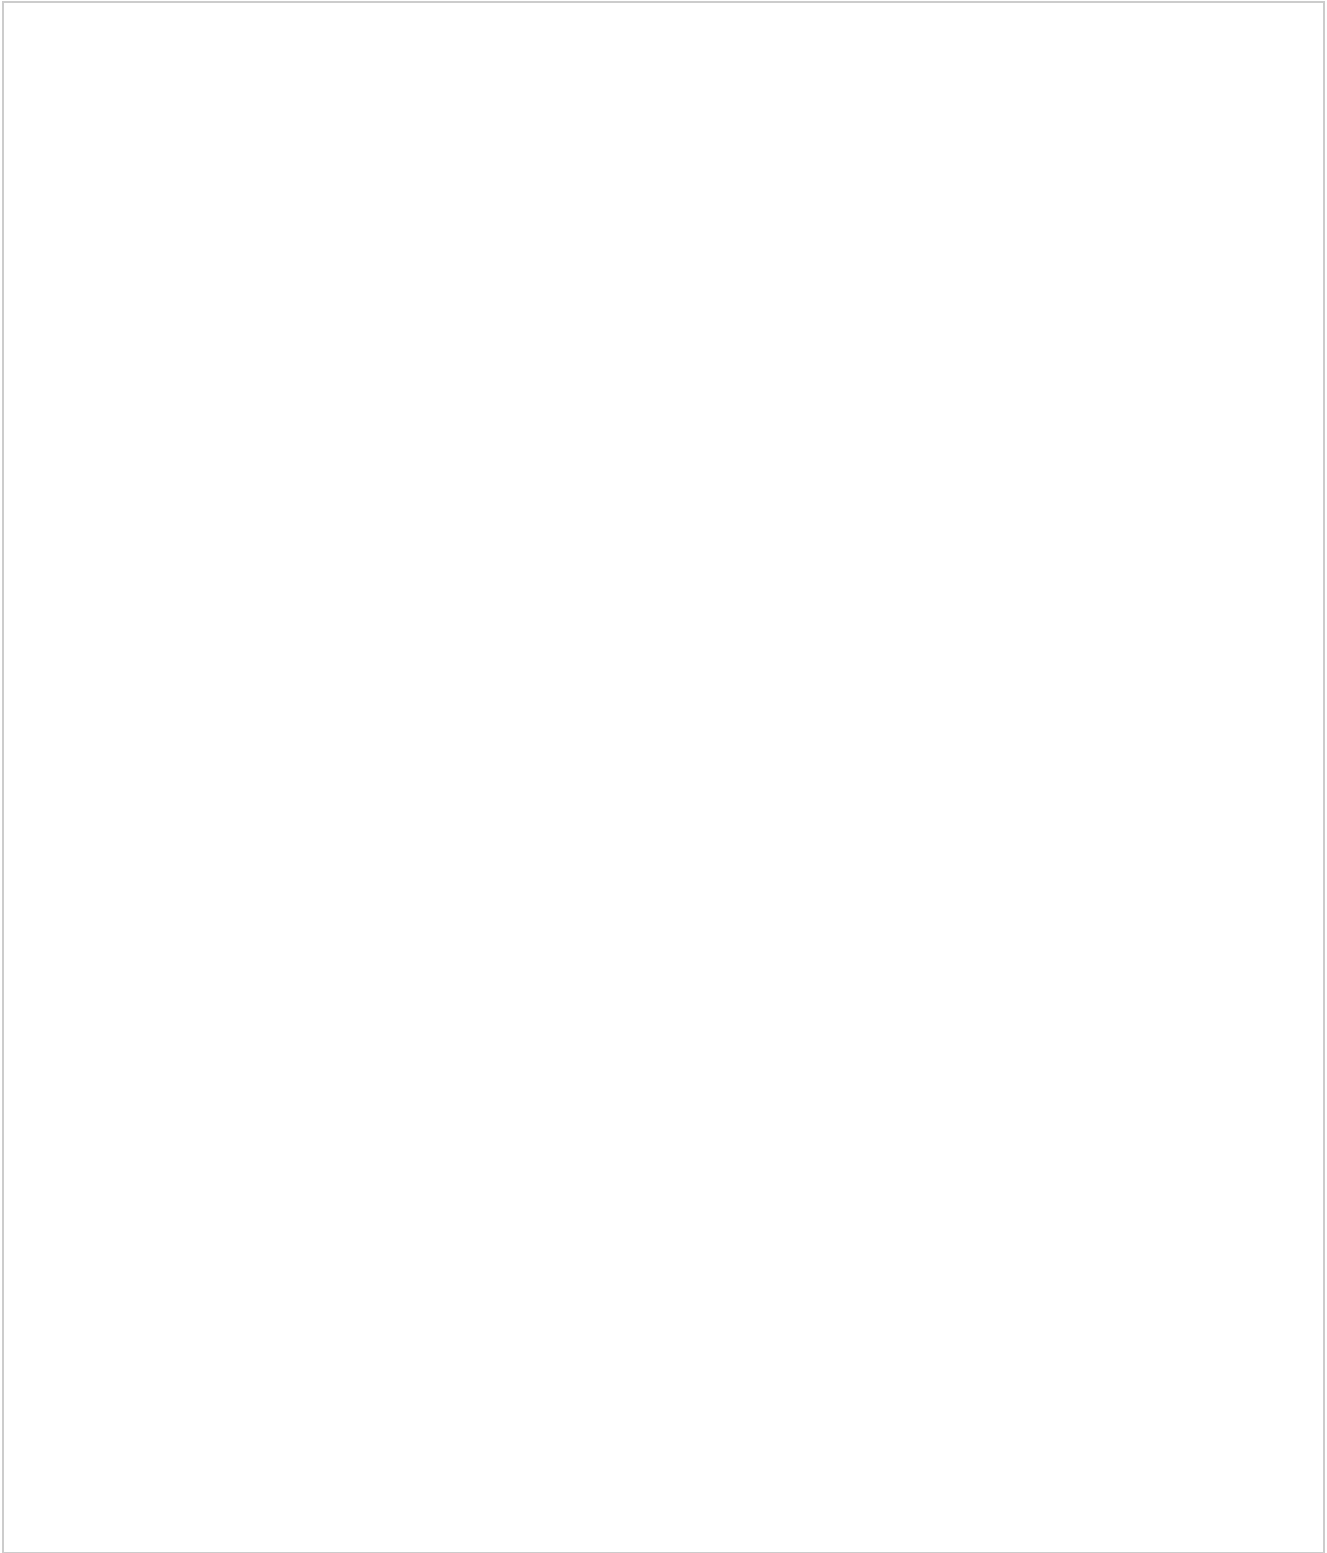

Please provide any of your comments on this color map.

64. How many percentages do the highlighted area match with your clinical judgment on the important features to classify LGG/HGG?

0%, Not matches at all                      50%                      Completely matches with mine, 100%

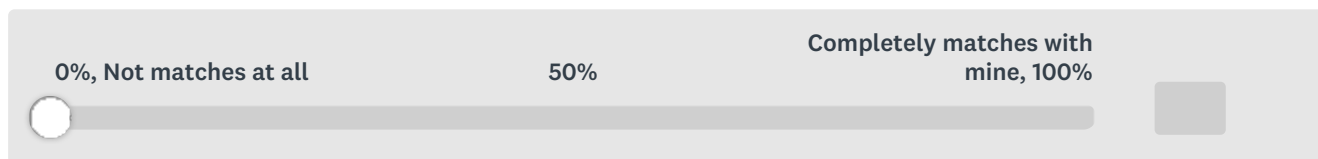A horizontal slider bar with a white circular knob at the 0% position. The bar is light gray and has a darker gray track. A small gray square button is located at the right end of the slider.

65. How helpful is this color map in clinical settings?

0, Not helpful at all                      5, Somewhat helpful                      Extremely helpful, 10

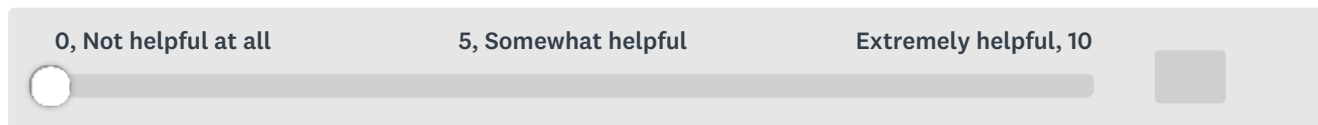A horizontal slider bar with a white circular knob at the 0 position. The bar is light gray and has a darker gray track. A small gray square button is located at the right end of the slider.

66. Did you notice the color map differences on different MRI modalities? How helpful is this feature in clinical settings?

0, Not helpful at all                      5, Somewhat helpful                      Extremely helpful, 10

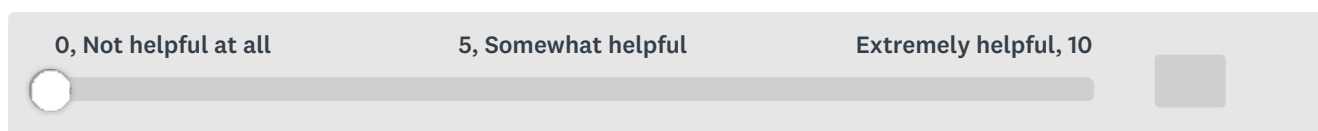A horizontal slider bar with a white circular knob at the 0 position. The bar is light gray and has a darker gray track. A small gray square button is located at the right end of the slider.

67.

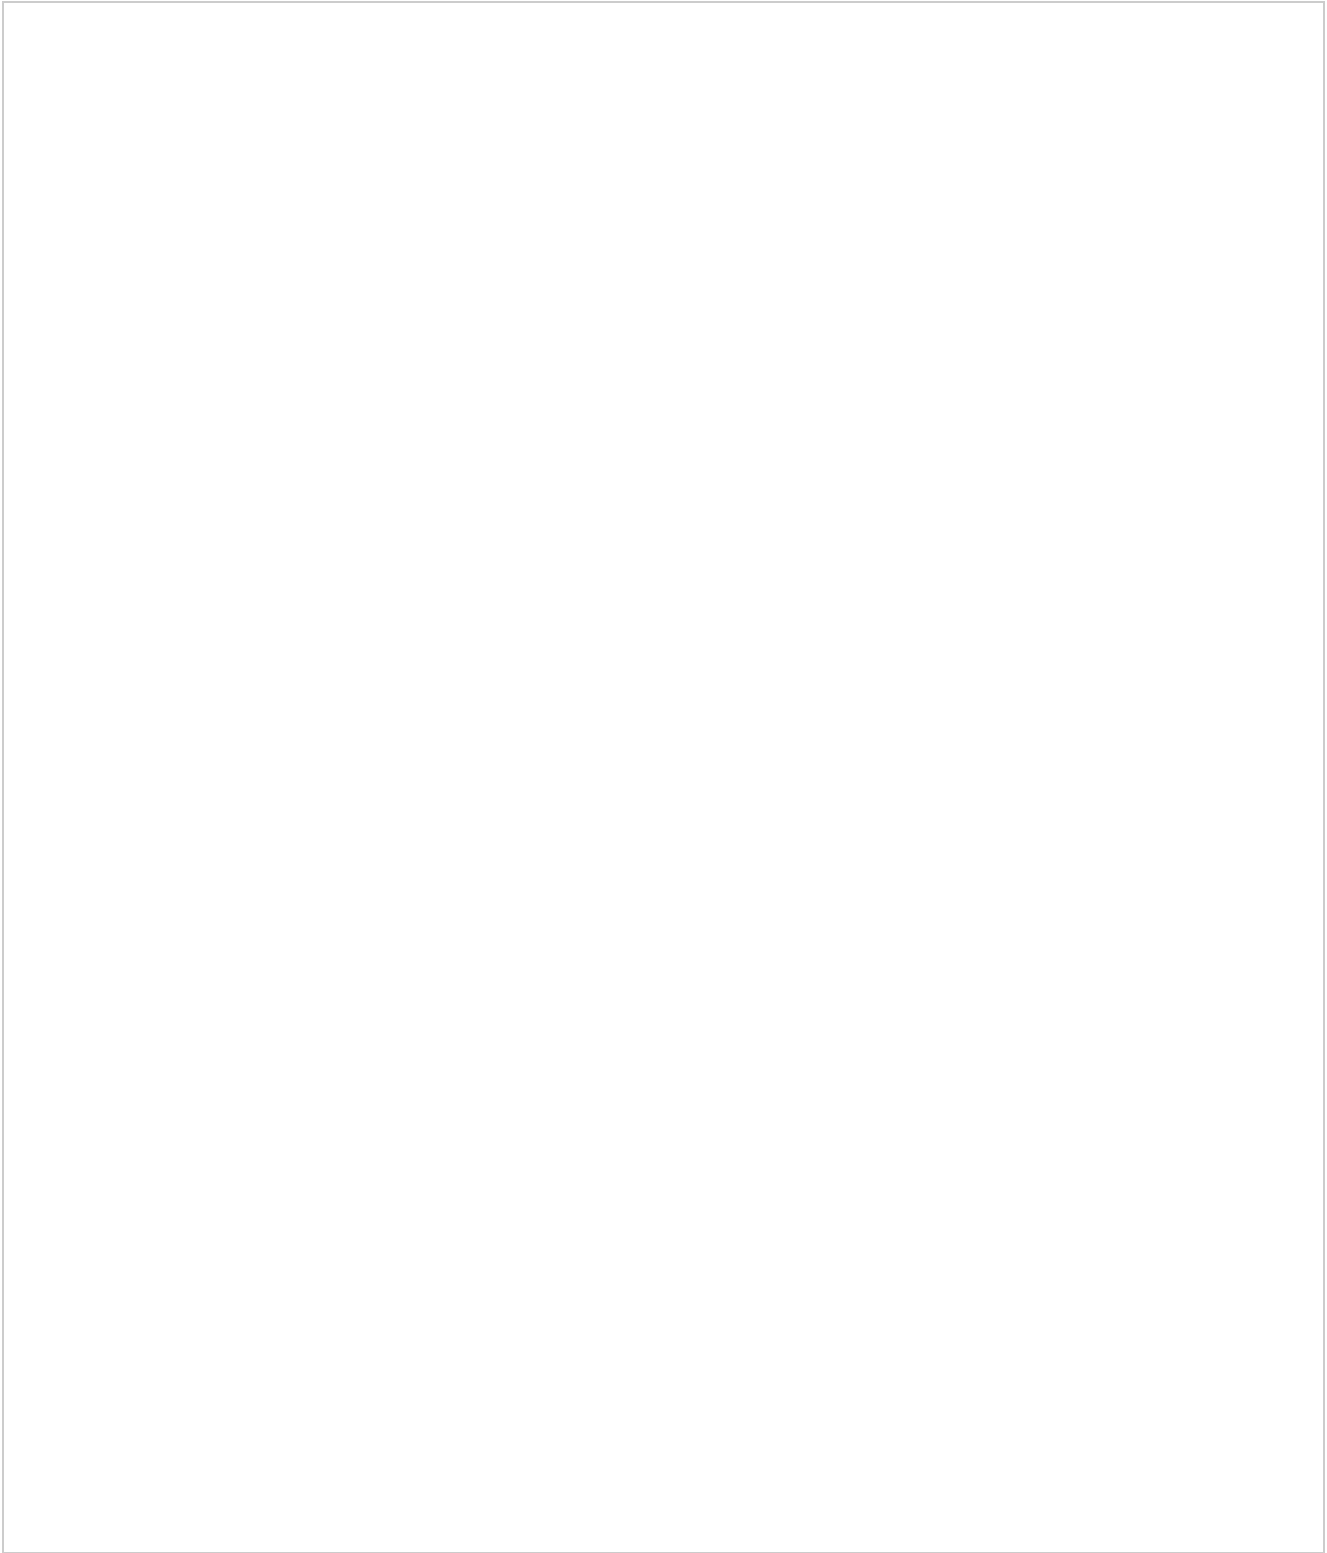

Please provide any of your comments on this color map.

68. How many percentages do the highlighted area match with your clinical judgment on the important features to classify LGG/HGG?

0%, Not matches at all                      50%                      Completely matches with mine, 100%

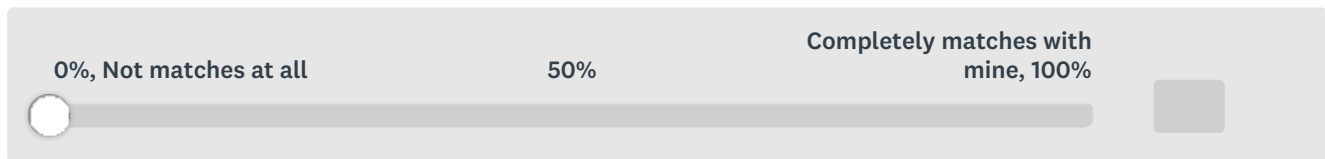

A horizontal slider bar with a white circular knob at the 0% position. The bar is light gray and spans the width of the question area.

☐

69. How helpful is this color map in clinical settings?

0, Not helpful at all                      5, Somewhat helpful                      Extremely helpful, 10

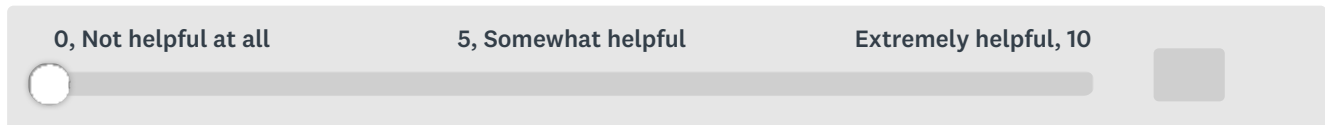

A horizontal slider bar with a white circular knob at the 0 position. The bar is light gray and spans the width of the question area.

☐

70. Did you notice the **color map differences** on **different MRI modalities**? How helpful is this feature in clinical settings?

0, Not helpful at all                      5, Somewhat helpful                      Extremely helpful, 10

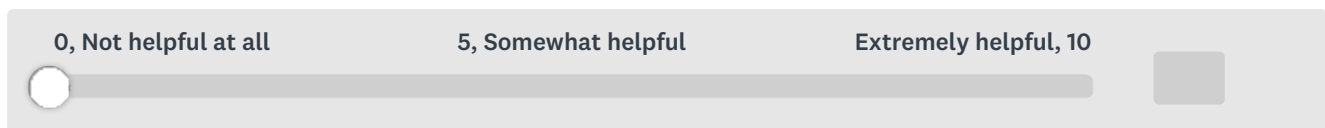

A horizontal slider bar with a white circular knob at the 0 position. The bar is light gray and spans the width of the question area.

☐

**71.**

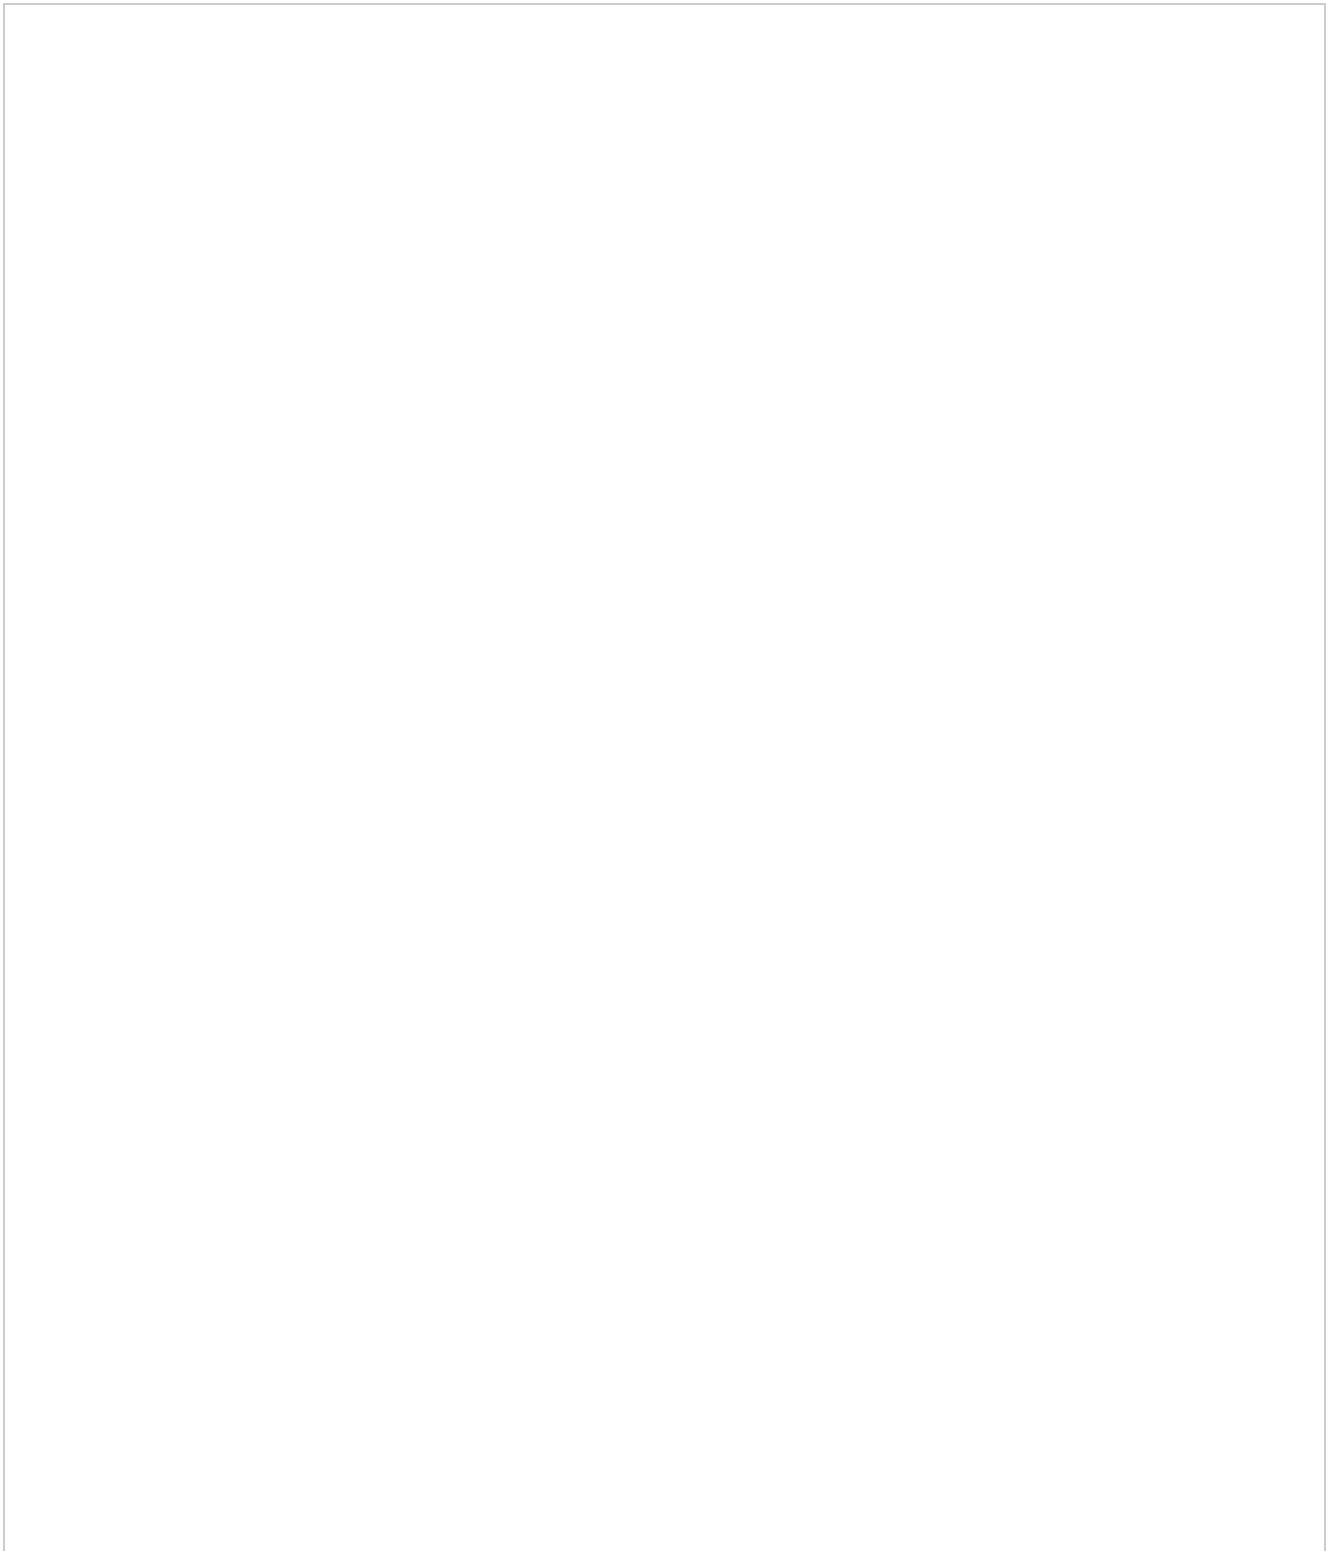

**Please provide any of your comments on this color map.**

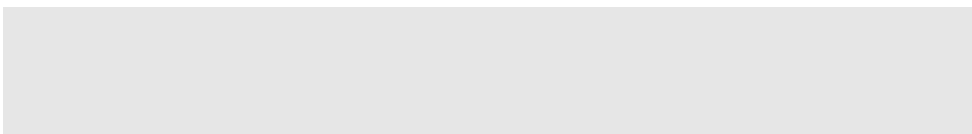

72. How many percentages do the highlighted area match with your clinical judgment on the important features to classify LGG/HGG?

0%, Not matches at all                      50%                      Completely matches with mine, 100%

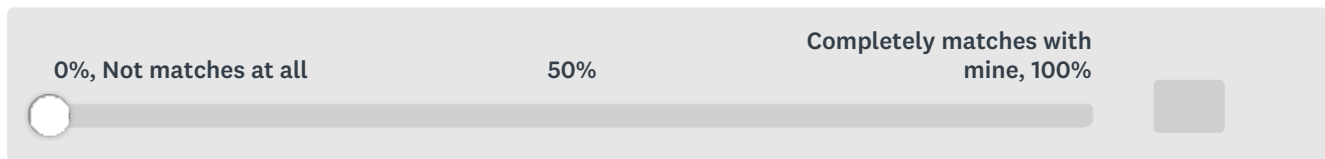

73. How helpful is this color map in clinical settings?

0, Not helpful at all                      5, Somewhat helpful                      Extremely helpful, 10

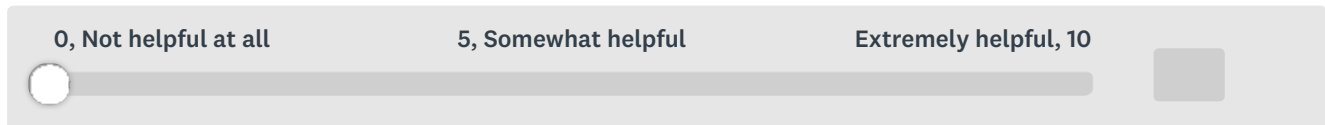

74. Did you notice the color map differences on different MRI modalities? How helpful is this feature in clinical settings?

0, Not helpful at all                      5, Somewhat helpful                      Extremely helpful, 10

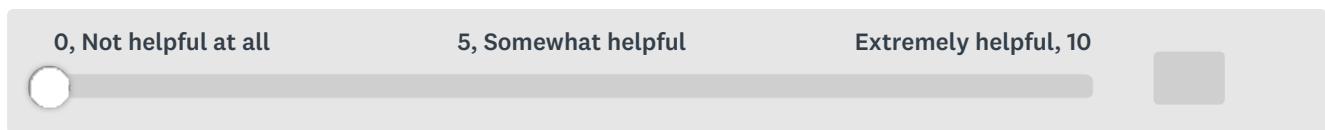

75. Suppose you have just reviewed the AI prediction and the **best** color map explanation, what is your trust level in this AI?

-5, Totally distrust the AI                      0, Neutral, neither distrust nor trust                      Totally trust the AI, 5

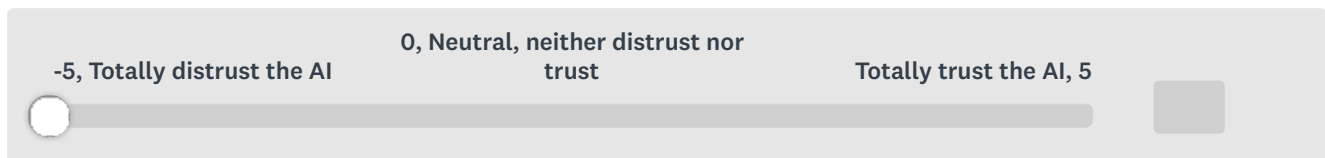

76. Suppose you have just reviewed the AI prediction and the **best** color map explanation, how likely will you incorporate this AI's suggestions into your clinical practice?

Consider the likelihood that you are willing to let this AI assist you (in ways such as: it may reinforce your confidence about a decision; or it may alert you to potential mistakes, etc.), and consider its suggestions to your patient's management plan.

0, Not likely                      5, Somewhat likely                      Very likely, 10

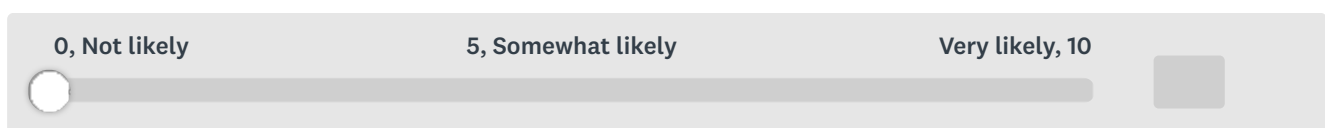

## Welcome to the Medical AI study

### MRI for Patient 2

\* 77. Now you have another new patient MRI, and this AI is available for you to use, to assist your judgment on tumor grade.

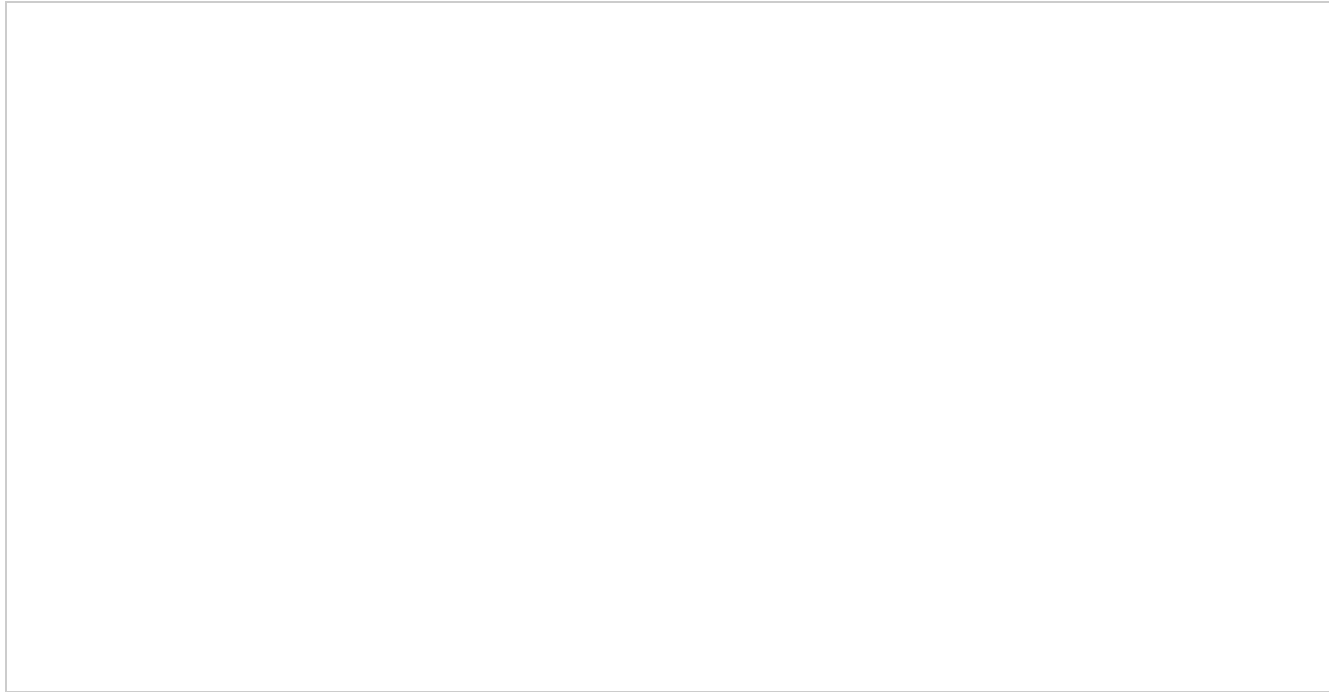

First, would you mind providing your judgment on this patient's MRI?

- ☐ Low-grade gliomas (LGG)
- ☐ High-grade gliomas (HGG)
- ☐ Other, please specify.

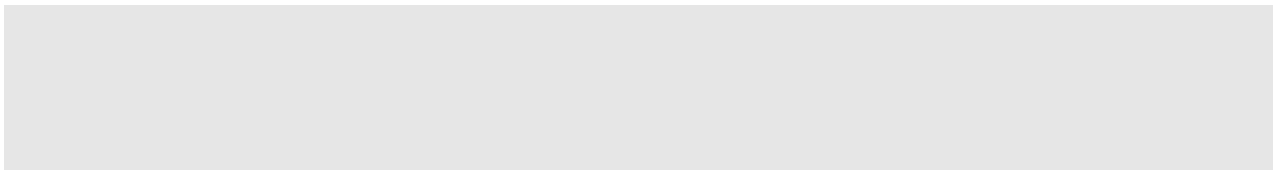



78. How confident are you in making this judgment?

0, Not confident at all      5, Somewhat confident      Completely confident, 10

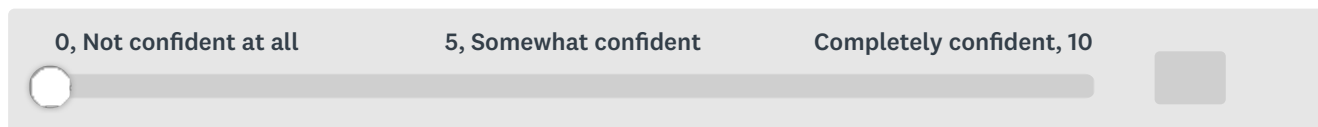

## Welcome to the Medical AI study

MRI for Patient 2

\* 79. AI predicts this is **low-grade gliomas**. What are your thoughts about AI's prediction?

- ☐ I am **OK with the prediction from AI**. I would like to check more detailed information from AI, to see how it reaches this prediction .
- ☐ I am **not comfortable with the prediction from AI** . I would like to check more detailed information from AI, to see how it reaches this prediction .
- ☐ I am **OK with the prediction from AI**. I have other priorities, and **won't check more detailed information from AI**.
- ☐ I am **not comfortable with the prediction from AI** . But I have other priorities, and **won't check more detailed information from AI**.

80. After viewing this AI's prediction on the new patient, what is your trust level in this AI?

-5, Totally distrust the AI

0, Neutral, neither distrust nor trust

Totally trust the AI, 5

81. After viewing this AI's prediction on the new patient, how likely will you incorporate this AI's suggestions into your clinical practice?

Consider the likelihood that you are willing to let this AI assist you (in ways such as: it may reinforce your confidence about a decision; or it may alert you to potential mistakes, etc.), and consider its suggestions to your patient's management plan.

0, Not likely                      5, Somewhat likely                      Very likely, 10

## Welcome to the Medical AI study

### Color Map Explanation for Patient 2

The AI could explain its decisions using color maps. The color maps indicate important brain regions for the AI's prediction.

Next, we would like to invite you to review the following 16 color maps. They all try to explain the same AI model that predicts **low-grade gliomas**, for the same patient MRI.

Row 1: the original MRI you just read

Row 2: the color map only

Row 3: the color map overlaid on the MRI

82.

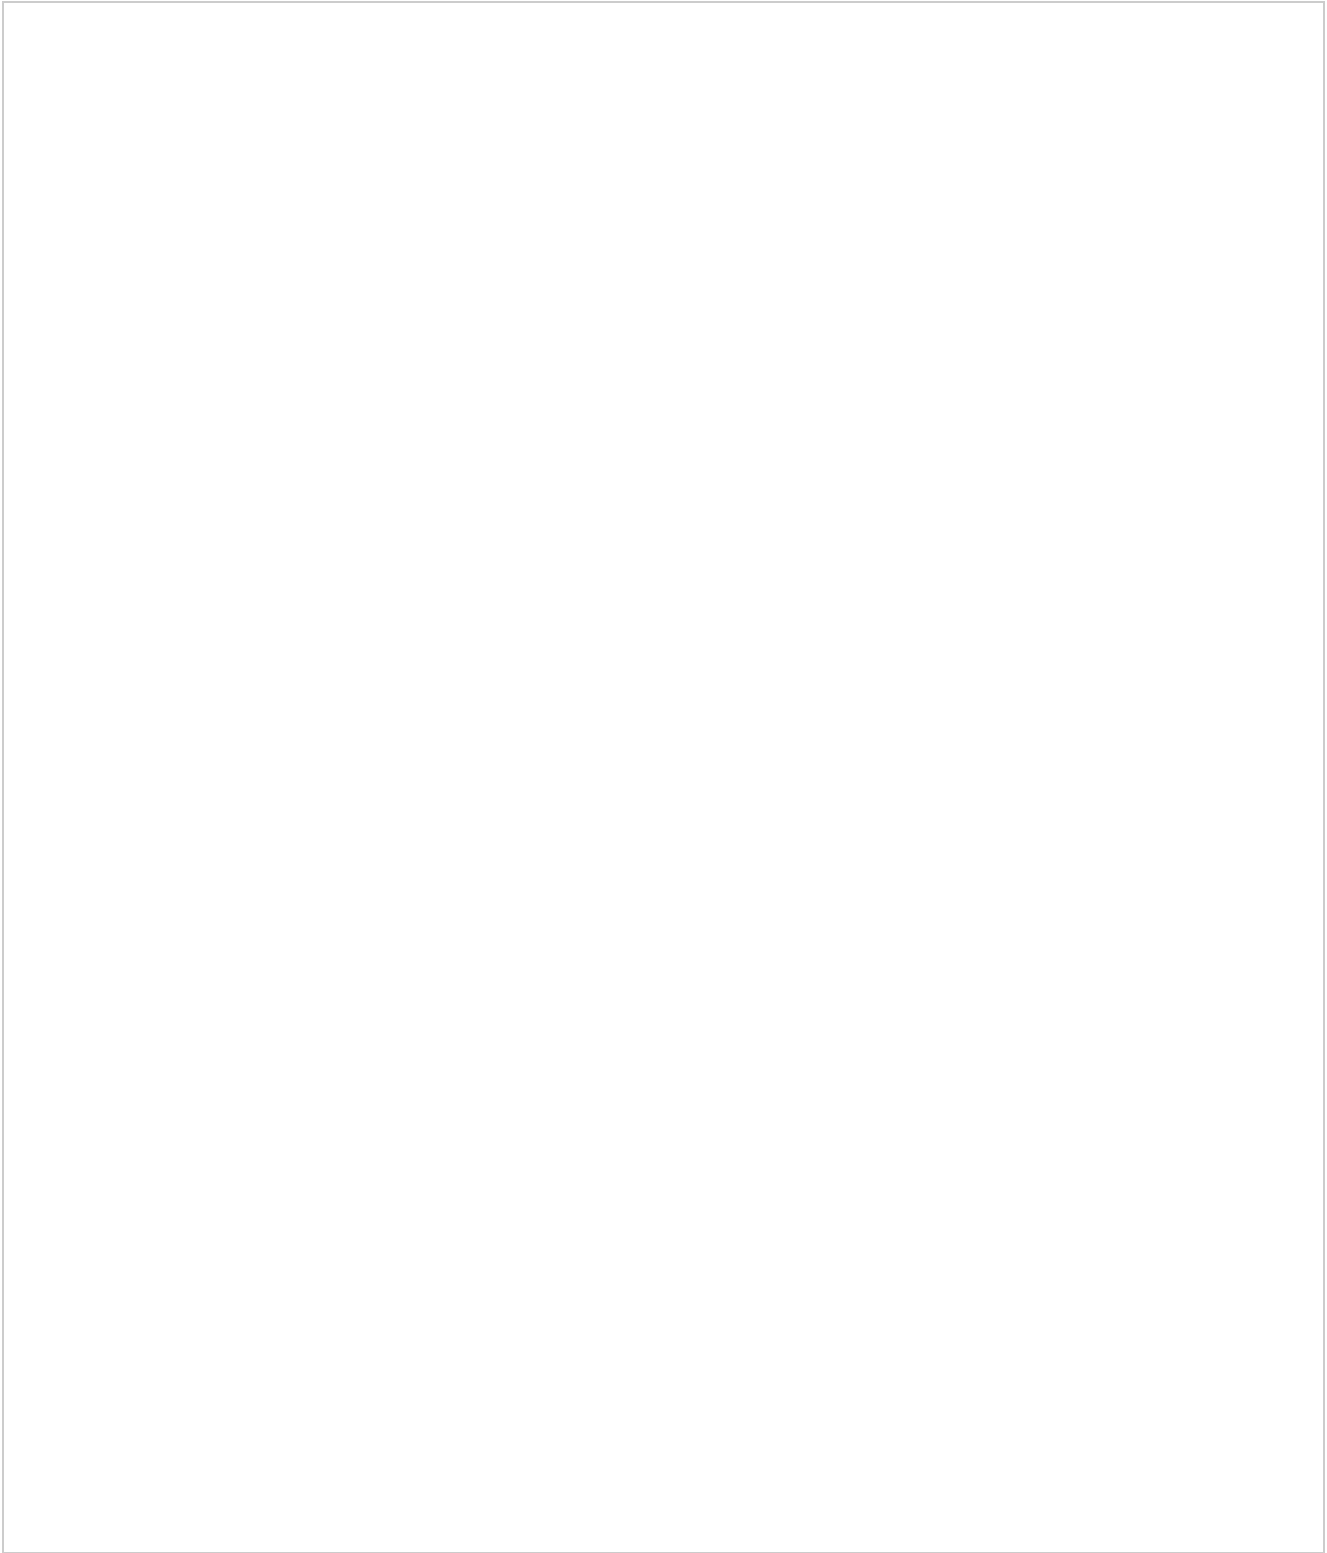

Please provide any of your comments on this color map.

83. How many percentages do the highlighted area match with your clinical judgment on the important features to classify LGG/HGG?

0%, Not matches at all                      50%                      Completely matches with mine, 100%

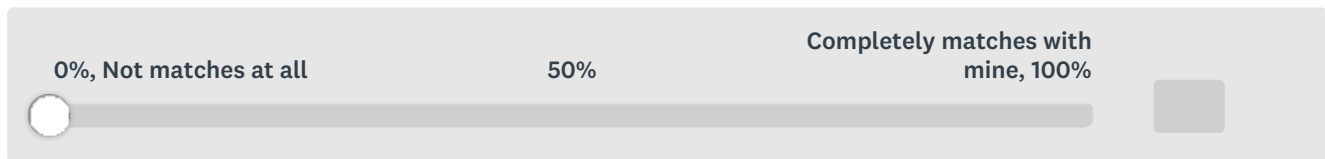A horizontal slider bar with a white circular knob at the 0% position. The bar is light gray with a darker gray track. The text "0%, Not matches at all" is on the left, "50%" is in the middle, and "Completely matches with mine, 100%" is on the right. A small gray square button is at the far right.

84. How helpful is this color map in clinical settings?

0, Not helpful at all                      5, Somewhat helpful                      Extremely helpful, 10

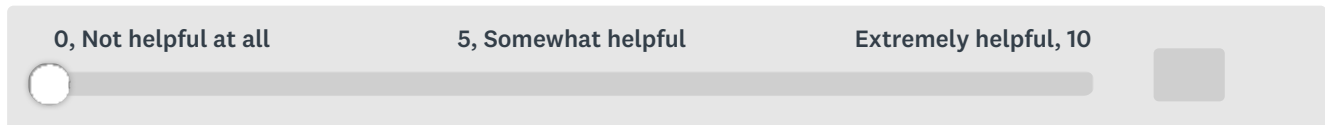A horizontal slider bar with a white circular knob at the 0 position. The bar is light gray with a darker gray track. The text "0, Not helpful at all" is on the left, "5, Somewhat helpful" is in the middle, and "Extremely helpful, 10" is on the right. A small gray square button is at the far right.

85. Did you notice the color map differences on different MRI modalities? How helpful is this feature in clinical settings?

0, Not helpful at all                      5, Somewhat helpful                      Extremely helpful, 10

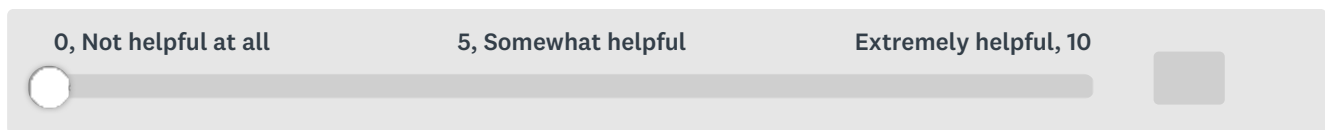A horizontal slider bar with a white circular knob at the 0 position. The bar is light gray with a darker gray track. The text "0, Not helpful at all" is on the left, "5, Somewhat helpful" is in the middle, and "Extremely helpful, 10" is on the right. A small gray square button is at the far right.

86.

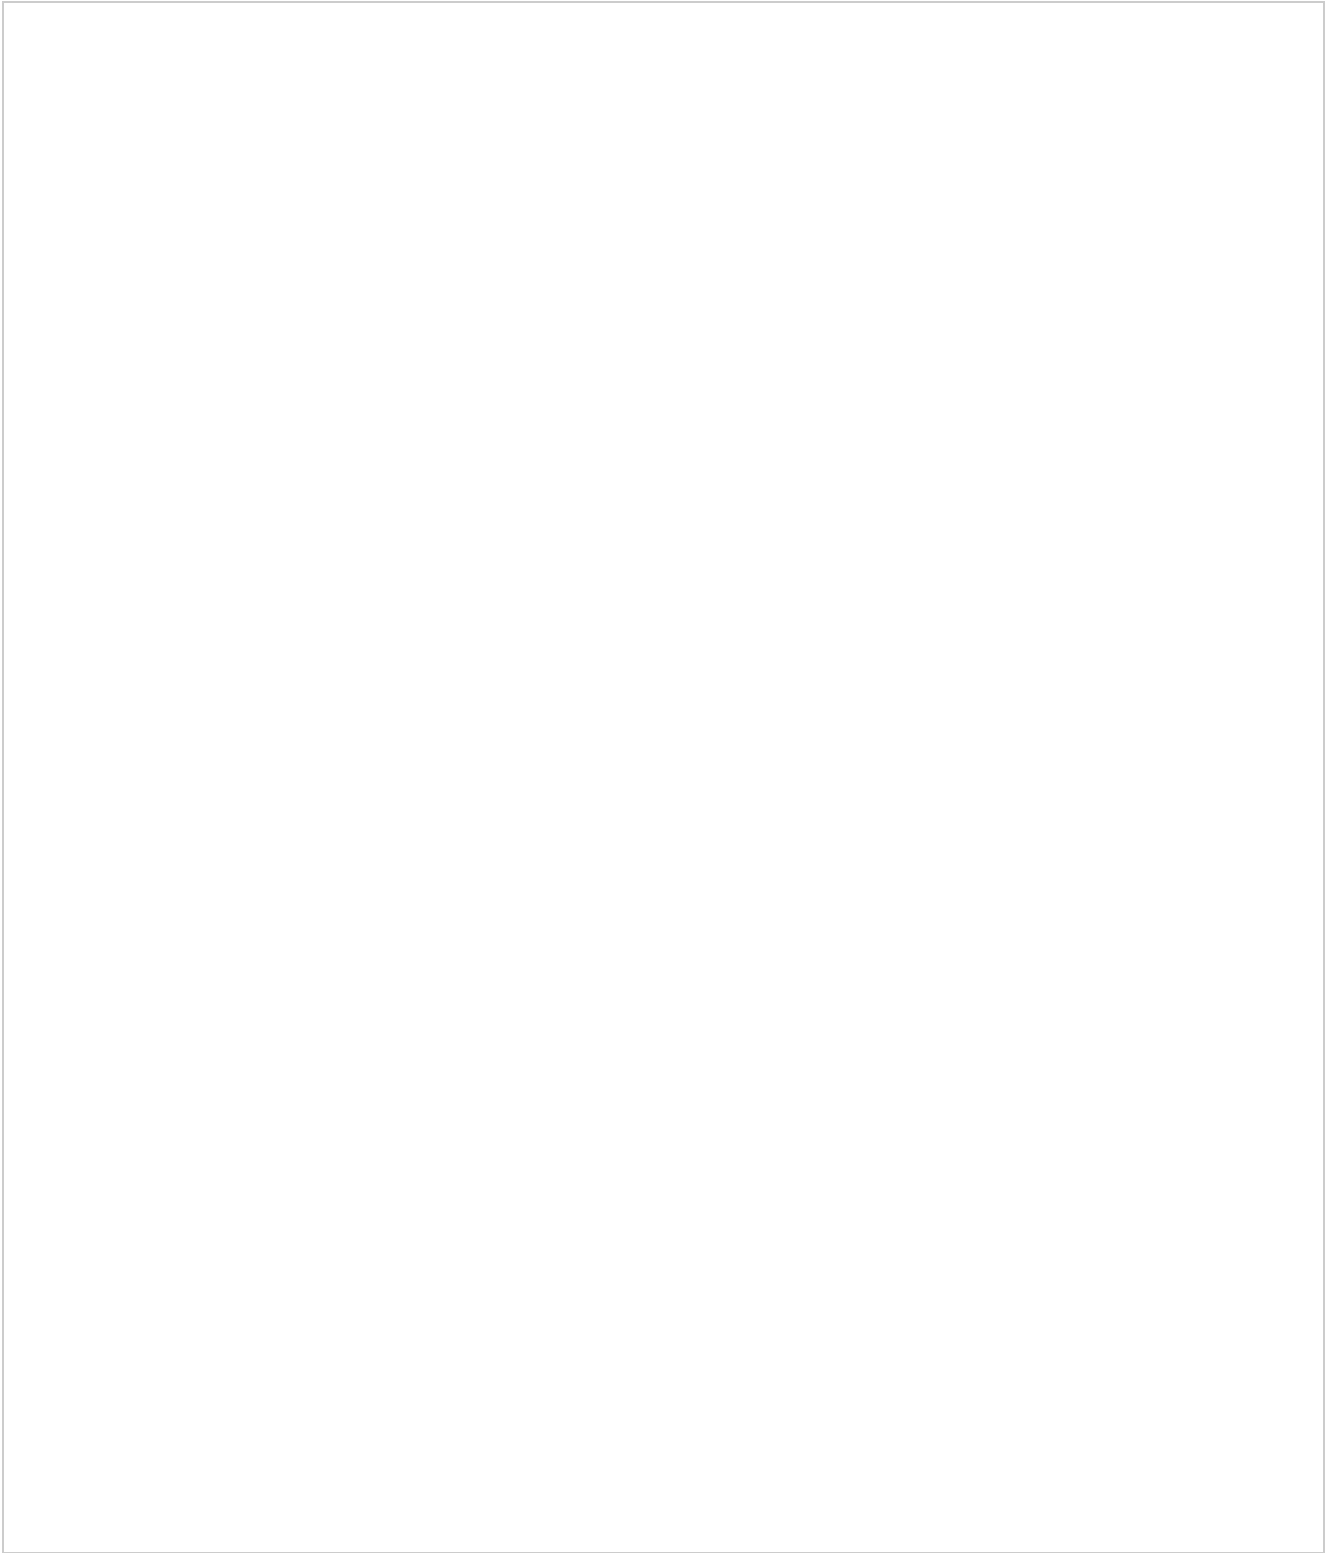

Please provide any of your comments on this color map.

87. How many percentages do the highlighted area match with your clinical judgment on the important features to classify LGG/HGG?

0%, Not matches at all                      50%                      Completely matches with mine, 100%

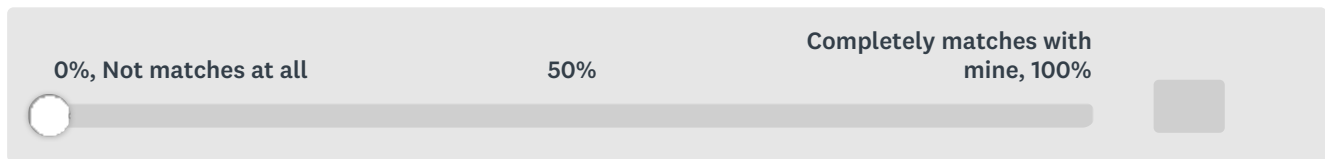A horizontal slider bar with a white circular knob at the 0% position. The bar is light gray with a darker gray track. The text "0%, Not matches at all" is on the left, "50%" is in the middle, and "Completely matches with mine, 100%" is on the right. A small gray square button is at the far right.

88. How helpful is this color map in clinical settings?

0, Not helpful at all                      5, Somewhat helpful                      Extremely helpful, 10

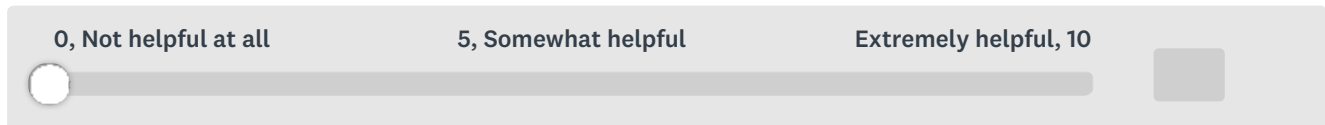A horizontal slider bar with a white circular knob at the 0 position. The bar is light gray with a darker gray track. The text "0, Not helpful at all" is on the left, "5, Somewhat helpful" is in the middle, and "Extremely helpful, 10" is on the right. A small gray square button is at the far right.

89. Did you notice the color map differences on different MRI modalities? How helpful is this feature in clinical settings?

0, Not helpful at all                      5, Somewhat helpful                      Extremely helpful, 10

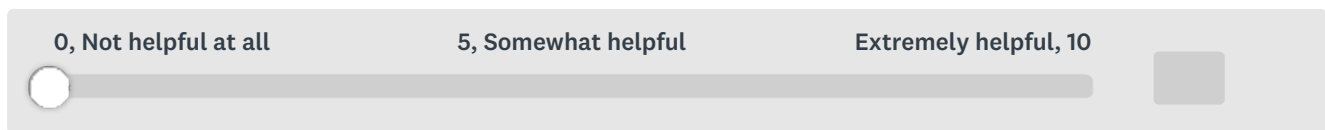A horizontal slider bar with a white circular knob at the 0 position. The bar is light gray with a darker gray track. The text "0, Not helpful at all" is on the left, "5, Somewhat helpful" is in the middle, and "Extremely helpful, 10" is on the right. A small gray square button is at the far right.

90.

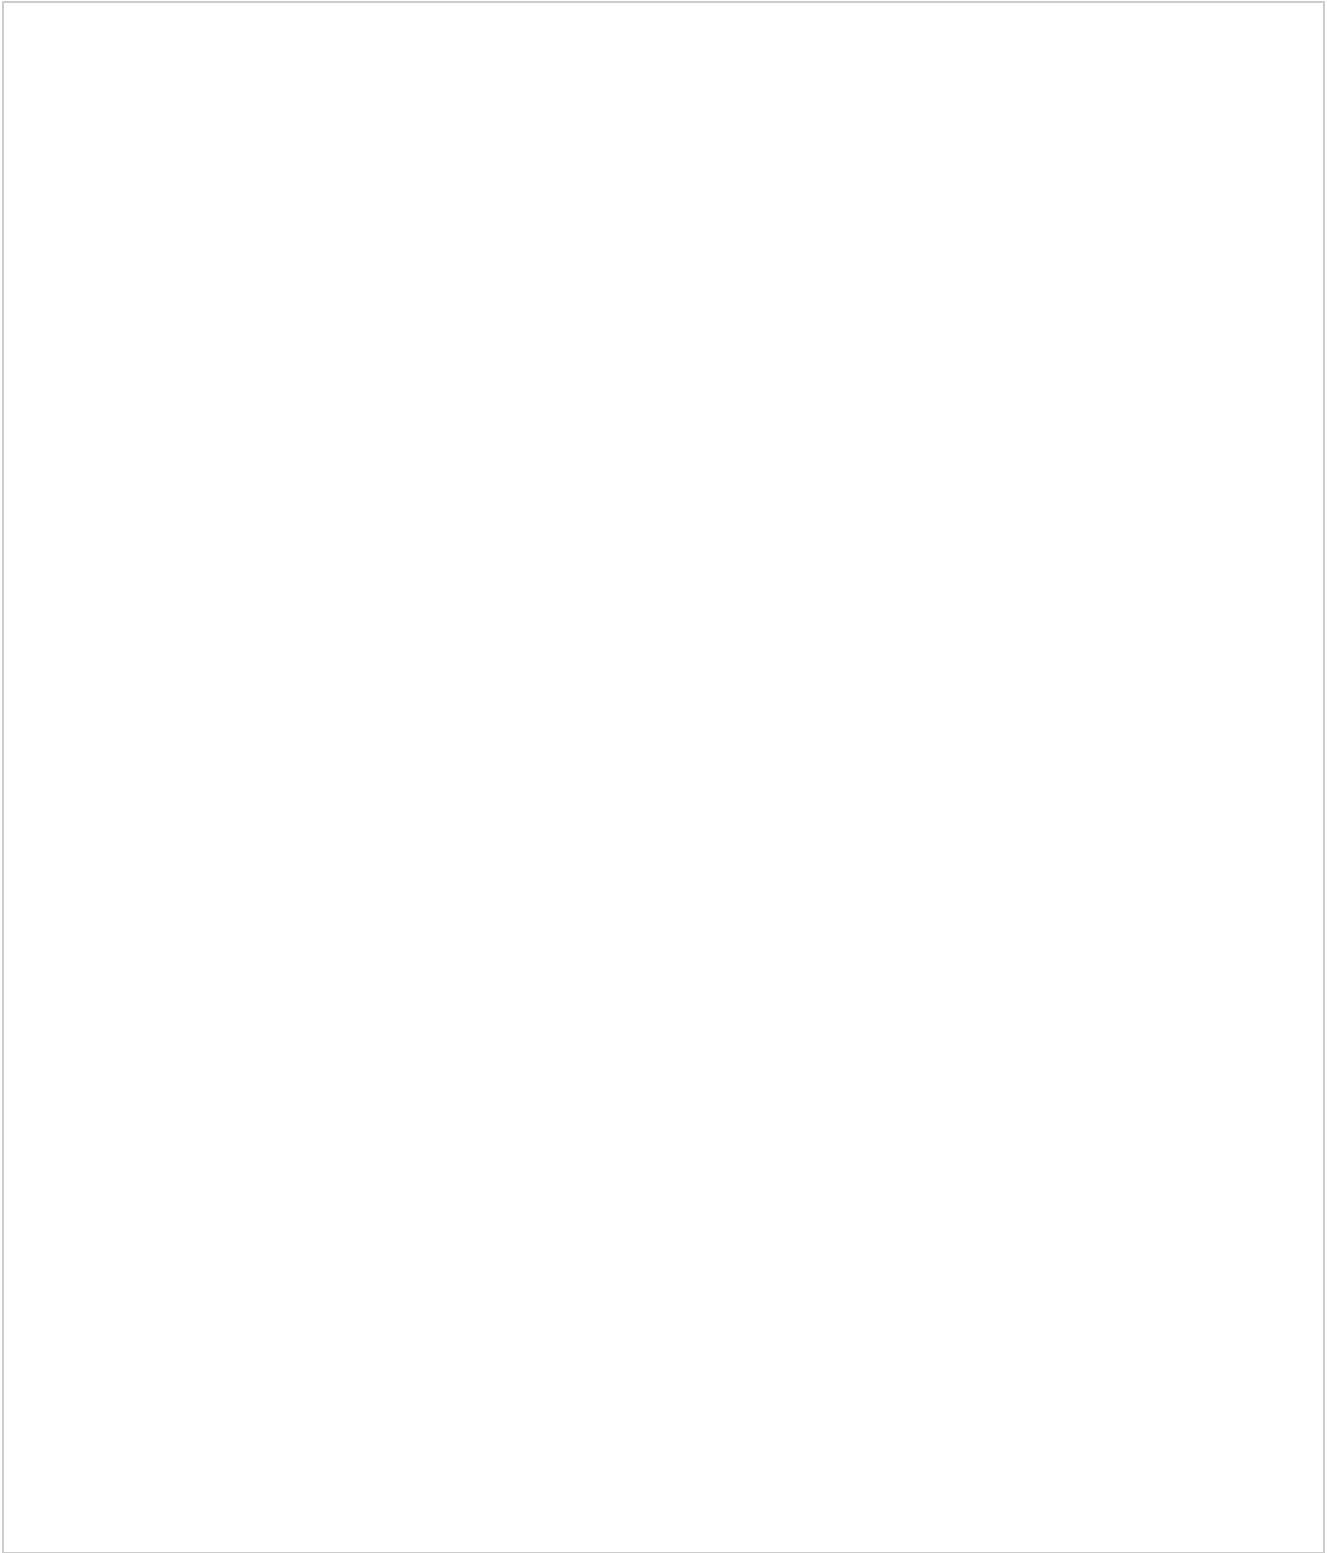

Please provide any of your comments on this color map.



91. How many percentages do the highlighted area match with your clinical judgment on the important features to classify LGG/HGG?

0%, Not matches at all                      50%                      Completely matches with mine, 100%

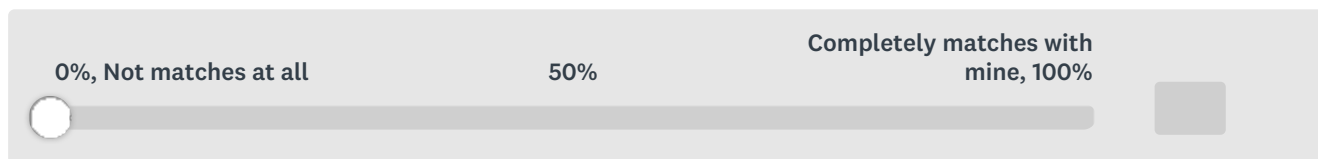A horizontal slider bar with a white circular knob at the 0% position. The bar is light gray with a darker gray track. The text "0%, Not matches at all" is at the left end, "50%" is in the middle, and "Completely matches with mine, 100%" is at the right end. A small gray square button is at the far right.

92. How helpful is this color map in clinical settings?

0, Not helpful at all                      5, Somewhat helpful                      Extremely helpful, 10

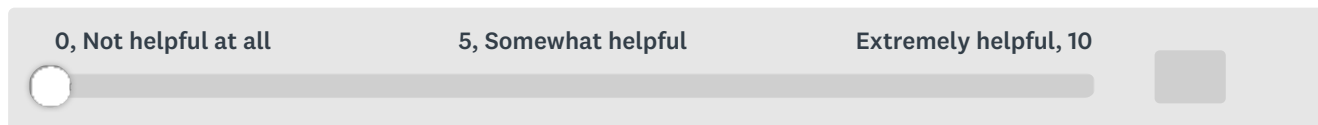A horizontal slider bar with a white circular knob at the 0 position. The bar is light gray with a darker gray track. The text "0, Not helpful at all" is at the left end, "5, Somewhat helpful" is in the middle, and "Extremely helpful, 10" is at the right end. A small gray square button is at the far right.

93. Did you notice the color map differences on different MRI modalities? How helpful is this feature in clinical settings?

0, Not helpful at all                      5, Somewhat helpful                      Extremely helpful, 10

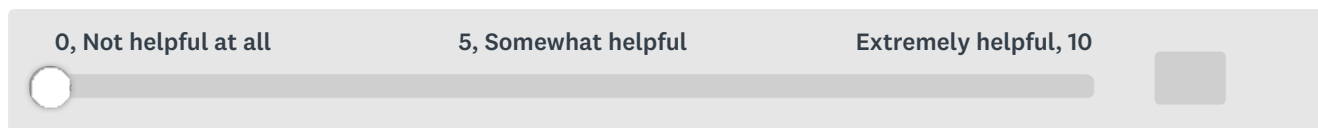A horizontal slider bar with a white circular knob at the 0 position. The bar is light gray with a darker gray track. The text "0, Not helpful at all" is at the left end, "5, Somewhat helpful" is in the middle, and "Extremely helpful, 10" is at the right end. A small gray square button is at the far right.

94.

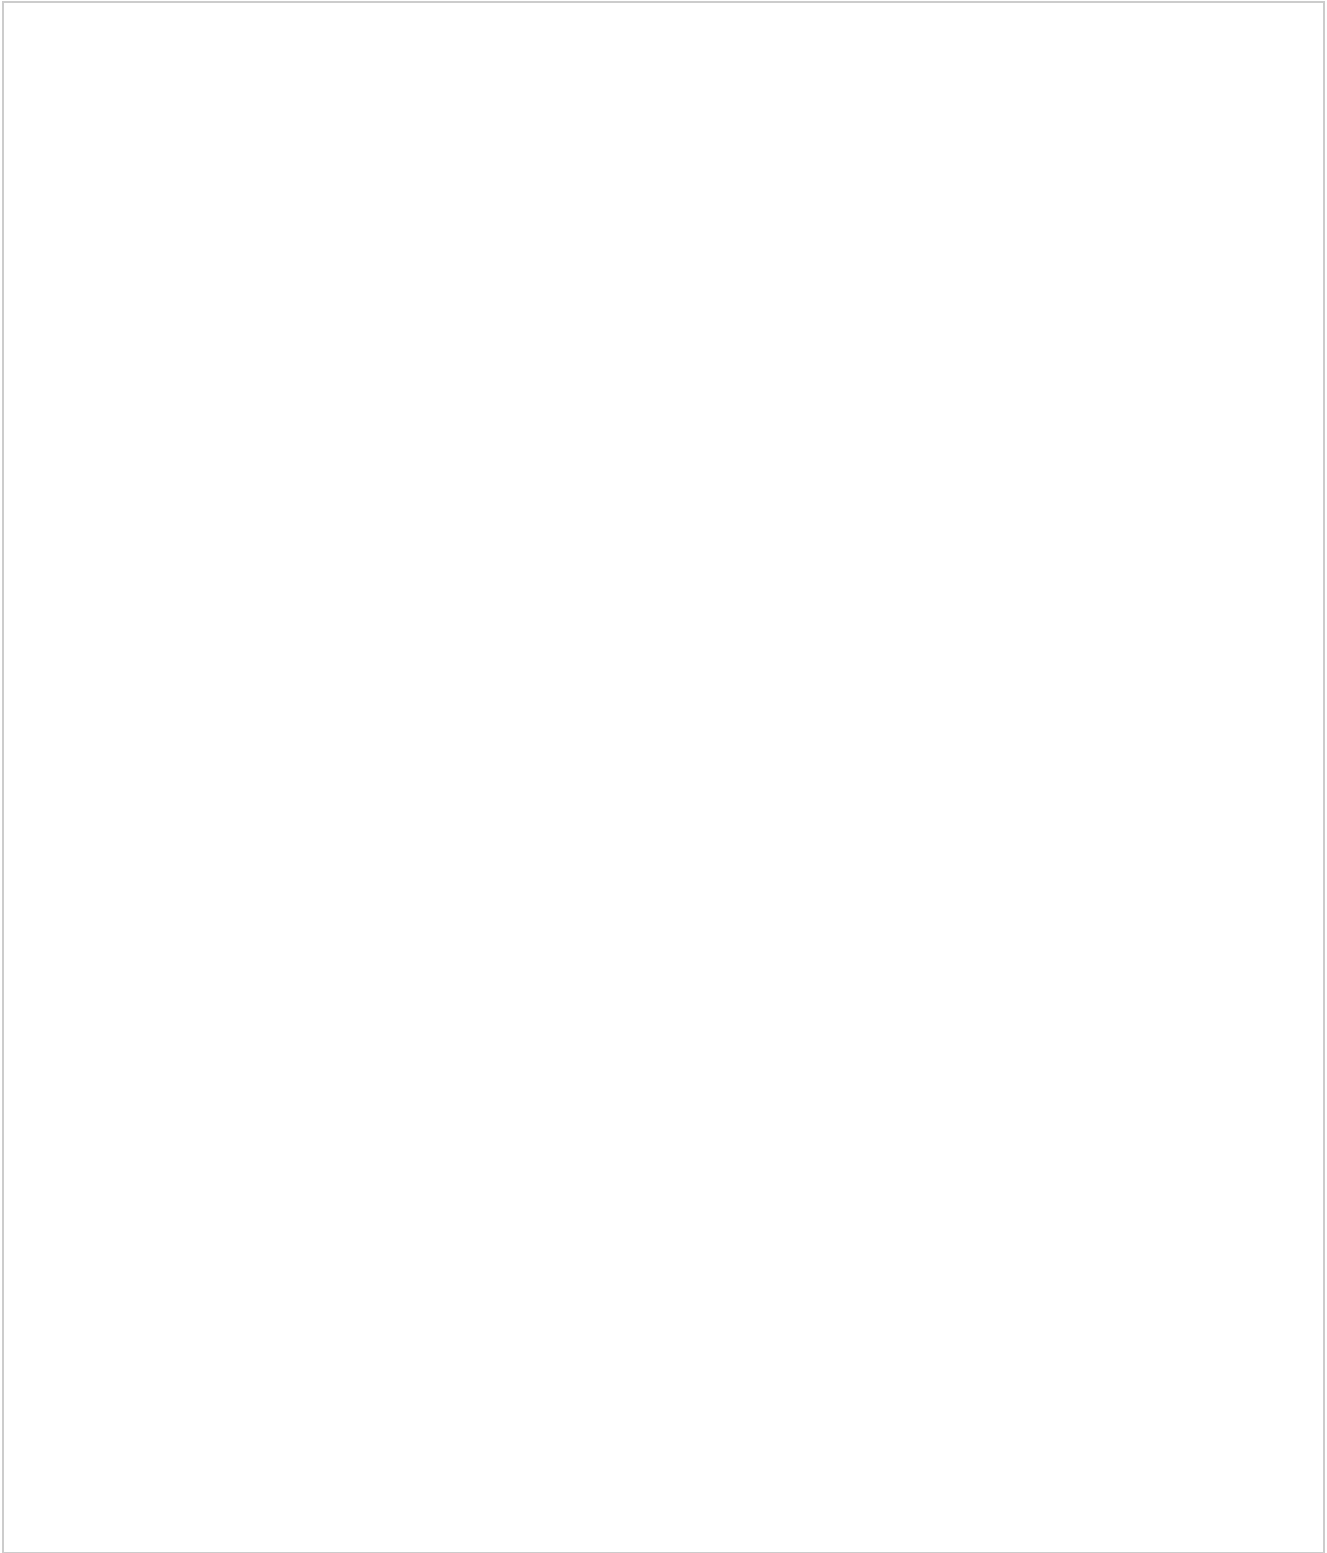

Please provide any of your comments on this color map.

95. How many percentages do the highlighted area match with your clinical judgment on the important features to classify LGG/HGG?

0%, Not matches at all                      50%                      Completely matches with mine, 100%

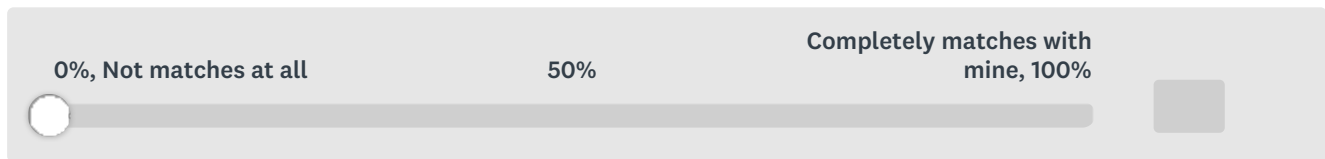A horizontal slider bar with a white circular knob at the 0% position. The bar is light gray and spans the width of the form.☐

96. How helpful is this color map in clinical settings?

0, Not helpful at all                      5, Somewhat helpful                      Extremely helpful, 10

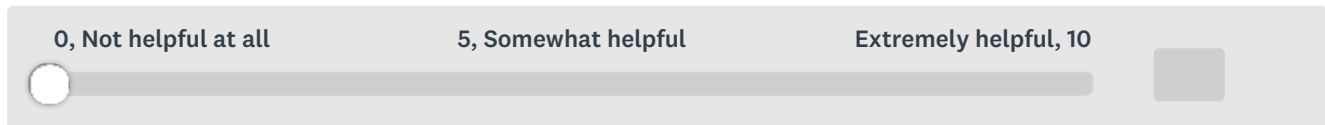A horizontal slider bar with a white circular knob at the 0 position. The bar is light gray and spans the width of the form.☐

97. Did you notice the color map differences on different MRI modalities? How helpful is this feature in clinical settings?

0, Not helpful at all                      5, Somewhat helpful                      Extremely helpful, 10

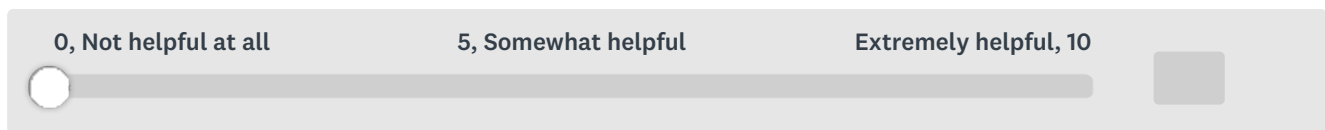A horizontal slider bar with a white circular knob at the 0 position. The bar is light gray and spans the width of the form.☐

98.

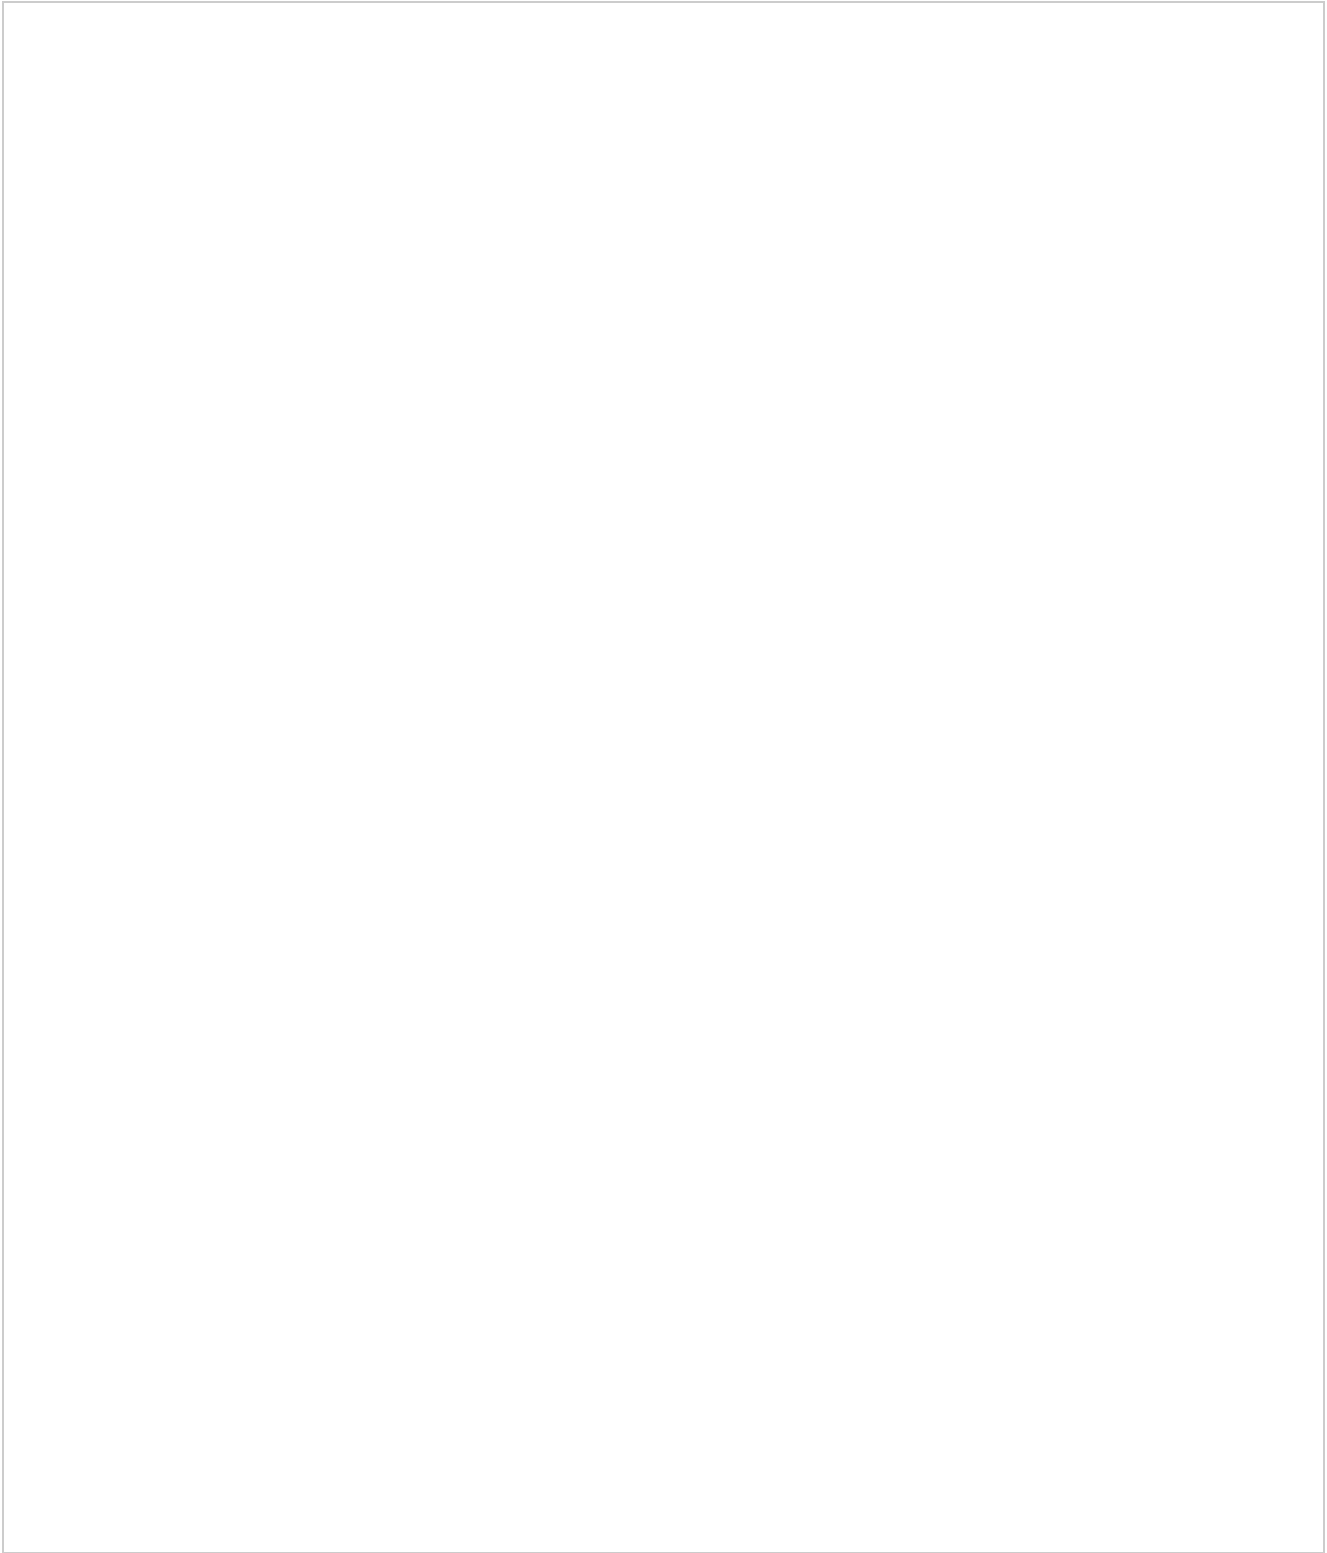

Please provide any of your comments on this color map.

99. How many percentages do the highlighted area match with your clinical judgment on the important features to classify LGG/HGG?

0%, Not matches at all                      50%                      Completely matches with mine, 100%

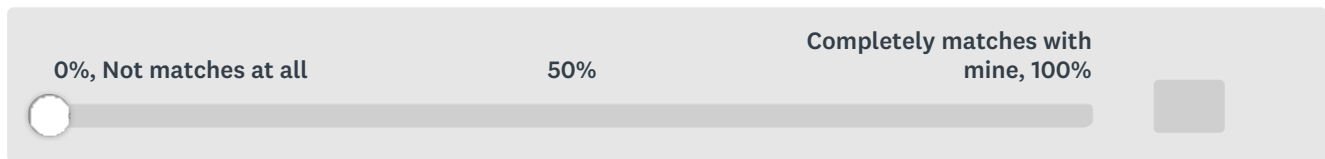A horizontal slider bar with a white circular knob at the 0% position. The bar is light gray and has a darker gray track. A small gray square button is located at the right end of the slider.

100. How helpful is this color map in clinical settings?

0, Not helpful at all                      5, Somewhat helpful                      Extremely helpful, 10

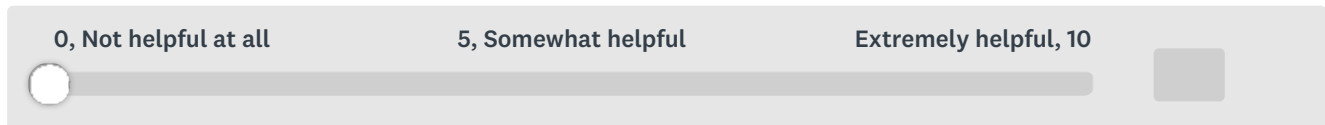A horizontal slider bar with a white circular knob at the 0 position. The bar is light gray and has a darker gray track. A small gray square button is located at the right end of the slider.

101. Did you notice the color map differences on different MRI modalities? How helpful is this feature in clinical settings?

0, Not helpful at all                      5, Somewhat helpful                      Extremely helpful, 10

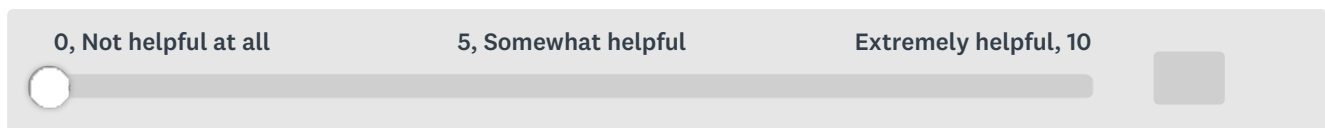A horizontal slider bar with a white circular knob at the 0 position. The bar is light gray and has a darker gray track. A small gray square button is located at the right end of the slider.

102.

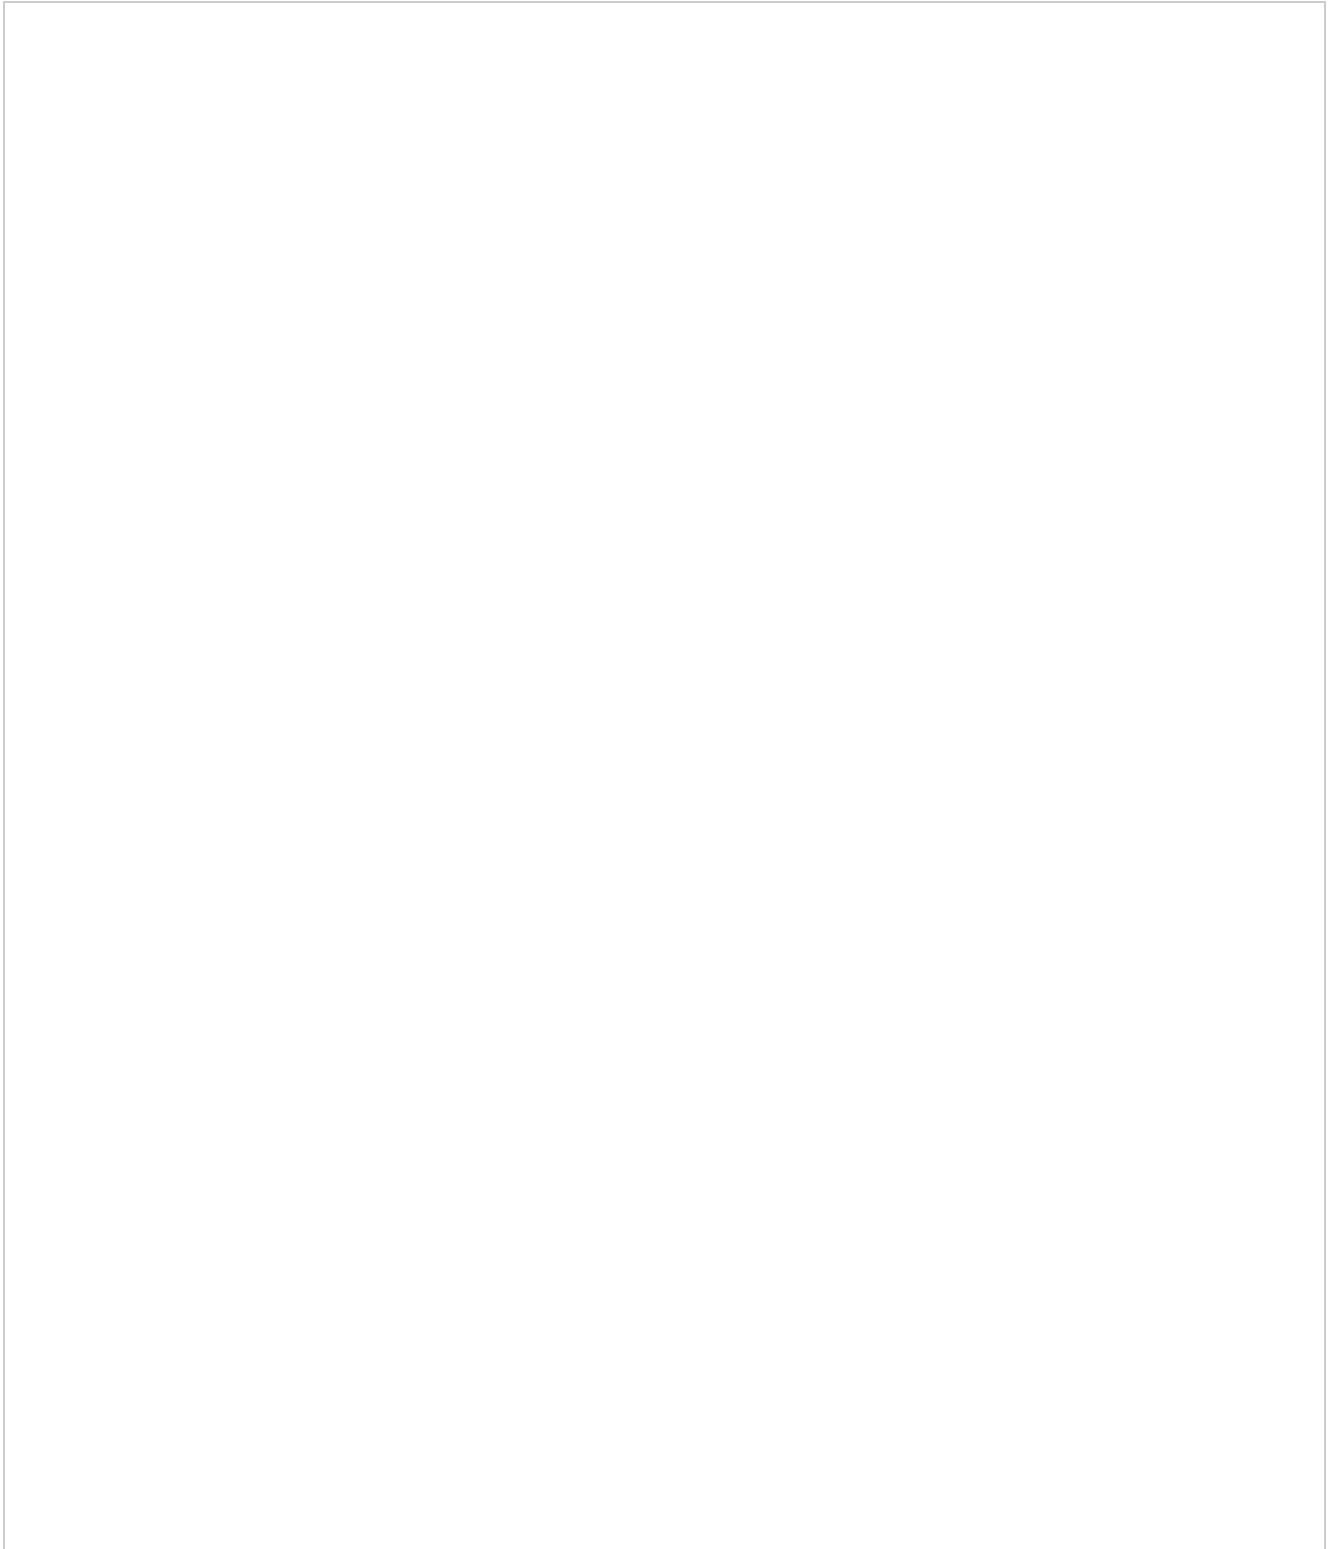

Please provide any of your comments on this color map.

A solid gray rectangular box, intended for providing comments on the color map.

103. How many percentages do the highlighted area match with your clinical judgment on the important features to classify LGG/HGG?

0%, Not matches at all                      50%                      Completely matches with mine, 100%

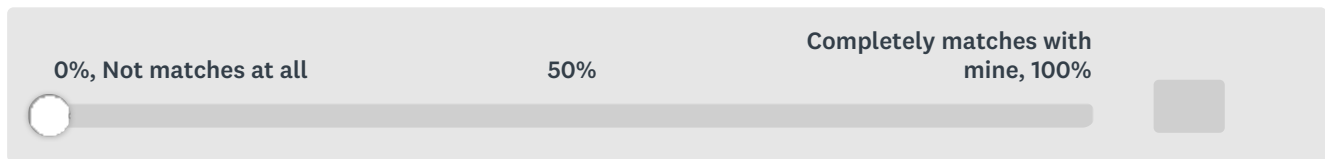A horizontal slider bar with a white circular knob at the 0% position. The bar is light gray with a darker gray track. The text "0%, Not matches at all" is on the left, "50%" is in the middle, and "Completely matches with mine, 100%" is on the right. A small gray square button is at the far right.

104. How helpful is this color map in clinical settings?

0, Not helpful at all                      5, Somewhat helpful                      Extremely helpful, 10

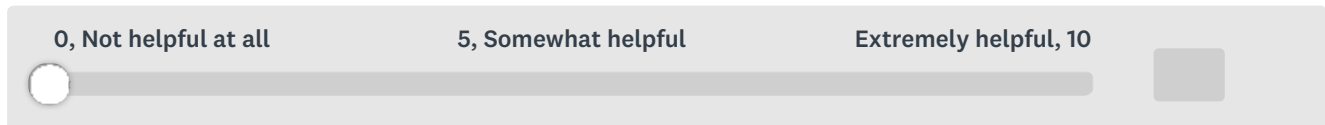A horizontal slider bar with a white circular knob at the 0 position. The bar is light gray with a darker gray track. The text "0, Not helpful at all" is on the left, "5, Somewhat helpful" is in the middle, and "Extremely helpful, 10" is on the right. A small gray square button is at the far right.

105. Did you notice the color map differences on different MRI modalities? How helpful is this feature in clinical settings?

0, Not helpful at all                      5, Somewhat helpful                      Extremely helpful, 10

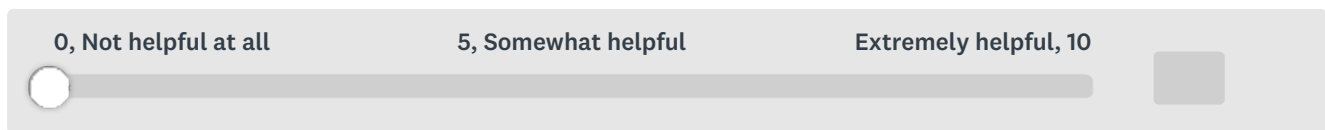A horizontal slider bar with a white circular knob at the 0 position. The bar is light gray with a darker gray track. The text "0, Not helpful at all" is on the left, "5, Somewhat helpful" is in the middle, and "Extremely helpful, 10" is on the right. A small gray square button is at the far right.

106.

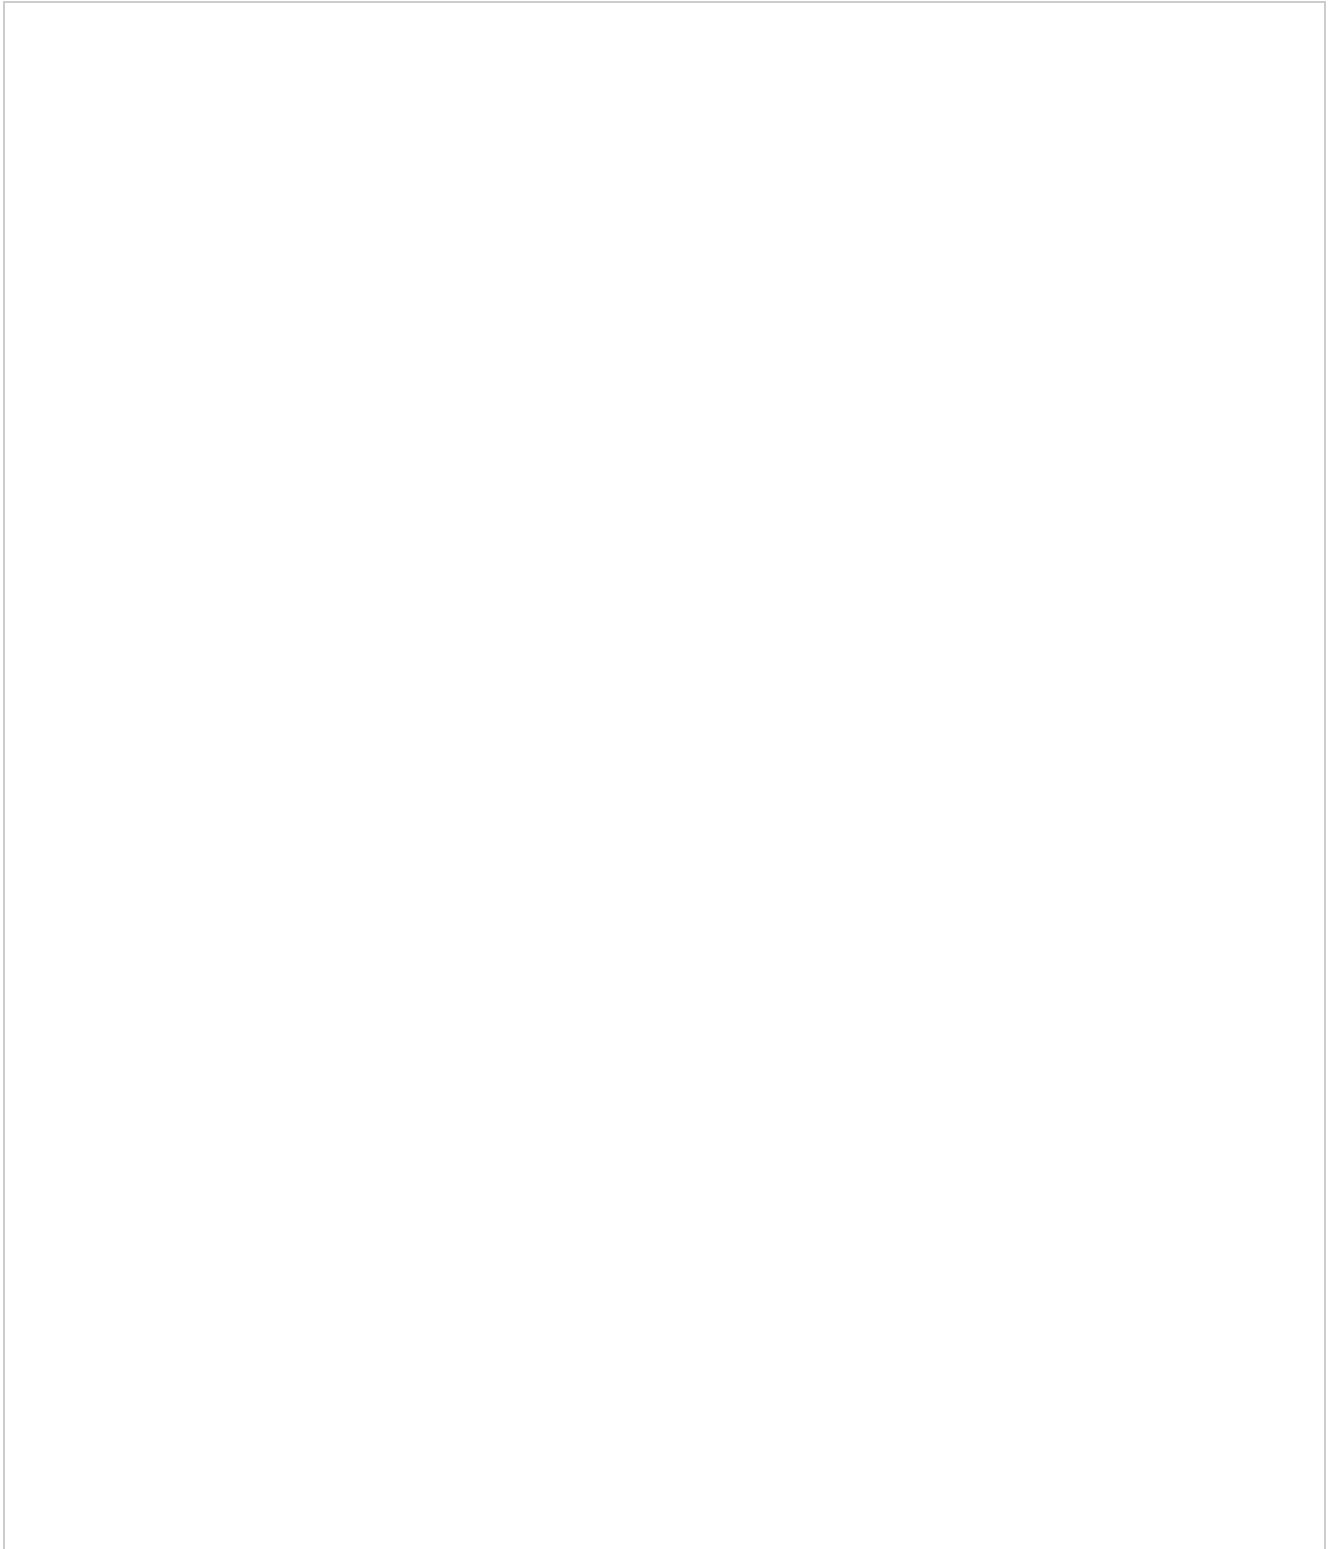

Please provide any of your comments on this color map.

A solid gray rectangular box, intended for providing comments on the color map.



107. How many percentages do the highlighted area match with your clinical judgment on the important features to classify LGG/HGG?

0%, Not matches at all                      50%                      Completely matches with mine, 100%

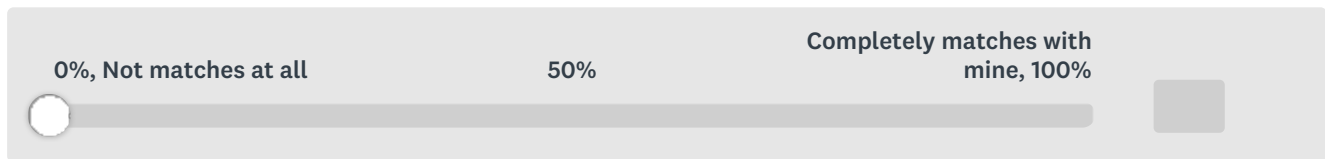A horizontal slider bar with a white circular knob at the 0% position. The bar is light gray with a darker gray track. The text "0%, Not matches at all" is on the left, "50%" is in the middle, and "Completely matches with mine, 100%" is on the right. A small gray square button is at the far right.

108. How helpful is this color map in clinical settings?

0, Not helpful at all                      5, Somewhat helpful                      Extremely helpful, 10

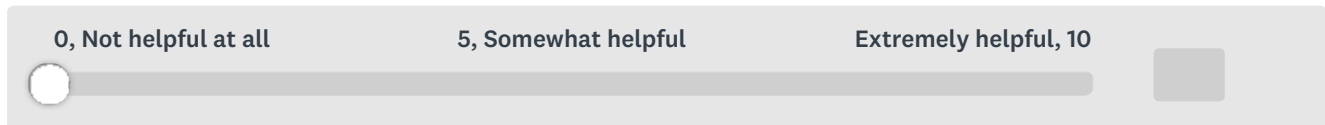A horizontal slider bar with a white circular knob at the 0 position. The bar is light gray with a darker gray track. The text "0, Not helpful at all" is on the left, "5, Somewhat helpful" is in the middle, and "Extremely helpful, 10" is on the right. A small gray square button is at the far right.

109. Did you notice the color map differences on different MRI modalities? How helpful is this feature in clinical settings?

0, Not helpful at all                      5, Somewhat helpful                      Extremely helpful, 10

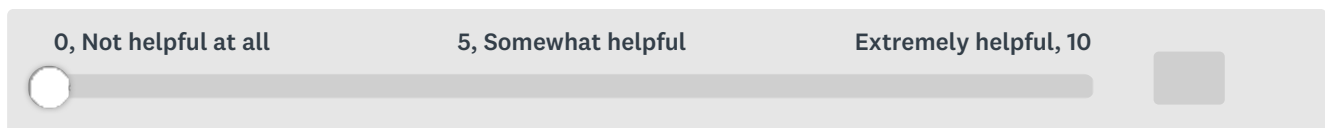A horizontal slider bar with a white circular knob at the 0 position. The bar is light gray with a darker gray track. The text "0, Not helpful at all" is on the left, "5, Somewhat helpful" is in the middle, and "Extremely helpful, 10" is on the right. A small gray square button is at the far right.

110.

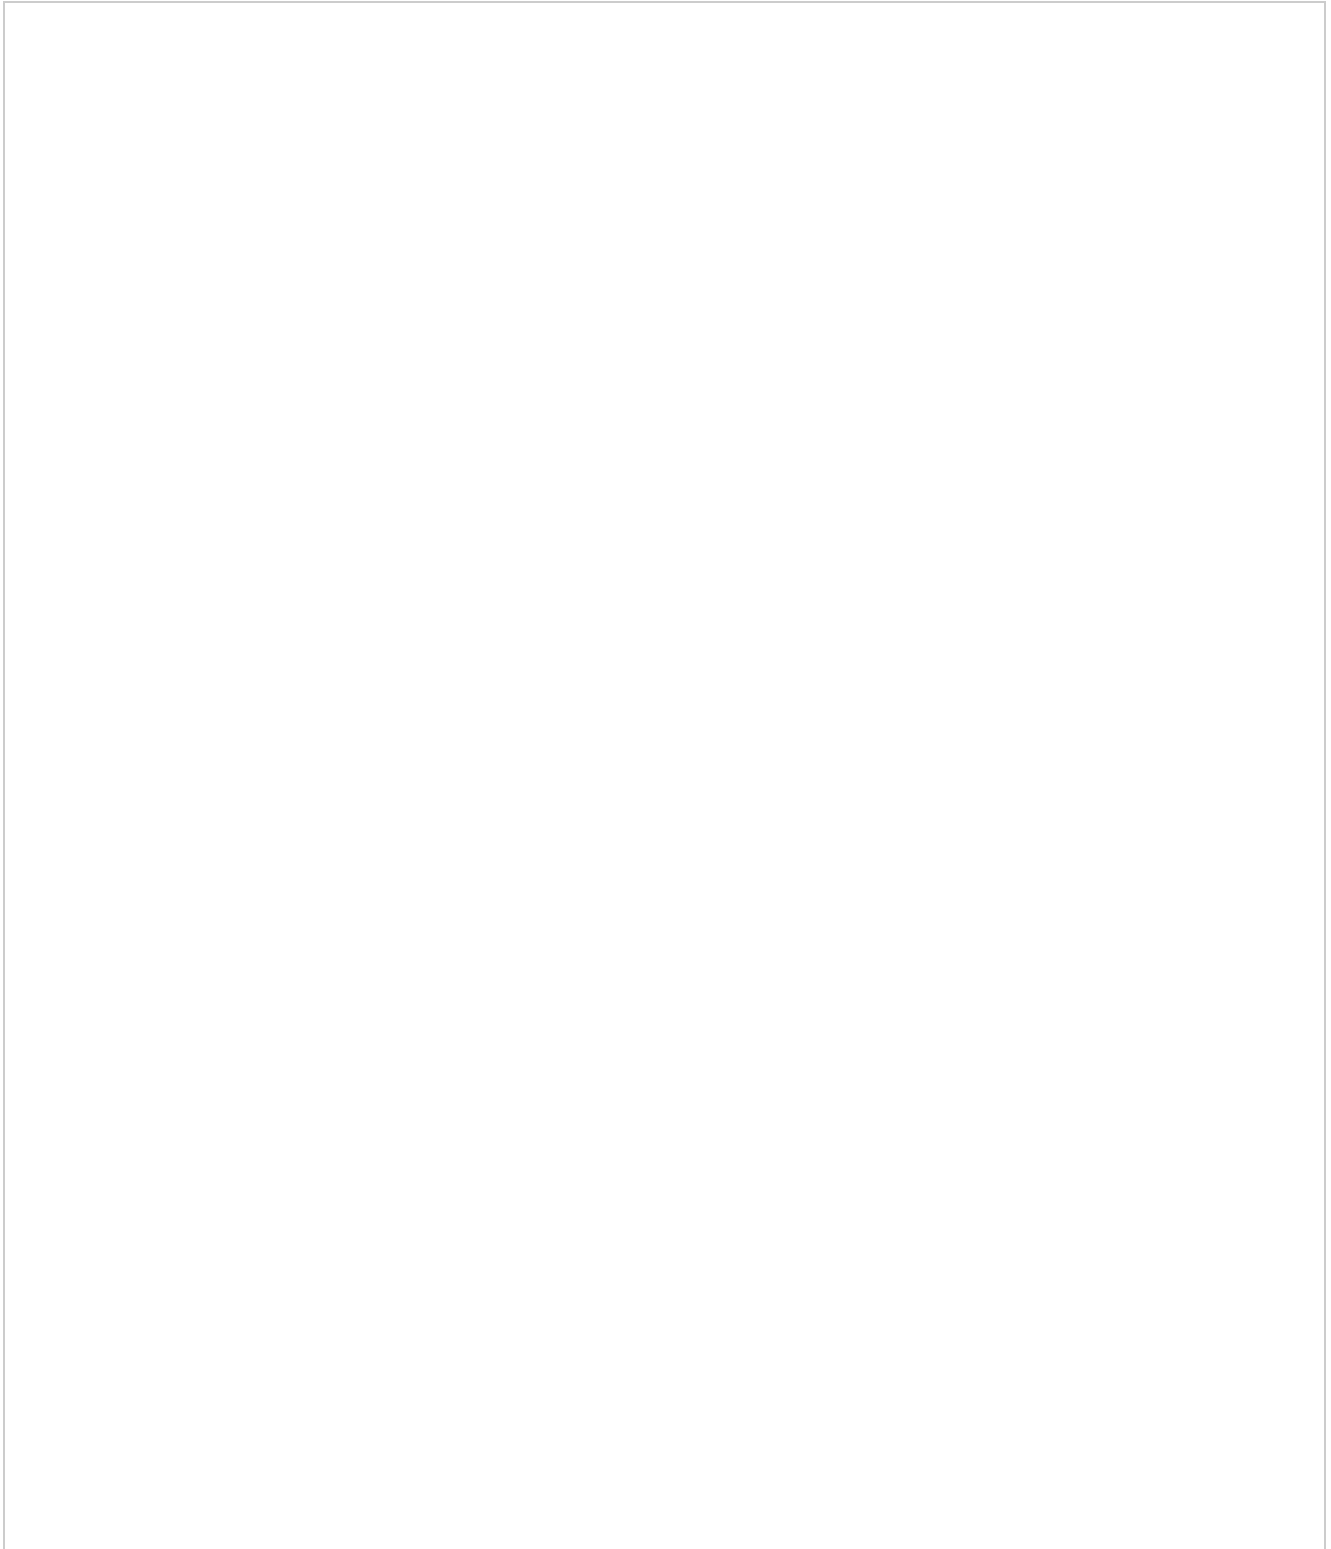

Please provide any of your comments on this color map.

A solid gray rectangular box, intended for providing comments.

111. How many percentages do the highlighted area match with your clinical judgment on the important features to classify LGG/HGG?

0%, Not matches at all                      50%                      Completely matches with mine, 100%

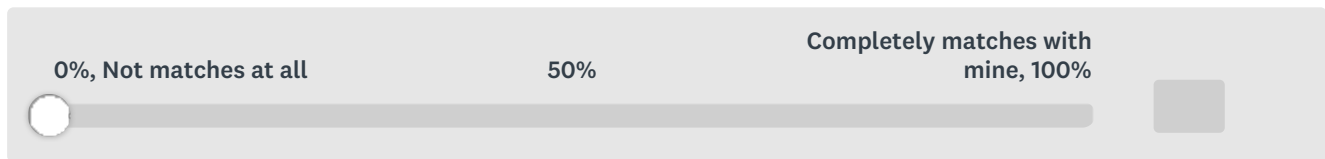A horizontal slider bar with a white circular knob at the 0% position. The bar is light gray and has a darker gray track. A small gray square button is located at the right end of the slider.

112. How helpful is this color map in clinical settings?

0, Not helpful at all                      5, Somewhat helpful                      Extremely helpful, 10

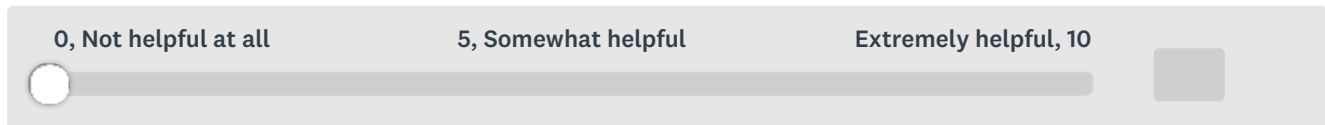A horizontal slider bar with a white circular knob at the 0 position. The bar is light gray and has a darker gray track. A small gray square button is located at the right end of the slider.

113. Did you notice the **color map differences** on **different MRI modalities**? How helpful is this feature in clinical settings?

0, Not helpful at all                      5, Somewhat helpful                      Extremely helpful, 10

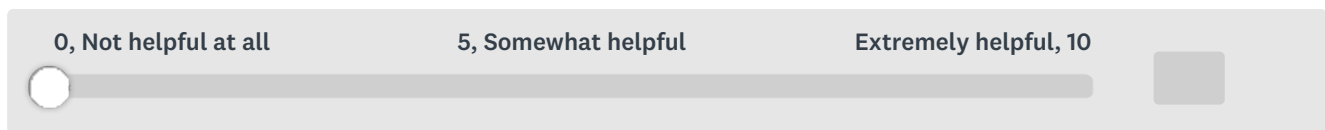A horizontal slider bar with a white circular knob at the 0 position. The bar is light gray and has a darker gray track. A small gray square button is located at the right end of the slider.

114.

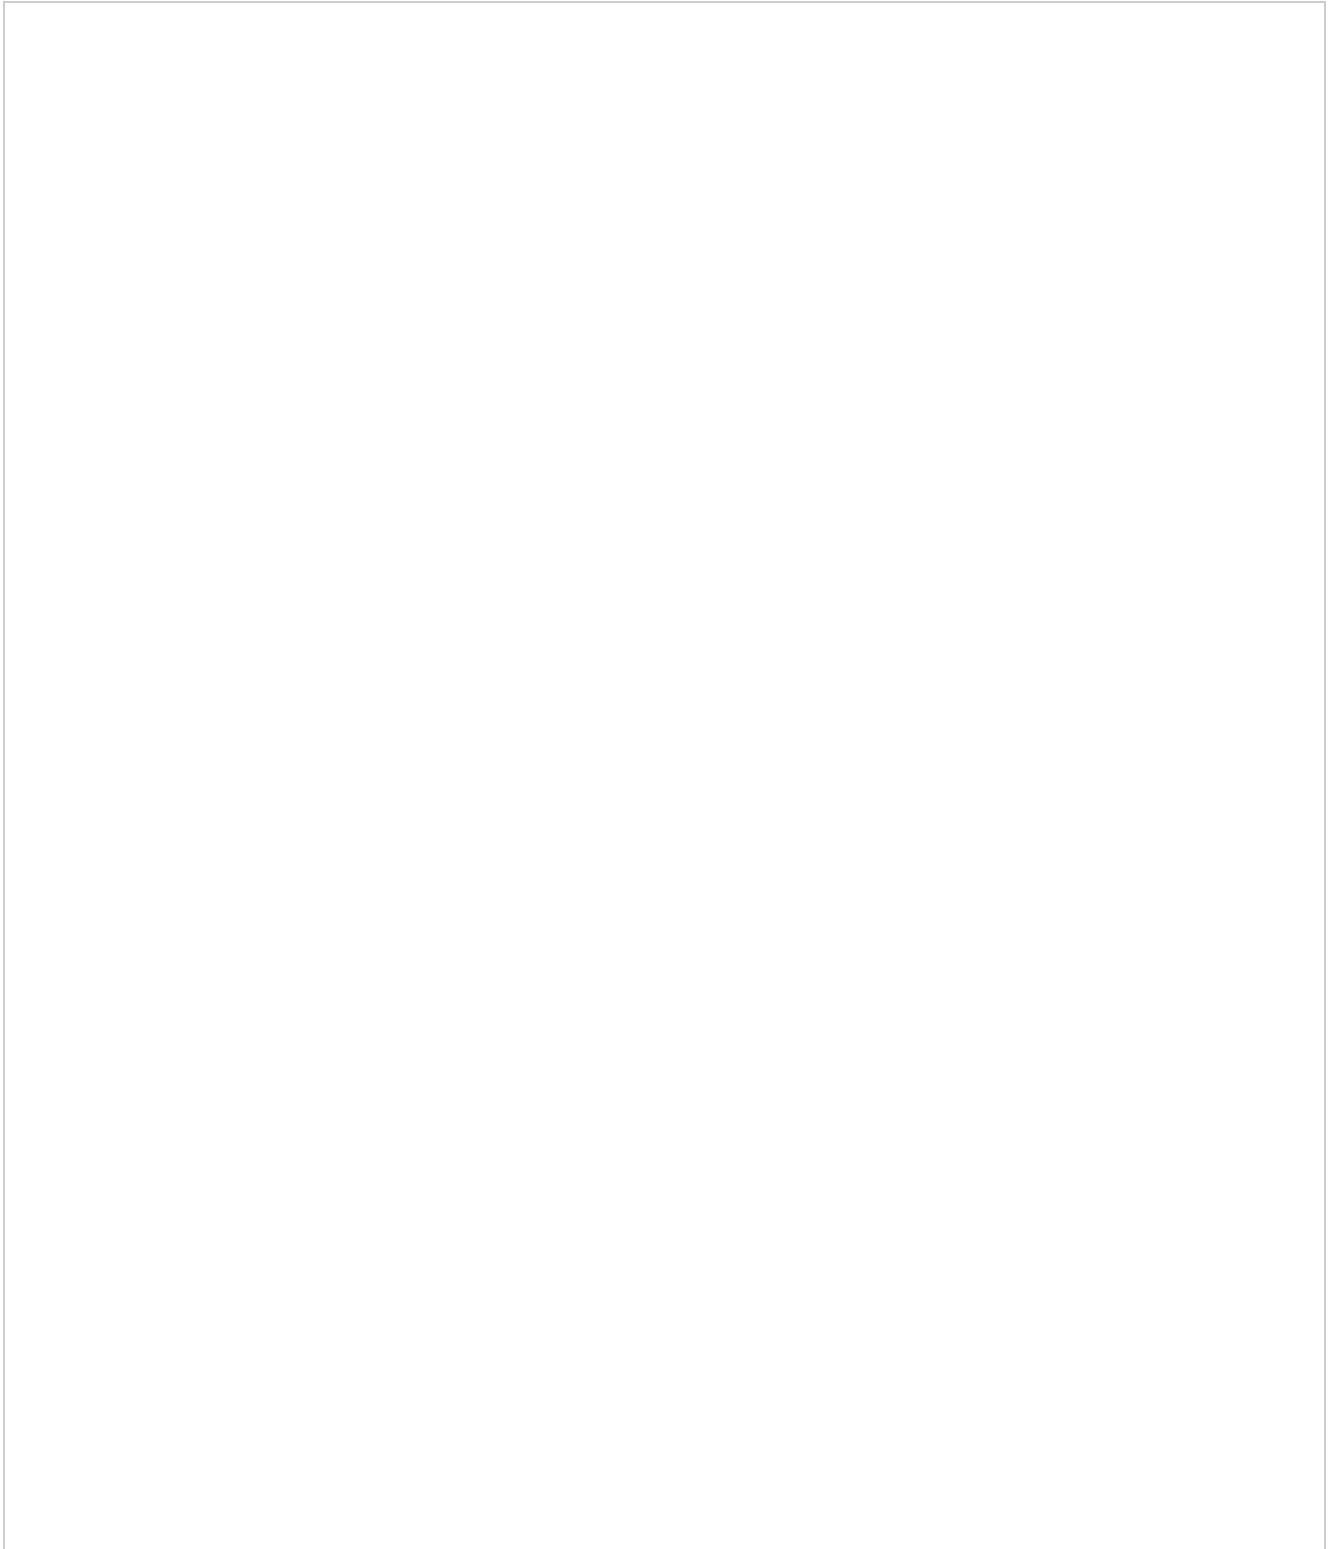

Please provide any of your comments on this color map.

A solid gray rectangular box, intended for providing comments on the color map.

115. How many percentages do the highlighted area match with your clinical judgment on the important features to classify LGG/HGG?

0%, Not matches at all                      50%                      Completely matches with mine, 100%

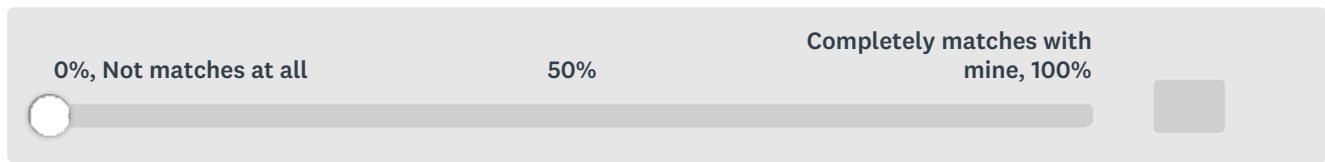A horizontal slider bar with a white circular knob at the 0% position. The bar is light gray and has a darker gray track. A small gray square button is located at the right end of the slider.

116. How helpful is this color map in clinical settings?

0, Not helpful at all                      5, Somewhat helpful                      Extremely helpful, 10

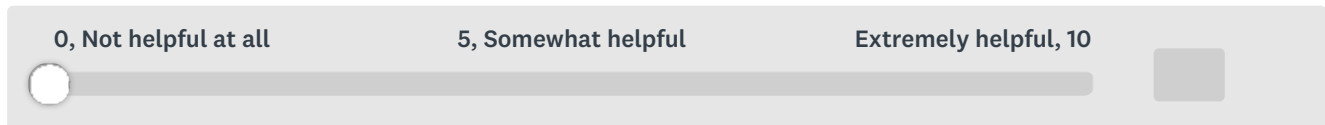A horizontal slider bar with a white circular knob at the 0 position. The bar is light gray and has a darker gray track. A small gray square button is located at the right end of the slider.

117. Did you notice the **color map differences** on **different MRI modalities**? How helpful is this feature in clinical settings?

0, Not helpful at all                      5, Somewhat helpful                      Extremely helpful, 10

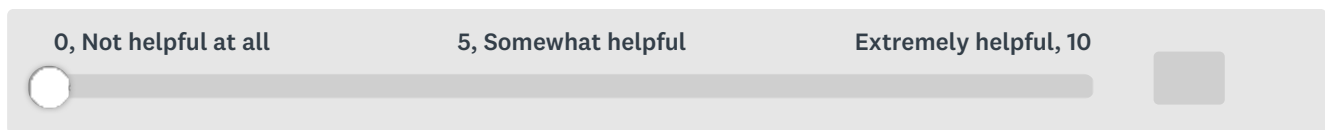A horizontal slider bar with a white circular knob at the 0 position. The bar is light gray and has a darker gray track. A small gray square button is located at the right end of the slider.

118.

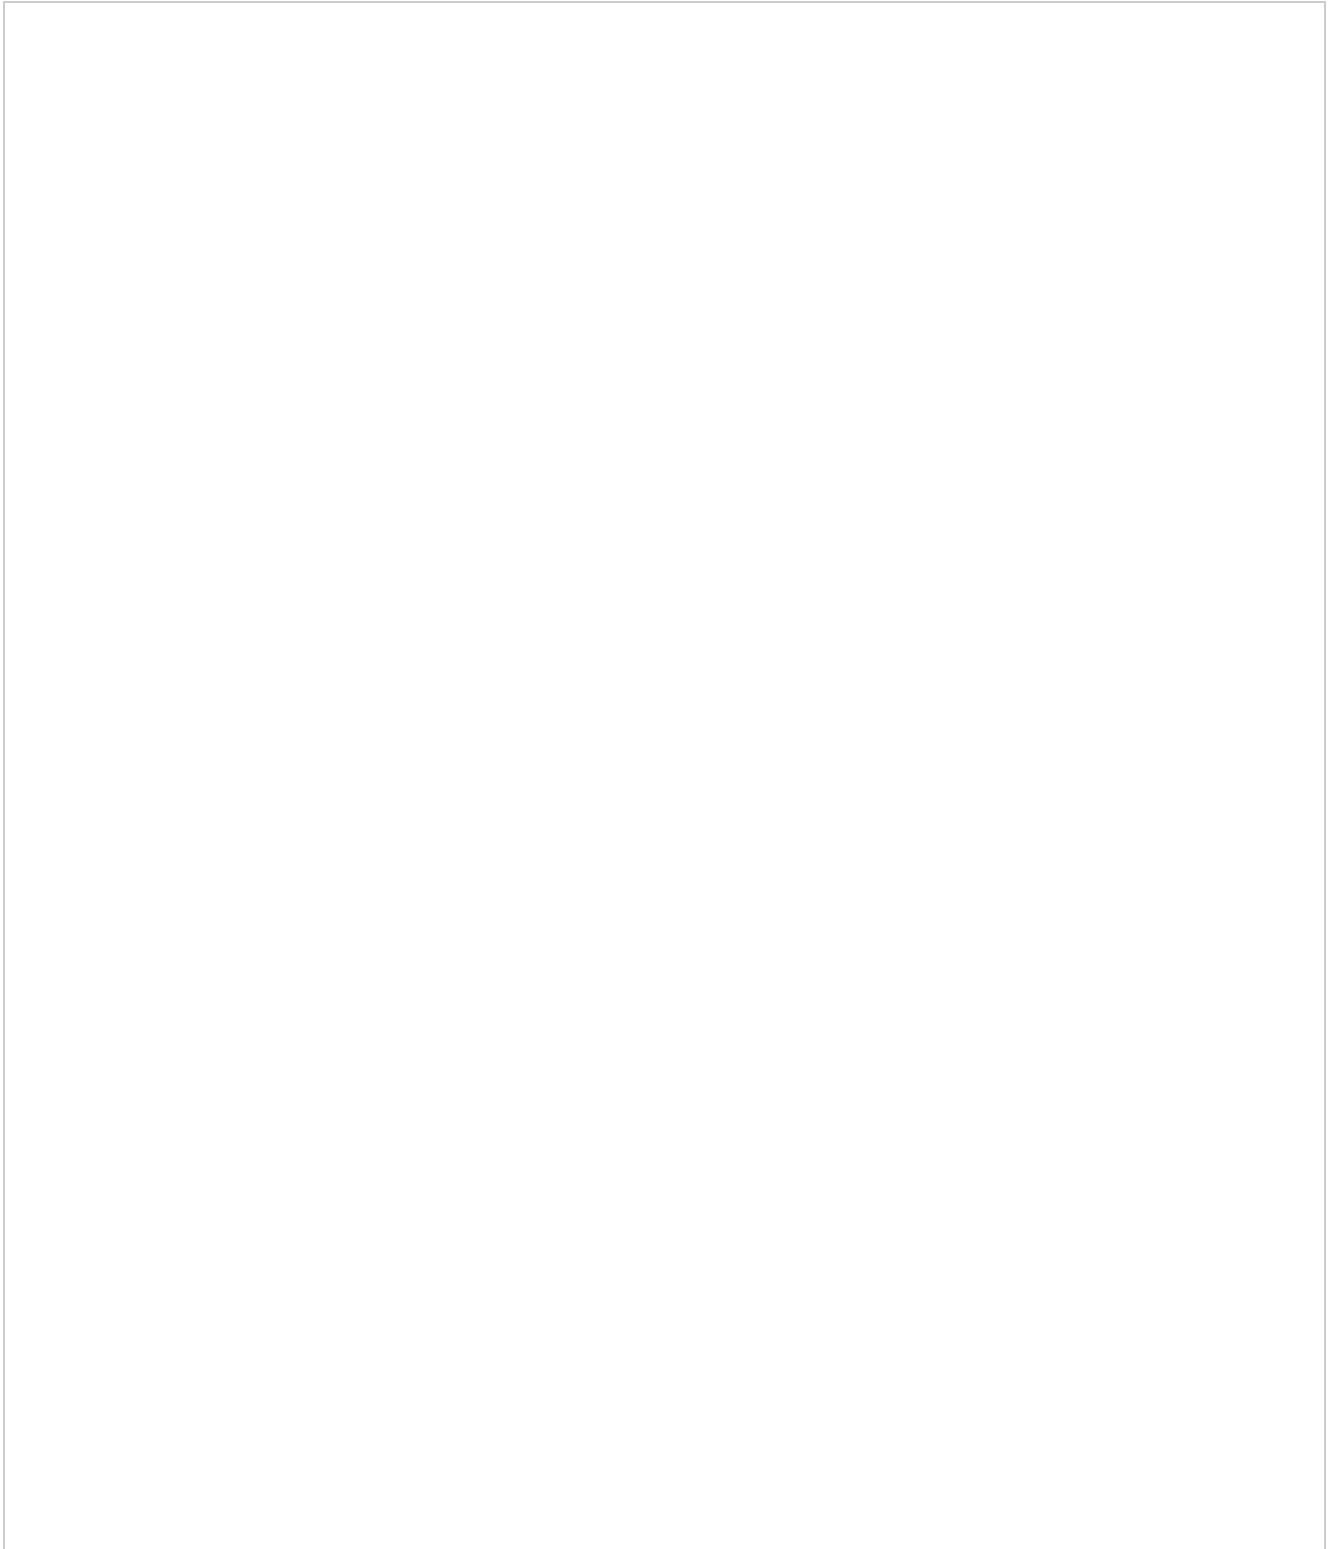

Please provide any of your comments on this color map.

A solid gray rectangular box, intended for providing comments on the color map.

119. How many percentages do the highlighted area match with your clinical judgment on the important features to classify LGG/HGG?

0%, Not matches at all                      50%                      Completely matches with mine, 100%

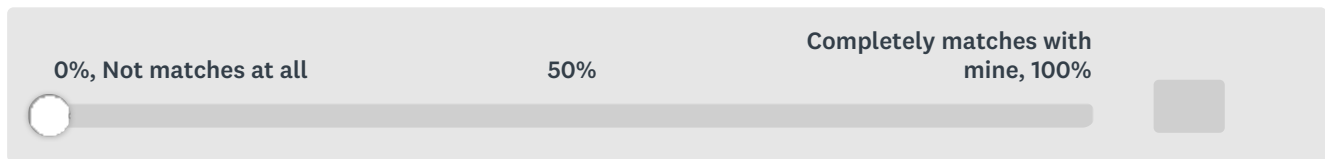A horizontal slider bar with a white circular knob at the 0% position. The bar is light gray and spans the width of the question area.☐

120. How helpful is this color map in clinical settings?

0, Not helpful at all                      5, Somewhat helpful                      Extremely helpful, 10

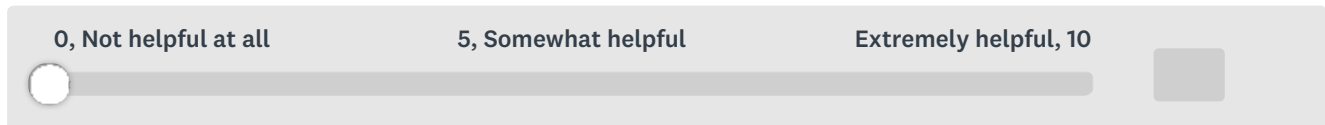A horizontal slider bar with a white circular knob at the 0 position. The bar is light gray and spans the width of the question area.☐

121. Did you notice the color map differences on different MRI modalities? How helpful is this feature in clinical settings?

0, Not helpful at all                      5, Somewhat helpful                      Extremely helpful, 10

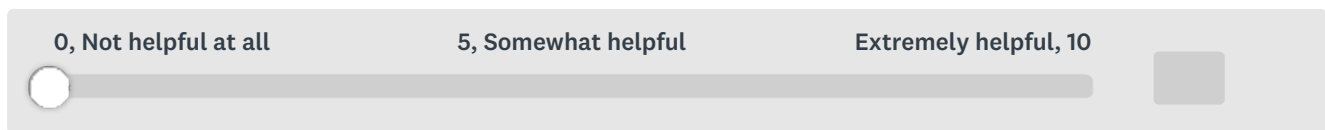A horizontal slider bar with a white circular knob at the 0 position. The bar is light gray and spans the width of the question area.☐

122.

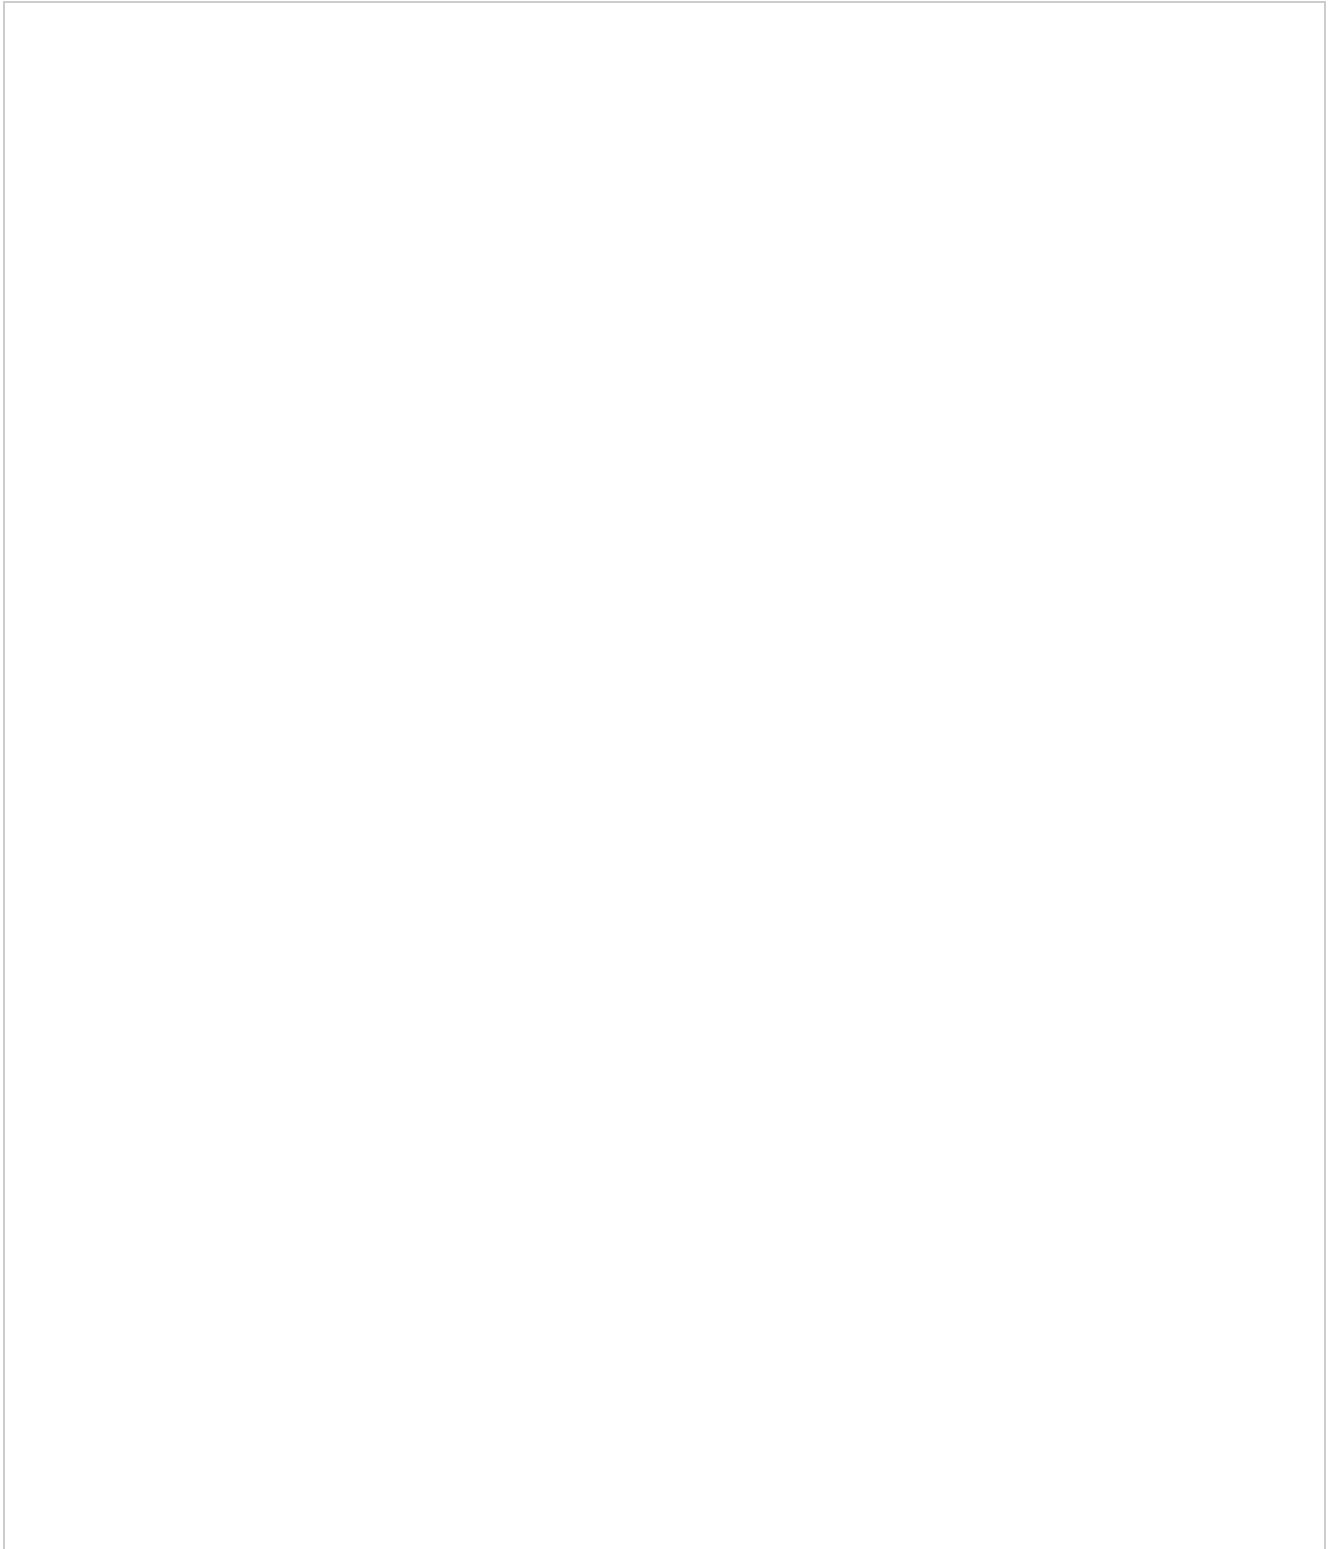

Please provide any of your comments on this color map.

A solid gray rectangular box, intended for providing comments on the color map.



123. How many percentages do the highlighted area match with your clinical judgment on the important features to classify LGG/HGG?

0%, Not matches at all                      50%                      Completely matches with mine, 100%

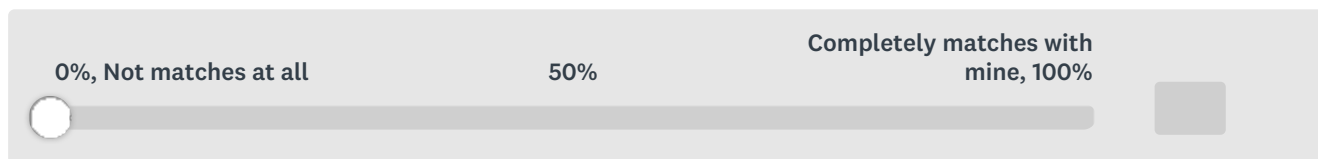A horizontal slider bar with a white circular knob at the 0% position. The bar is light gray and has a darker gray segment from 0% to 50%. To the right of the bar is a small gray square button.

☐

124. How helpful is this color map in clinical settings?

0, Not helpful at all                      5, Somewhat helpful                      Extremely helpful, 10

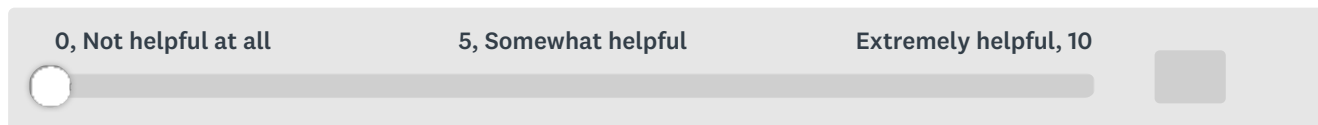A horizontal slider bar with a white circular knob at the 0 position. The bar is light gray and has a darker gray segment from 0 to 5. To the right of the bar is a small gray square button.

☐

125. Did you notice the color map differences on different MRI modalities? How helpful is this feature in clinical settings?

0, Not helpful at all                      5, Somewhat helpful                      Extremely helpful, 10

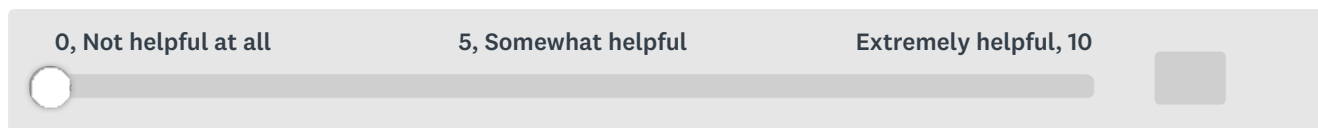A horizontal slider bar with a white circular knob at the 0 position. The bar is light gray and has a darker gray segment from 0 to 5. To the right of the bar is a small gray square button.

☐

126.

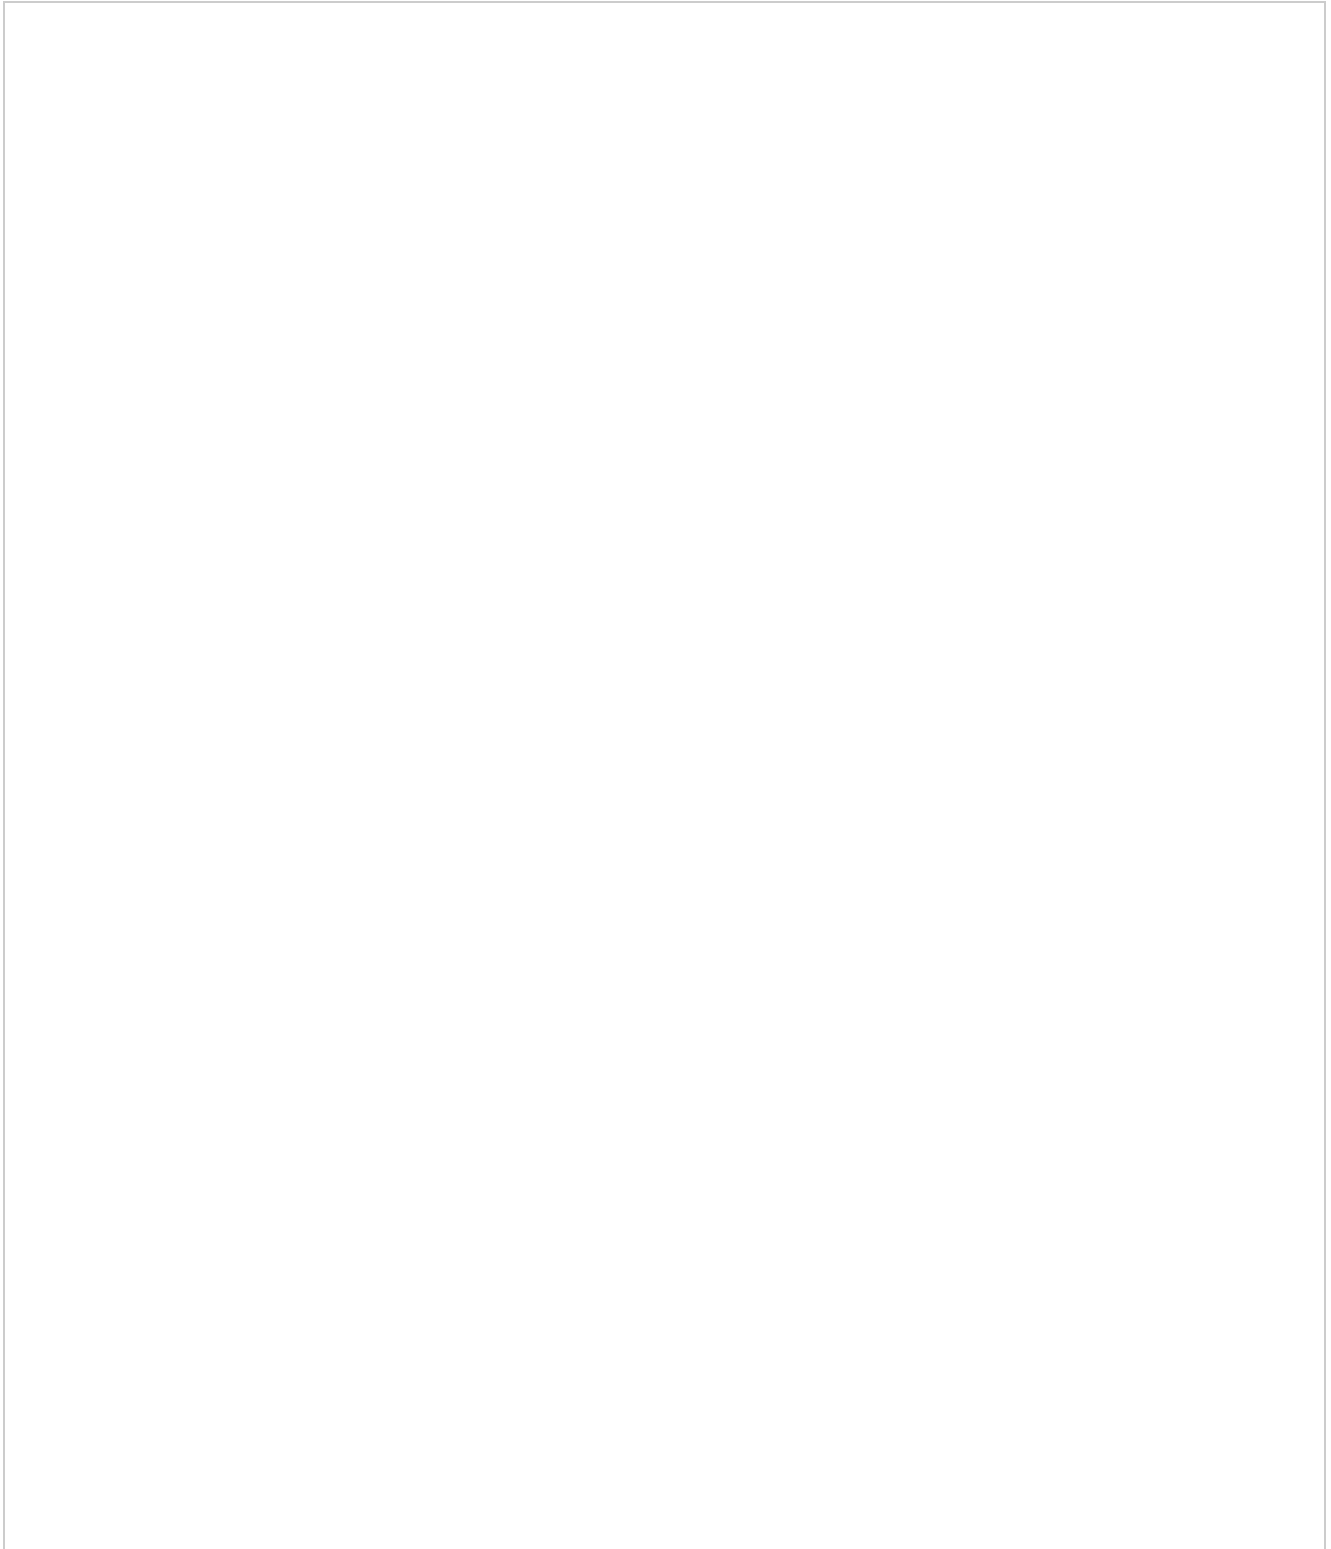

Please provide any of your comments on this color map.

A solid gray rectangular box, intended for providing comments on the color map.

127. How many percentages do the highlighted area match with your clinical judgment on the important features to classify LGG/HGG?

0%, Not matches at all                      50%                      Completely matches with mine, 100%

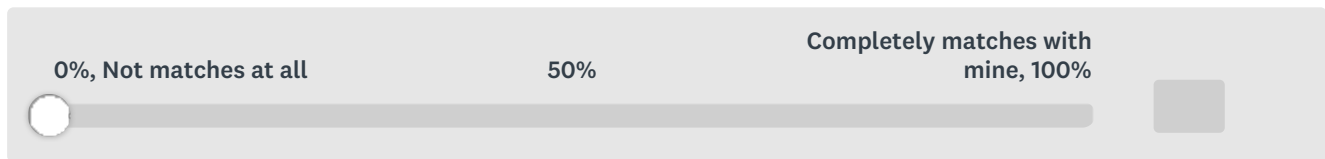A horizontal slider bar with a white circular knob at the 0% position. The bar is light gray and has a darker gray segment at the end. A small gray square button is located to the right of the slider.

128. How helpful is this color map in clinical settings?

0, Not helpful at all                      5, Somewhat helpful                      Extremely helpful, 10

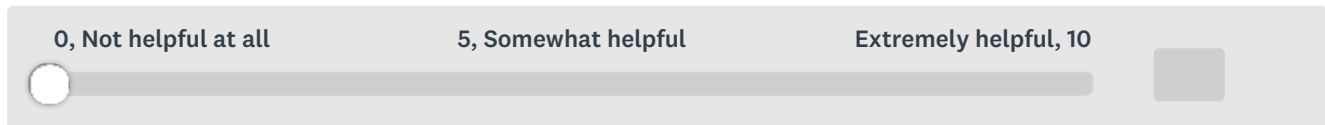A horizontal slider bar with a white circular knob at the 0 position. The bar is light gray and has a darker gray segment at the end. A small gray square button is located to the right of the slider.

129. Did you notice the color map differences on different MRI modalities? How helpful is this feature in clinical settings?

0, Not helpful at all                      5, Somewhat helpful                      Extremely helpful, 10

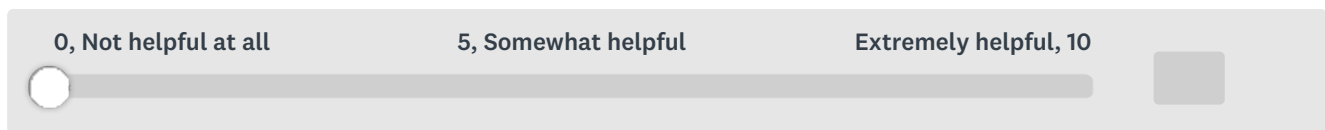A horizontal slider bar with a white circular knob at the 0 position. The bar is light gray and has a darker gray segment at the end. A small gray square button is located to the right of the slider.

130.

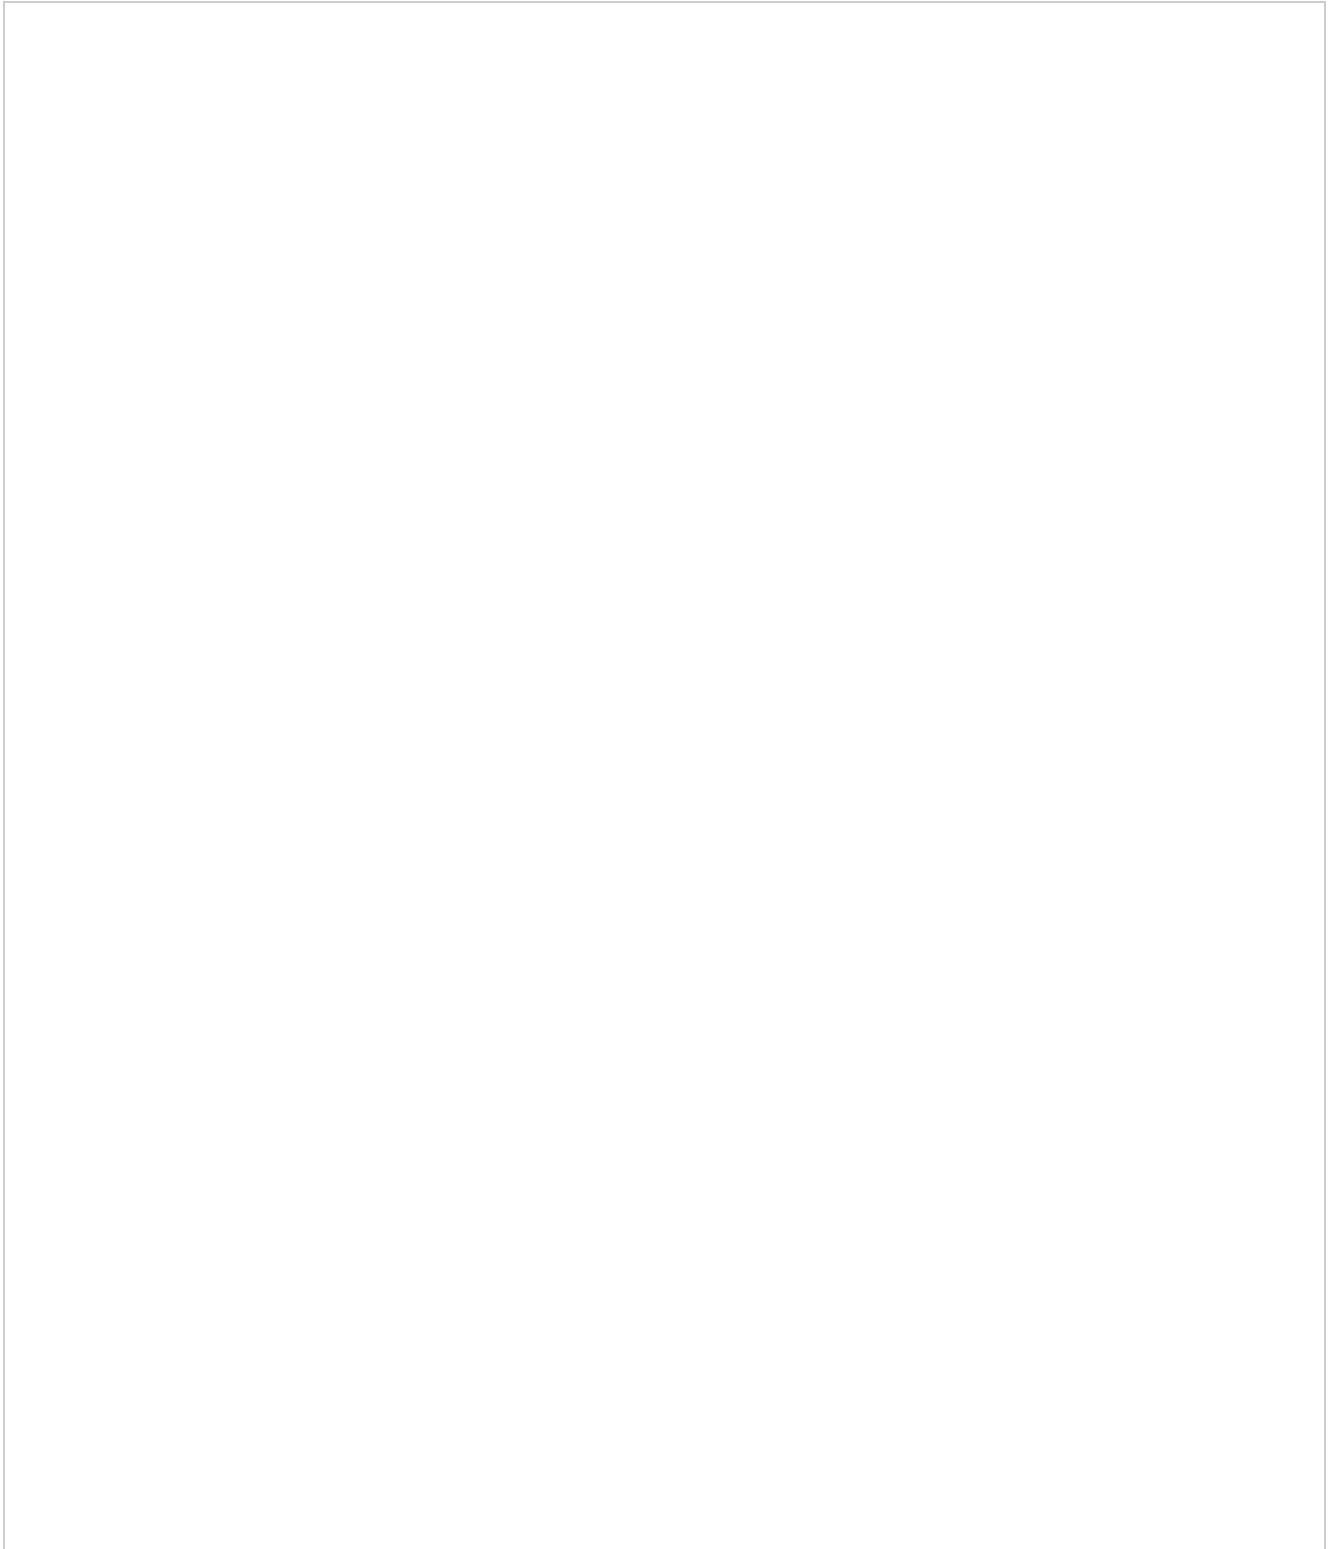

Please provide any of your comments on this color map.

A solid gray rectangular box, intended for providing comments on the color map.

131. How many percentages do the highlighted area match with your clinical judgment on the important features to classify LGG/HGG?

0%, Not matches at all                      50%                      Completely matches with mine, 100%

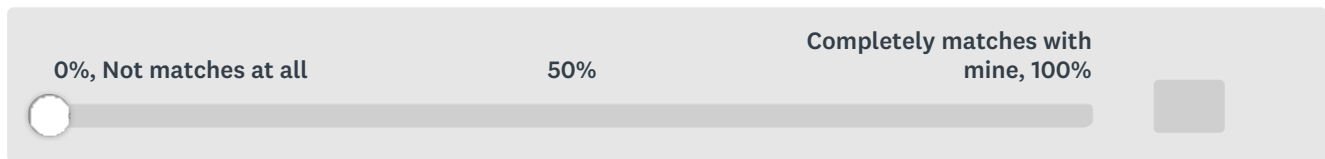A horizontal slider bar with a white circular knob at the 0% position. The bar is light gray and spans the width of the form.☐

132. How helpful is this color map in clinical settings?

0, Not helpful at all                      5, Somewhat helpful                      Extremely helpful, 10

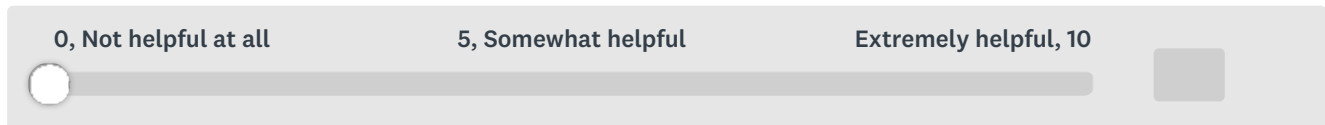A horizontal slider bar with a white circular knob at the 0 position. The bar is light gray and spans the width of the form.☐

133. Did you notice the color map differences on different MRI modalities? How helpful is this feature in clinical settings?

0, Not helpful at all                      5, Somewhat helpful                      Extremely helpful, 10

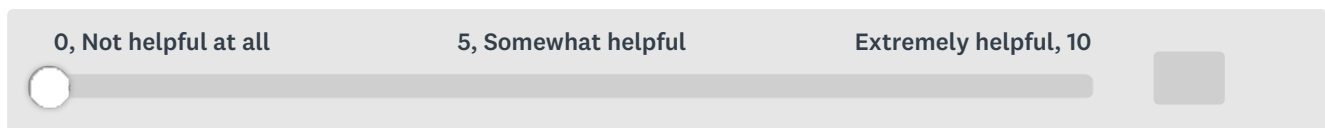A horizontal slider bar with a white circular knob at the 0 position. The bar is light gray and spans the width of the form.☐

134.

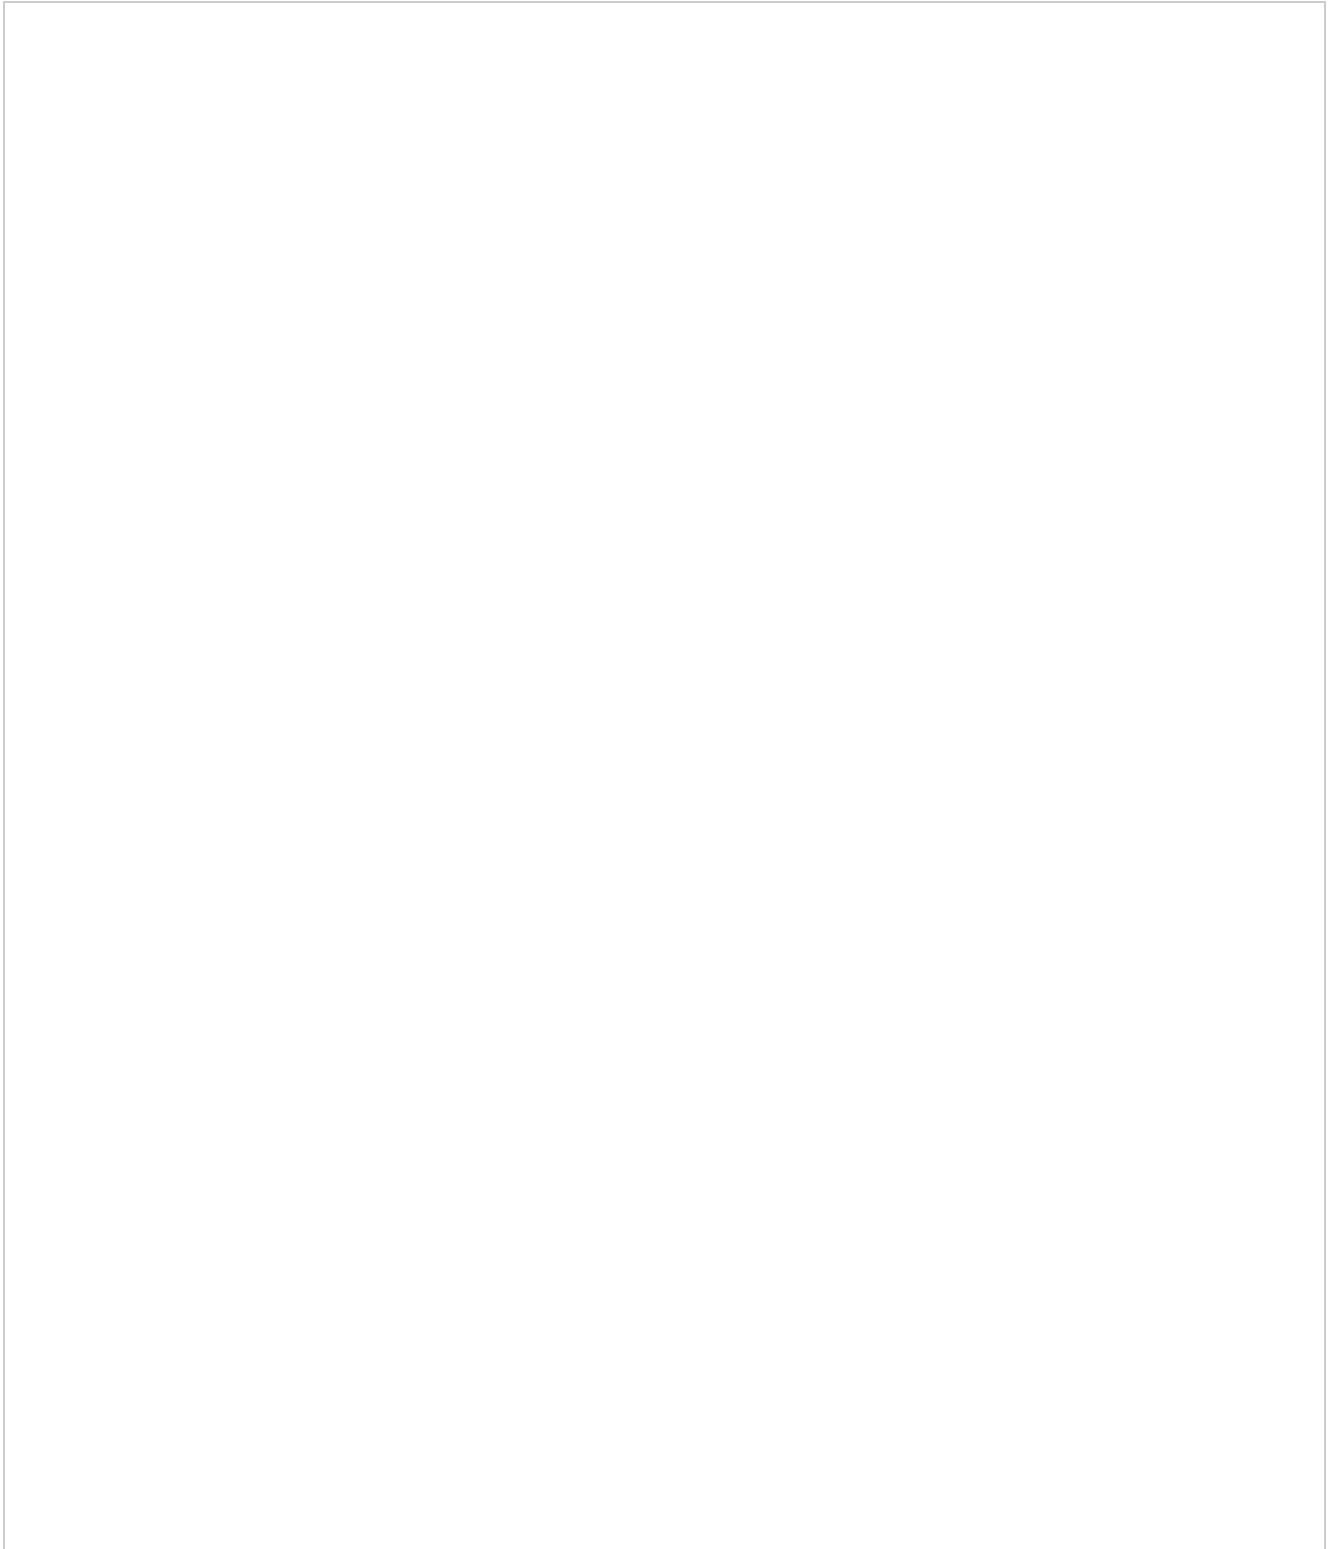

Please provide any of your comments on this color map.

A solid gray rectangular box, intended for providing comments on the color map.

135. How many percentages do the highlighted area match with your clinical judgment on the important features to classify LGG/HGG?

0%, Not matches at all                      50%                      Completely matches with mine, 100%

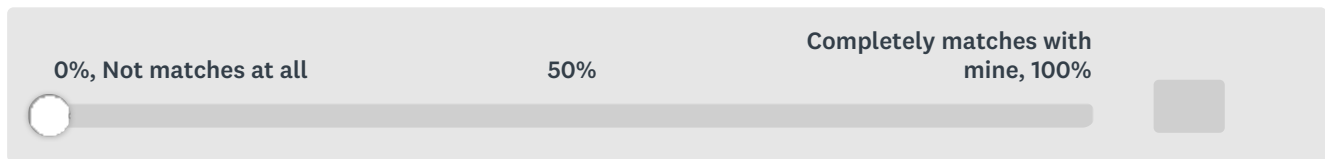A horizontal slider bar with a white circular knob at the 0% position. The bar is light gray and has a darker gray track. A small gray square button is located at the right end of the slider.

136. How helpful is this color map in clinical settings?

0, Not helpful at all                      5, Somewhat helpful                      Extremely helpful, 10

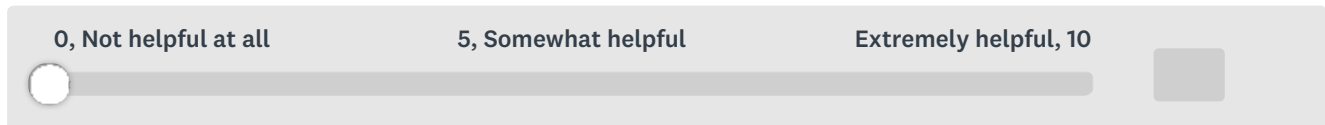A horizontal slider bar with a white circular knob at the 0 position. The bar is light gray and has a darker gray track. A small gray square button is located at the right end of the slider.

137. Did you notice the **color map differences** on **different MRI modalities**? How helpful is this feature in clinical settings?

0, Not helpful at all                      5, Somewhat helpful                      Extremely helpful, 10

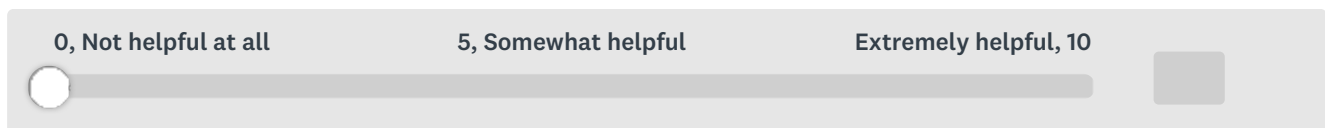A horizontal slider bar with a white circular knob at the 0 position. The bar is light gray and has a darker gray track. A small gray square button is located at the right end of the slider.

138.

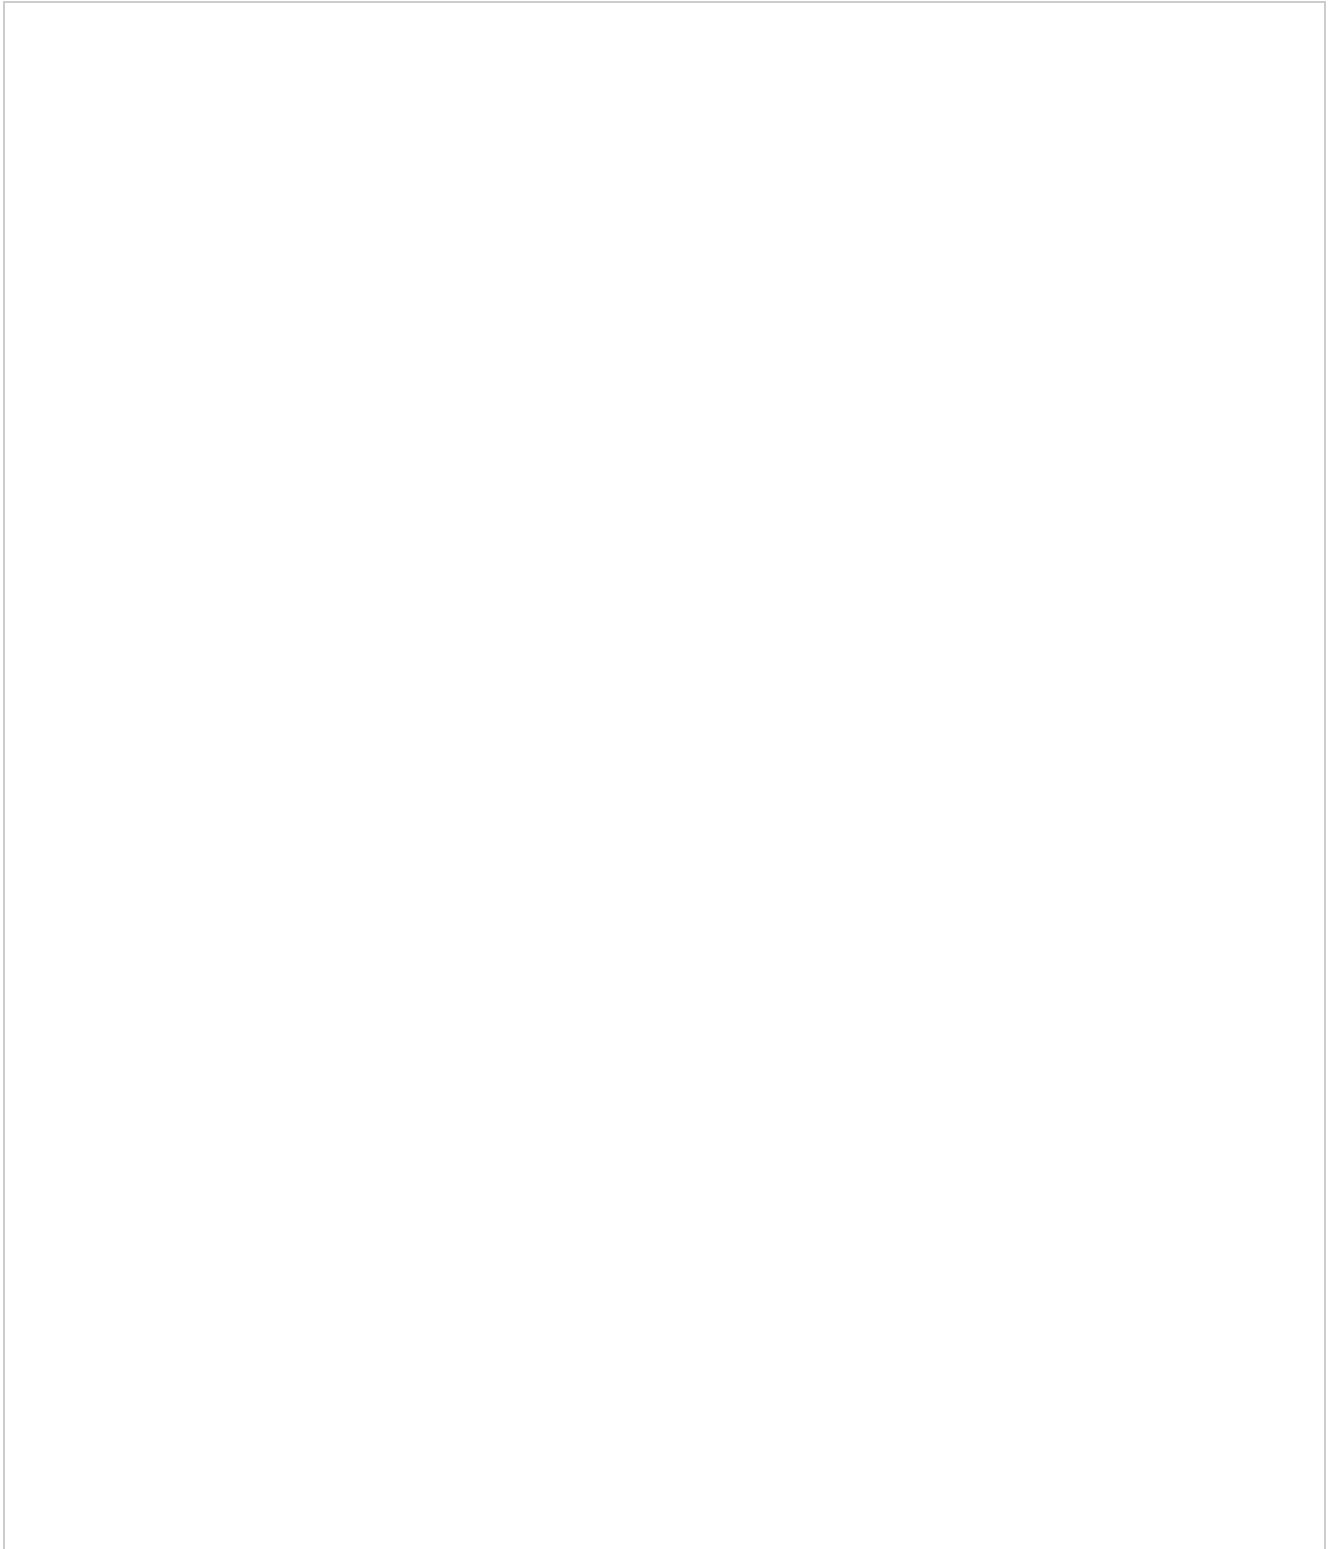

Please provide any of your comments on this color map.

A solid gray rectangular box, intended for providing comments on the color map.



139. How many percentages do the highlighted area match with your clinical judgment on the important features to classify LGG/HGG?

0%, Not matches at all                      50%                      Completely matches with mine, 100%

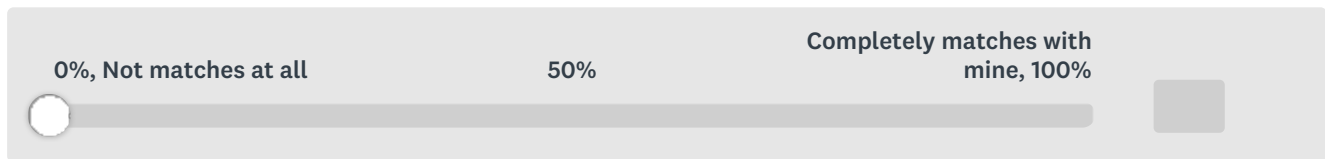A horizontal slider bar with a white circular knob at the 0% position. The bar is light gray with a darker gray track. The text "0%, Not matches at all" is on the left, "50%" is in the middle, and "Completely matches with mine, 100%" is on the right.☐

140. How helpful is this color map in clinical settings?

0, Not helpful at all                      5, Somewhat helpful                      Extremely helpful, 10

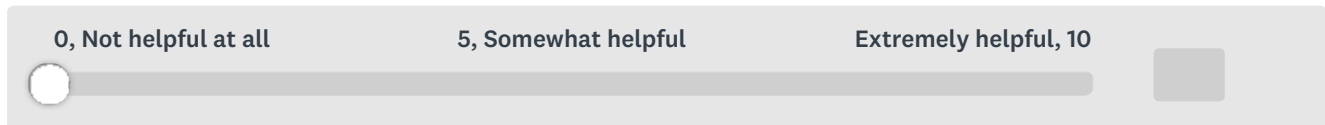A horizontal slider bar with a white circular knob at the 0 position. The bar is light gray with a darker gray track. The text "0, Not helpful at all" is on the left, "5, Somewhat helpful" is in the middle, and "Extremely helpful, 10" is on the right.☐

141. Did you notice the **color map differences** on **different MRI modalities**? How helpful is this feature in clinical settings?

0, Not helpful at all                      5, Somewhat helpful                      Extremely helpful, 10

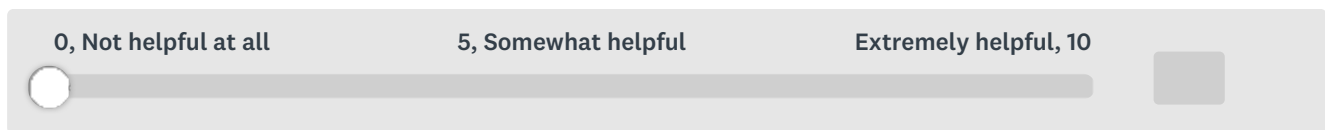A horizontal slider bar with a white circular knob at the 0 position. The bar is light gray with a darker gray track. The text "0, Not helpful at all" is on the left, "5, Somewhat helpful" is in the middle, and "Extremely helpful, 10" is on the right.☐

142.

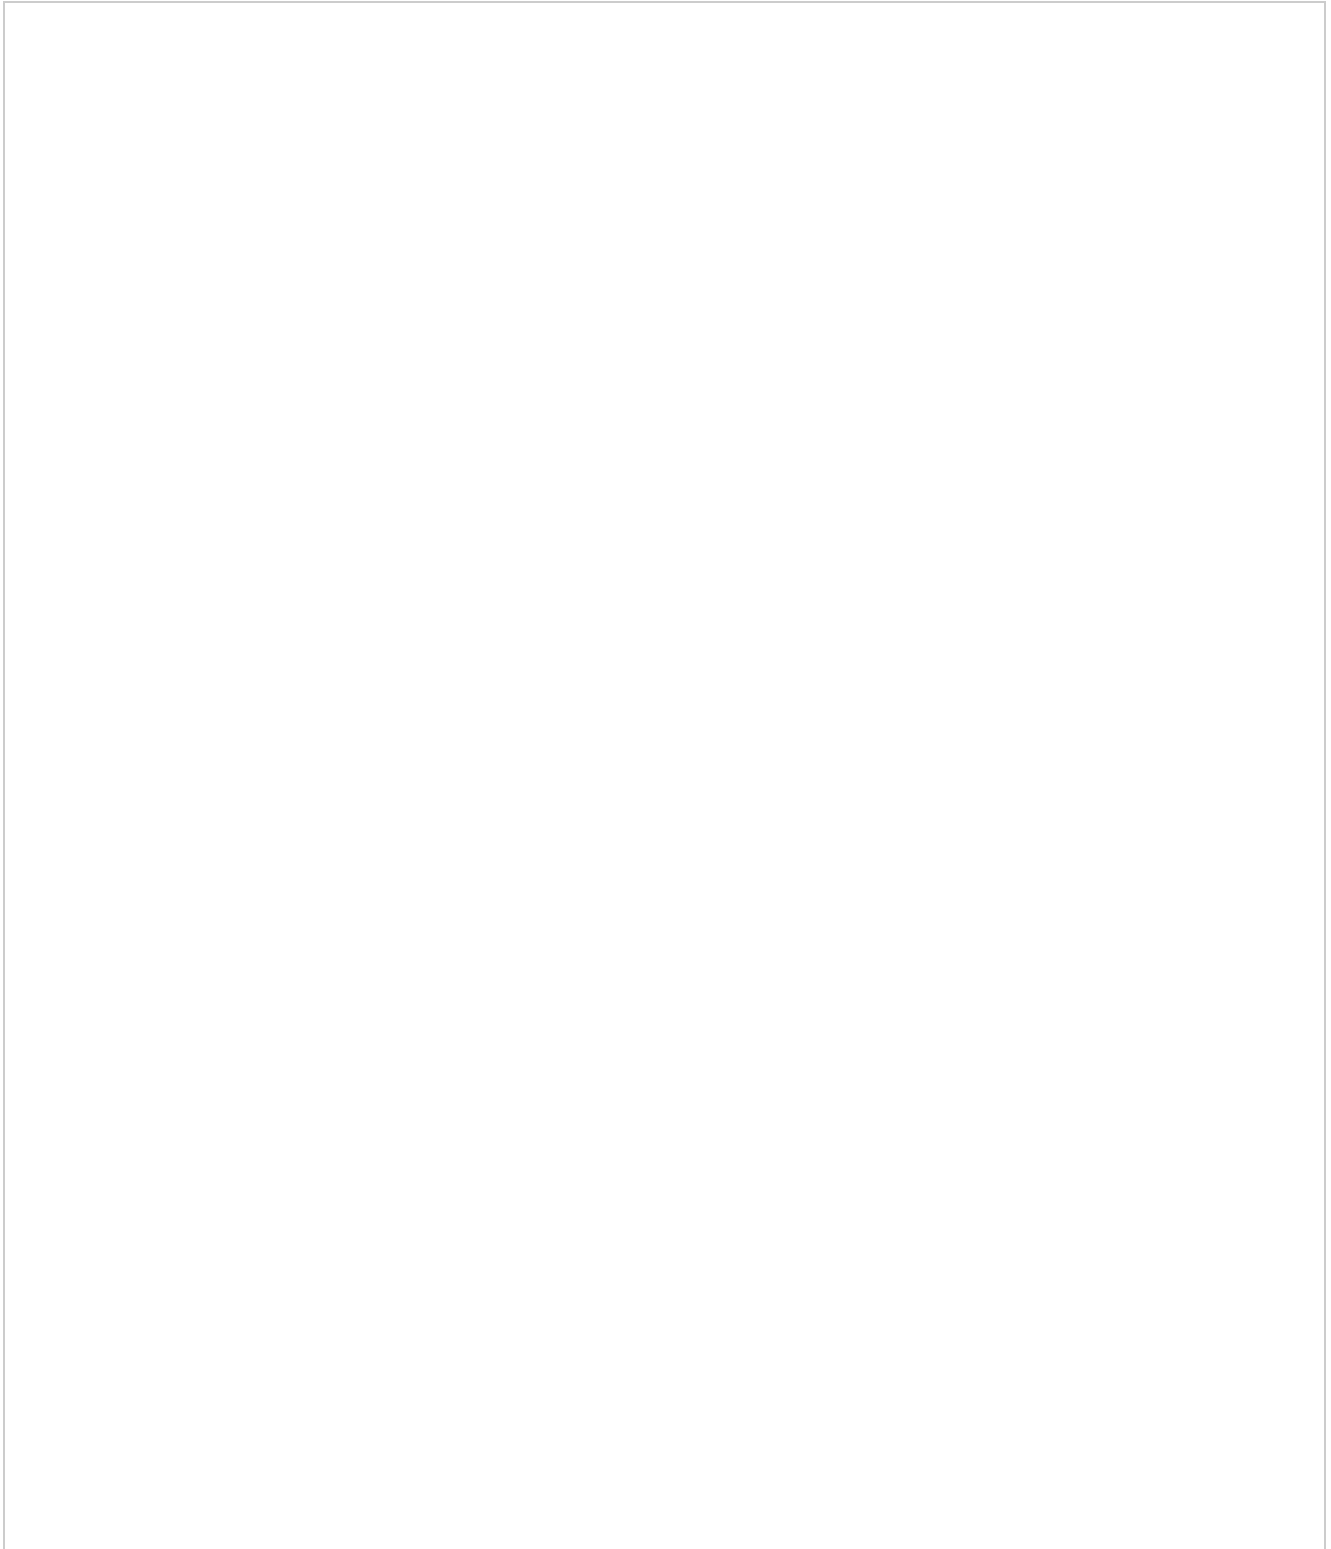

Please provide any of your comments on this color map.

A solid gray rectangular box, intended for providing comments on the color map.

143. How many percentages do the highlighted area match with your clinical judgment on the important features to classify LGG/HGG?

0%, Not matches at all                      50%                      Completely matches with mine, 100%

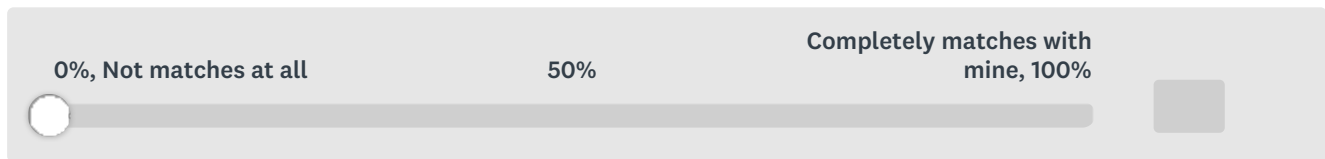☐

144. How helpful is this color map in clinical settings?

0, Not helpful at all                      5, Somewhat helpful                      Extremely helpful, 10

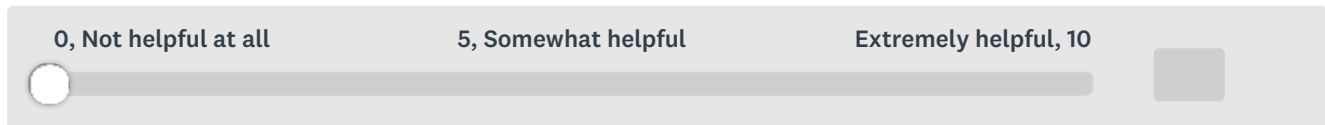☐

145. Did you notice the color map differences on different MRI modalities? How helpful is this feature in clinical settings?

0, Not helpful at all                      5, Somewhat helpful                      Extremely helpful, 10

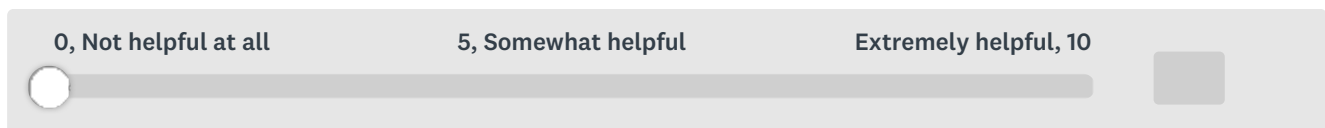☐

146. Suppose you have just reviewed the AI prediction and the **best** color map explanation, what is your trust level in this AI?

-5, Totally distrust the AI                      0, Neutral, neither distrust nor trust                      Totally trust the AI, 5

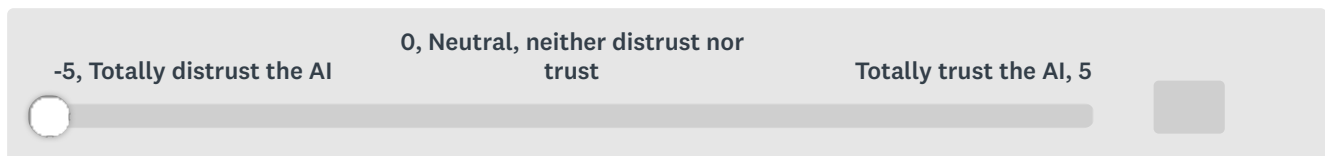☐

147. Suppose you have just reviewed the AI prediction and the **best** color map explanation, how likely will you incorporate this AI's suggestions into your clinical practice?

Consider the likelihood that you are willing to let this AI assist you (in ways such as: it may reinforce your confidence about a decision; or it may alert you to potential mistakes, etc.), and consider its suggestions to your patient's management plan.

0, Not likely                      5, Somewhat likely                      Very likely, 10

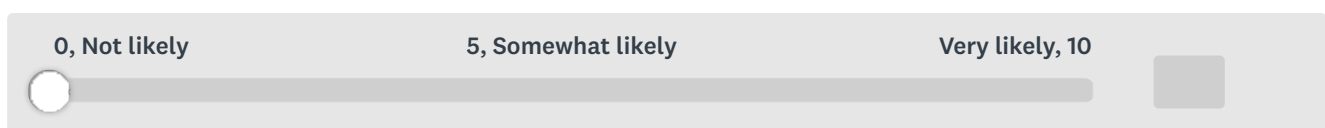☐

148. Suppose we have one of the best color maps embedded in the AI system, will and when are you most likely to check those color maps?

- ☐ To build and calibrate my trust in this AI
- ☐ To ensure the safety use of the AI
- ☐ To meet the ethical requirements
- ☐ To meet the legal requirements
- ☐ When I doubt about the prediction from AI
- ☐ For a difficult case, when I am not certain
- ☐ To ensure fairness and no biases in the AI model
- ☐ To generate report or patient chart
- ☐ To make Differential Diagnosis
- ☐ Before discussion with my colleagues
- ☐ To learn from AI
- ☐ To make new medical discovery
- ☐ To improve my patients' outcomes
- ☐ When I am trading off among multiple objectives for my patient
- ☐ Other (please specify)

## Welcome to the Medical AI study

149. For your selected scenarios to check the explanation from AI, would you mind ranking them regarding your likelihood of checking the explanations?

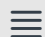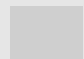

To build and calibrate my trust in this AI

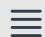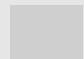

To ensure the safety use of the AI

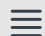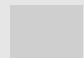

To meet the ethical requirements

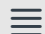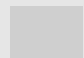

To meet the legal requirements

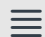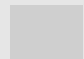

When I doubt about the prediction from AI

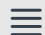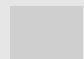

For a difficult case, when I am not certain

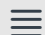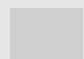

To ensure fairness and no biases in the AI model

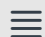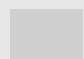

To generate report or patient chart

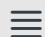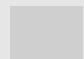

To make Differential Diagnosis

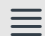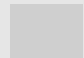

Before discussion with my colleagues

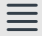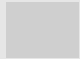

To learn from AI

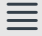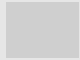

To make new medical discovery

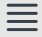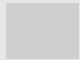

To improve my patients' outcomes

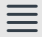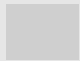

When I am trading off among multiple objectives for my patient

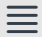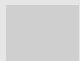

[Insert text from Other]
